# Supplementary material for: Designs from Local Random Quantum Circuits with SU(d) Symmetry
Source: arXiv:2309.08155 source file (2024-12-30)
Supplement: Supplementary file 1 [file CQA_SM1.pdf]

# Supplemental Material: Designs from local random quantum circuits with $SU(d)$ symmetry

Zimu Li<sup>\*</sup>,<sup>1,\*</sup> Han Zheng<sup>\*,2,3,†</sup> Junyu Liu,<sup>2,3,4,5,6,‡</sup> Liang Jiang,<sup>2,§</sup> and Zi-Wen Liu<sup>1,7,¶</sup>

<sup>1</sup>*Yau Mathematical Sciences Center, Tsinghua University, Beijing 100084, China*

<sup>2</sup>*Pritzker School of Molecular Engineering, The University of Chicago, Chicago, IL 60637, USA*

<sup>3</sup>*Department of Computer Science, The University of Chicago, Chicago, IL 60637, USA*

<sup>4</sup>*Kadanoff Center for Theoretical Physics, The University of Chicago, Chicago, IL 60637, USA*

<sup>5</sup>*qBraid Co., Chicago, IL 60637, USA*

<sup>6</sup>*SeQure, Chicago, IL 60637, USA*

<sup>7</sup>*Perimeter Institute for Theoretical Physics, Waterloo, Ontario N2L 2Y5, Canada*

In this Supplemental Material, we will provide more mathematical backgrounds and prove theorems given in the main text.

## CONTENTS

|                                                                                           |    |
|-------------------------------------------------------------------------------------------|----|
| I. Preliminaries                                                                          | 1  |
| A. Miscellaneous Facts on $S_n$ Representation Theory                                     | 2  |
| B. Schur-Weyl Duality and CQA Architecture                                                | 6  |
| II. Characterizing Random Circuit Designs by Commutant under Group Representation         | 8  |
| A. Quantum $k$ -fold Channel                                                              | 8  |
| B. Approximate $k$ -design and Random Walk on Group                                       | 9  |
| C. Frame Potential, Form factors, and $k$ -Invariance                                     | 11 |
| D. Commutant of the Group $U(\bigoplus_\lambda S^\lambda)$ of $SU(d)$ Symmetric Unitaries | 13 |
| III. Establishing Exact $k$ -design with $SU(d)$ Symmetry by CQA                          | 16 |
| A. Comparison of the $k$ -fold Channels $T_k^{SU}$ and $T_k^{\text{Haar}}$                | 16 |
| B. Comparison of the $k$ -fold Channels $T_k^{\text{CQA}}$ and $T_k^{\text{Haar}}$        | 18 |
| C. Circuit Locality for Universality and Unitary $k$ -design with $SU(d)$ Symmetry        | 21 |
| D. High Order CQA Group for Arbitrary Unitary Design with $SU(d)$ Symmetry                | 23 |
| IV. Approximating Unitary $k$ -design with $SU(d)$ Symmetry by CQA Ensembles              | 27 |
| A. CQA Ensemble and Its Variants                                                          | 27 |
| B. Several Attempts to Evaluate the Convergence Speed of $\mathcal{E}_{\text{CQA}}$       | 30 |
| C. Numerical Methods on Qudits                                                            | 35 |
| References                                                                                | 36 |

## I. PRELIMINARIES

We briefly introduce some basic notions and facts from  $S_n$  representation theory, as well as our CQA model, that may provide a comprehensive understanding on the later mathematical proofs. We also recommend the interested readers to [1–5] for more systematic presentations on these topics.

---

<sup>\*</sup> lizm@mail.sustech.edu.cn

<sup>†</sup> hanz98@uchicago.edu

<sup>‡</sup> junyuliu@uchicago.edu

<sup>§</sup> liangjiang@uchicago.edu

<sup>¶</sup> zwliu.permanent@gmail.com

A. Miscellaneous Facts on  $S_n$  Representation Theory

Irreducible representations (irreps) of the symmetric group  $S_n$  permuting  $n$  nodes are in one-to-one correspondence with the so-called *Young diagrams*, e.g., for  $S_6$  the following two Young diagrams stand for the *trivial* and the *fundamental* representation:

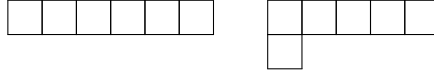

whose direct sum is more familiar as the 6-dimensional defining representation under which each  $\sigma \in S_6$  permutes the components of vectors from  $\mathbb{R}^6$ .

**Definition I.1.** Formally, let  $\lambda = (\lambda_1, \dots, \lambda_r)$  be a collection of positive integers such that  $\lambda_i \geq \lambda_{i+1}$  and  $\sum_i \lambda_i = n$ . Then  $\lambda$  is called a *partition of the integer  $n$* , denoted by  $\lambda \vdash n$ . Obviously,  $\lambda$  defines a Young diagram abstractly and the  $S_n$  irrep corresponding to this Young diagram is always denoted as  $S^\lambda$ . The dimension of this irrep is given by the *hook length formula*:

$$\dim S^\lambda = \frac{n!}{\prod_{(x,y) \in \lambda} h_{x,y}}, \quad (1)$$

where  $(x, y)$  specifies a box from  $\lambda$  by its *row* and *column numbers* and  $h(x, y)$  counts the number of all boxes on the right hand side and below  $(x, y)$ , including itself.

Given an arbitrary  $S_n$  irrep  $S^\lambda$ , there is a canonical way to label a basis, called *Gelfand-Tsetlin basis (GZ)* or *Young-Yamanouchi basis*, on the representation space using *standard Young tableau  $T$* , which are defined by filling into each box of  $\lambda$  a positive integer from  $1, 2, \dots, n$  in an increasing order from left to right and top to bottom. For instance, the fundamental representation of  $S_6$  mentioned above is 5-dimensional with 5 basis vectors being labeled as

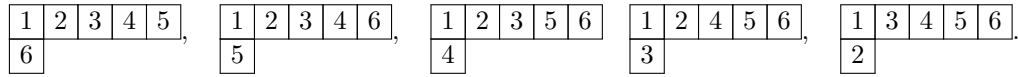

When we study the group commutant of  $SU(d)$  symmetric unitaries in the main text, Young basis  $\{|\alpha_T\rangle\}$  labeled by standard tableaux are implicitly used and a detailed treatment can be found in Section II D.

**Definition I.2.** For  $1 < k \leq n$ , the *Young-Jucys-Murphy element*, or YJM-element for short, is defined as a (formal) sum of *transpositions* or SWAPs

$$X_i = (1, i) + (2, i) + \dots + (i-1, i) \quad (2)$$

We set  $X_1 = 0$  as a convention.

YJM-element is the central concept used in our work developed by Young [6], Jucys [7] and Murphy [8] and later used by Okounkov and Vershik [9]. Under any  $S_n$  representation, it may be more comprehensible to treat  $X_i = (1, i) + (2, i) + \dots + (i-1, i)$  as the sum of matrix representations of these transpositions, or we can say that the representation is extended to the *group algebra*

$$\mathbb{C}[S_n] = \left\{ \sum_i c_i \sigma_i; \sigma_i \in S_n \right\} \quad (3)$$

consisting of formal finite linear combinations  $S_n$  group elements. By Wedderburn Theorem [2, 3],  $\mathbb{C}[S_n]$  is isomorphic with the direct sum of all inequivalent  $S_n$  irreps  $\bigoplus_\lambda S^\lambda$ . By Schur-Weyl duality, the  $\mathbb{C}[S_n]$  embraces all  $SU(d)$ -symmetric local Hamiltonian which is used to argue a quantum speedup in [5]. It also provides a perspective to discuss  $k$ -design through Lie group and Lie algebra in Section III.

Let us consider coordinate differences  $x - y$  of boxes from a Young diagram  $\lambda$ . Given any standard tableaux  $T$  of  $\lambda$ , its *content vector* is defined by rearranging them with respect to the order of boxes determined by the tableau. For example, content vectors of the above five standard tableaux are listed as follows:

$$(0, 1, 2, 3, 4, -1), \quad (0, 1, 2, 3, -1, 4), \quad (0, 1, 2, -1, 3, 4), \quad (0, 1, -1, 2, 3, 4), \quad (0, -1, 1, 2, 3, 4).$$

One significant feature of YJM-elements is their special actions under Young basis revealed by content vectors:

1. They are diagonal matrices under Young basis (even each single transposition  $(i, j)$  from Eq.(2) may not be diagonal).

2. The diagonal entries of  $X_i$  under the Young basis vector  $|\alpha_T\rangle$  corresponding to standard tableau  $T$  is just the  $i$ th component of the content vector.

On the irrep  $S^{(5,1)}$ ,

$$\begin{aligned} X_1 &= \begin{pmatrix} 0 & 0 & 0 & 0 & 0 \\ 0 & 0 & 0 & 0 & 0 \\ 0 & 0 & 0 & 0 & 0 \\ 0 & 0 & 0 & 0 & 0 \\ 0 & 0 & 0 & 0 & 0 \end{pmatrix}, & X_2 &= \begin{pmatrix} 1 & 0 & 0 & 0 & 0 \\ 0 & 1 & 0 & 0 & 0 \\ 0 & 0 & 1 & 0 & 0 \\ 0 & 0 & 0 & 1 & 0 \\ 0 & 0 & 0 & 0 & -1 \end{pmatrix}, & X_3 &= \begin{pmatrix} 2 & 0 & 0 & 0 & 0 \\ 0 & 2 & 0 & 0 & 0 \\ 0 & 0 & 2 & 0 & 0 \\ 0 & 0 & 0 & -1 & 0 \\ 0 & 0 & 0 & 0 & 1 \end{pmatrix}, \\ X_4 &= \begin{pmatrix} 3 & 0 & 0 & 0 & 0 \\ 0 & 3 & 0 & 0 & 0 \\ 0 & 0 & -1 & 0 & 0 \\ 0 & 0 & 0 & 2 & 0 \\ 0 & 0 & 0 & 0 & 2 \end{pmatrix}, & X_5 &= \begin{pmatrix} 4 & 0 & 0 & 0 & 0 \\ 0 & -1 & 0 & 0 & 0 \\ 0 & 0 & 3 & 0 & 0 \\ 0 & 0 & 0 & 3 & 0 \\ 0 & 0 & 0 & 0 & 3 \end{pmatrix}, & X_6 &= \begin{pmatrix} -1 & 0 & 0 & 0 & 0 \\ 0 & 4 & 0 & 0 & 0 \\ 0 & 0 & 4 & 0 & 0 \\ 0 & 0 & 0 & 4 & 0 \\ 0 & 0 & 0 & 0 & 4 \end{pmatrix} \end{aligned} \quad (4)$$

In summary, *Young basis vectors*  $|\alpha_T\rangle$ , *standard tableaux*  $T$  and *content vectors*  $\alpha_T$  are in one-to-one correspondence and uniquely determine the matrix representations of YJM-elements. We will introduce and apply other remarkable properties of YJM-elements in Section III D and IV B when derive our own results.

As mentioned when introducing our numerical method in the main text, Matrix representation of each *adjacent transposition*  $(i, i+1)$  can be explicitly read off under Young basis by *Young orthogonal form*: let  $r = \alpha_T(i+1) - \alpha_T(i)$  be the *axial distance* and let  $(i, i+1) \cdot T$  denote the tableau defined by exchanging integers  $i, i+1$  from  $T$ . It is easy to check that as long as  $r \neq \pm 1$ ,  $(i, i+1) \cdot T$  is still a standard Young tableau. Then

$$(i, i+1) |\alpha_T\rangle = \frac{1}{r} |\alpha_T\rangle + \sqrt{1 - \frac{1}{r^2}} |\alpha_{(i,i+1) \cdot T}\rangle, \quad (i, i+1) |\alpha_{(i,i+1) \cdot T}\rangle = \sqrt{1 - \frac{1}{r^2}} |\alpha_T\rangle - \frac{1}{r} |\alpha_{(i,i+1) \cdot T}\rangle. \quad (5)$$

On the irrep  $S^{(5,1)}$ ,

$$\begin{aligned} (1, 2) &= \begin{pmatrix} 1 & 0 & 0 & 0 & 0 \\ 0 & 1 & 0 & 0 & 0 \\ 0 & 0 & 1 & 0 & 0 \\ 0 & 0 & 0 & 1 & 0 \\ 0 & 0 & 0 & 0 & -1 \end{pmatrix}, & (2, 3) &= \begin{pmatrix} 1 & 0 & 0 & 0 & 0 \\ 0 & 1 & 0 & 0 & 0 \\ 0 & 0 & 1 & 0 & 0 \\ 0 & 0 & 0 & -\frac{1}{2} & \frac{\sqrt{3}}{2} \\ 0 & 0 & 0 & \frac{\sqrt{3}}{2} & \frac{1}{2} \end{pmatrix}, & (3, 4) &= \begin{pmatrix} 1 & 0 & 0 & 0 & 0 \\ 0 & 1 & 0 & 0 & 0 \\ 0 & 0 & -\frac{1}{3} & \frac{2\sqrt{2}}{3} & 0 \\ 0 & 0 & \frac{2\sqrt{2}}{3} & \frac{1}{3} & 0 \\ 0 & 0 & 0 & 0 & 1 \end{pmatrix}, \\ (4, 5) &= \begin{pmatrix} 1 & 0 & 0 & 0 & 0 \\ 0 & -\frac{1}{4} & \frac{\sqrt{15}}{4} & 0 & 0 \\ 0 & \frac{\sqrt{15}}{4} & \frac{1}{4} & 0 & 0 \\ 0 & 0 & 0 & 1 & 0 \\ 0 & 0 & 0 & 0 & 1 \end{pmatrix}, & (5, 6) &= \begin{pmatrix} -\frac{1}{5} & \frac{2\sqrt{6}}{5} & 0 & 0 & 0 \\ \frac{2\sqrt{6}}{5} & \frac{1}{5} & 0 & 0 & 0 \\ 0 & 0 & 1 & 0 & 0 \\ 0 & 0 & 0 & 1 & 0 \\ 0 & 0 & 0 & 0 & 1 \end{pmatrix}. \end{aligned} \quad (6)$$

Having access to the matrix representations of all adjacent transpositions allows us to calculate that for any permutation  $\sigma \in S_n$  in principal and there are classical or quantum  $S_n$ -Fast Fourier Transform designed for this task [10, 11] A detailed illustration of using Young orthogonal form in our numerical computation is in Section IV B.

**Definition I.3.** Given an arbitrarily partition/Young diagram  $\lambda \vdash n$ . A permutation  $\sigma \in S_n$  is of *cycle type*  $\lambda$  if it is decomposed into cycles of lengths  $\lambda_1, \dots, \lambda_r$ .

For instance,  $\sigma = (134)(56) \in S_6$  is of the type  $\lambda = (3, 2, 1)$ . The trivial permutation  $\text{id} \in S_n$  is of type  $(1, \dots, 1)$ . Transpositions or SWAPs  $(i, j)$  are just 2-cycles. Products of transpositions like  $(i, j)(k, l) \cdots (s, t)$  are of the type  $(2, 2, \dots, 2, 1, \dots, 1)$ .

**Definition I.4.** Let  $p(n)$  denotes the *number of partitions of  $n$* . Then it equals the number of all inequivalent  $S_n$  irreps, as well as the number of possible cycle types in  $S_n$ . Analogously, we define  $p(n, d)$  as the *number of partitions of  $n$  with at most  $d$  parts*, i.e., the number of all Young diagrams of  $n$  boxes with at most  $d$  rows.

We encounter  $p(n)$  and  $p(n, d)$  in the main text when arguing the difficulty of computing frame potential with the presence of  $SU(d)$  symmetry. They also appear when we study the locality required to achieve arbitrary  $k$ -design (Section II D and III C in this supplementary material). It is due to the celebrated work of Ramanujan and Hardy [12] and Uspensky [13] that

$$p(n) \sim \frac{e^{\sqrt{\pi^2 2n/3}}}{4n\sqrt{3}}, n \rightarrow \infty \quad (7)$$

with further researches [14, 15] and useful bounds on  $p(n)$  being found later such as [16, 17]

$$\frac{e^{2\sqrt{n}}}{an} < p(n) < e^{b\sqrt{n}}. \quad (8)$$

If  $d = 2$ ,  $p(n, 2) = \lfloor \frac{n}{2} \rfloor + 1$ . However, there is no closed formulas for these partition functions in general.

**Proposition I.5.** Let  $c_\mu \in \mathbb{C}[S]$  be the sum of all  $\sigma \in S_n$  with cycle type  $\mu$ . Consider all possible Young diagrams of size  $n$ , the collection  $\{c_\mu\}_{\mu \vdash n}$  forms a basis for the center  $Z(\mathbb{C}[S_n])$  consisting of all elements that commute with  $\mathbb{C}[S_n]$ .

It is by definition that  $c_\mu$  commutes with any  $\sigma \in S_n$ . By Wedderburn theorem [2, 3], its matrix representation, still denoted by  $c_\mu$  for simplicity, under any  $S_n$  irrep  $S^\lambda$  is just a scalar. As a result, the representation of  $Z(\mathbb{C}[S_n])$  consists of scalars matrices within any  $S_n$  irrep. Being a basis of  $Z(\mathbb{C}[S_n])$  means being a basis capable of spanning all scalars matrices, called *relative phase factors* when we study  $k$ -design with symmetry, respecting the direct sum  $\bigoplus S^\lambda$  of all inequivalent  $S_n$  irreps. In Section III C and III D, the diagonal phase matrix  $e^{-ic_\mu}$  helps to replenish relative phase factors for the group of  $SU(d)$  symmetric unitaries.

Besides the basis  $\{c_\mu\}$  defined above, we still have the following two kinds of center bases:

**Theorem I.6.** The following two collections also constitute bases for  $Z(\mathbb{C}[S_n])$ :

1. Let us consider the  $S_n$  group character

$$\chi_\lambda(\sigma) = \text{tr}_\lambda \sigma \quad (9)$$

defined by taking the trace of  $\sigma \in S_n$  restricted to the irrep  $S^\lambda$ , then

$$\Pi_\mu := \frac{\dim S^\mu}{n!} \sum_{\sigma \in S_n} \bar{\chi}_\mu(\sigma) \sigma = \begin{cases} I, & \mu = \lambda \\ 0, & \text{otherwise} \end{cases}. \quad (10)$$

The collection  $\{\Pi_\mu\}$  is an orthonormal basis.

2. Let us consider the YJM-elements  $X_i$ . For any  $\mu = (\mu_1, \dots, \mu_r) \vdash n$ , we set

$$X_\mu = \sum_{2 \leq i_1 \neq i_2 \neq \dots \neq i_r \leq n} X_{i_1}^{\mu_1-1} X_{i_2}^{\mu_2-1} \dots X_{i_r}^{\mu_r-1} \quad (11)$$

The collection  $\{X_\mu\}$  is also a basis for  $Z(\mathbb{C}[S_n])$  [4, 7, 8].

For the purpose of efficient implementation into quantum circuits, we would always construct center basis elements through  $X_\mu$  because encoding  $c_\mu$  requires to sum over all permutations of a given cycle type  $\mu$  and encoding  $\Pi_\mu$  even needs doing that over the whole symmetric group with  $n!$  elements. However, it should be noted that for either cases, building a complete basis finally employs non-local operator acting on all qudits and we will come back to discuss the problem of locality in Section III C and III D.

In Section III B, we also need to compute the character  $\chi_\lambda(\sigma)$  explicitly for some  $\sigma \in S_n$ , so we briefly introduce the method here. We first present the following proposition which is crucial to the proofs in Section III C:

**Proposition I.7.** For any  $\sigma \in S_n$ ,  $\chi_\lambda(\sigma) \in \mathbb{Z}$ . That is,  $S_n$  characters are integer-valued.

One can prove a bunch of similar facts by Galois Theory for general finite groups. In our case, we simply note that there is the so-called *Young's natural representation* which is a *non-unitary* representation of  $S^\lambda$  under which each  $\sigma$  is expressed as matrices with integer entries [2]. As trace is invariant under matrix similarity,  $\chi_\lambda(\sigma) = \text{tr}_\lambda \sigma \in \mathbb{Z}$  in general.

It is also well known that permutations  $\sigma, \sigma'$  with the same cycle type are conjugate to each other, so  $\chi_\lambda(\sigma) = \chi_\lambda(\sigma')$  and thus we only concern the value of  $\chi_\lambda$  for a given cycle type  $\mu$ . The so-called *Frobenius character formula* [3] expresses  $S_n$  character values as coefficients of a power series. The coefficient can be computed by, for instance, contour integrals with residue theorem in principal. However, closed formulas are only seen for very few simple cases [18, 19]. For instance, characters for 2-cycles (transpositions/SWAPs) equals

$$\frac{\chi_\lambda(i, j)}{\dim S^\lambda} = \frac{2}{n(n-1)} \sum_i \left( \binom{\lambda_i}{2} - \binom{\lambda'_i}{2} \right) = \frac{1}{n(n-1)} \sum_i [(\lambda_i - 1)(\lambda_i - 1 + i) - i(i - 1)], \quad (12)$$

where  $\lambda'$  denotes the conjugate of  $\lambda$ , e.g.,

$$\lambda = \begin{array}{|c|c|c|c|} \hline & & & \\ \hline & & & \\ \hline & & & \\ \hline & & & \\ \hline \end{array} \quad \lambda' = \begin{array}{|c|c|c|} \hline & & \\ \hline & & \\ \hline & & \\ \hline & & \\ \hline \end{array}$$

If  $\lambda_i < 2$ , the corresponding binomial coefficient is set to zero.

Let us relate the above character formula to some techniques involving YJM-elements. Restricted to any irrep  $S^\lambda$ , we can associate the following invariants:

$$P_l = \left( \sum_i X_i \right)^l, l = 1, 2, \dots \quad (13)$$

where  $\sum_i X_i$  is the summation of all YJM-elements. Let us check its matrix form under Young basis  $|\alpha_T\rangle$ :

$$\left( \sum_i X_i \right) |\alpha_T\rangle = \sum_i \alpha_T(i) |\alpha_T\rangle \quad (14)$$

with  $\alpha_T$  being the content vector. Obviously, for any fixed Young diagram  $\lambda$ , the sum of all components of any of its content vector  $\alpha_T$  is simply equal to the sum of all coordinate differences, and we denote it as  $\alpha_\lambda$ . Then

$$P_l |\alpha_T\rangle = (\alpha_\lambda)^l |\alpha_T\rangle \quad (15)$$

for all standard tableaux/Young basis vectors of the Young diagram  $\lambda$ .

Let  $\text{tr}_\lambda$  denote by taking trace within  $S^\lambda$  (it is actually just the  $S_n$  character in Eq.(9)). When  $l = 1$ , we note that

$$\alpha_\lambda = \frac{\text{tr}_\lambda(P_1)}{\dim S^\lambda} = \frac{\text{tr}_\lambda \sum_i X_i}{\dim S^\lambda} = \frac{n(n-1)}{2} \frac{\text{tr}_\lambda(i, j)}{\dim S^\lambda} = \frac{n(n-1)}{2} \frac{\chi_\lambda(i, j)}{\dim S^\lambda} \quad (16)$$

which gives another way to compute the character value of 2-cycles by summing all components from the content vector. The method using YJM-elements and content vectors to express general  $S_n$  characters can be found in [20].

**Definition I.8.** Given two partitions  $\lambda = (\lambda_i), \mu = (\mu_i) \vdash n$ . We say that  $\lambda$  dominates  $\mu$ , denoted by  $\lambda \triangleright \mu$ , if for all  $j > 0$ ,  $\sum_i^j \lambda_i \geq \sum_i^j \mu_i$ .

For instance, we have

$$(6) \triangleright (5, 1) \triangleright (4, 2) \triangleright (4, 1^2) \quad (17)$$

where  $(4, 1^2)$  is the abbreviation of  $(4, 1, 1)$ . The dominance relation is not *totally ordered*, e.g., we cannot compare  $(4, 1^2)$  and  $(3, 3)$ . However, in the case of qubits ( $d = 2$ ), where we focus on two-row Young diagrams by Schur-Weyl duality introduced in the following, partitions  $\lambda = (\lambda_1, \lambda_2)$  with  $\lambda_1 \geq \lambda_2$  clearly give rise to a total ordering.

**Lemma I.9.** For any two partitions unequal  $\lambda, \mu \vdash n$ , if  $\lambda \triangleright \mu$ , then  $\alpha_\lambda > \alpha_\mu$ .

*Proof.* We prove the lemma by induction. Suppose the statement holds for  $n - 1$ . Given unequal  $\lambda, \mu \vdash n$  with  $\lambda \triangleright \mu$ , there should be some  $i$  such that  $\lambda_i > \mu_i$  as the lengths of  $i$ th rows of  $\lambda$  and  $\mu$  respectively. If  $\lambda_i > \lambda_{i+1}$  and  $\mu_i > \mu_{i+1}$ , then we discard the RHS boxes on the  $i$ th rows of  $\lambda$  and  $\mu$ . The resultant Young diagrams, denoted by  $\lambda'$  and  $\mu'$  still satisfy the relation  $\lambda' \triangleright \mu'$ . Then by induction hypothesis,  $\alpha_{\lambda'} > \alpha_{\mu'}$ . On the other hand, the content of the discarded box from  $\lambda$  is larger than that from  $\mu$  by definition, hence we conclude that  $\alpha_\lambda > \alpha_\mu$ .

Suppose  $\lambda_i = \lambda_{i+1} = \dots = \lambda_r$  or  $\mu_i = \mu_{i+1} = \dots = \mu_s$ . Then we are only allowed to discard the RHS boxes of  $\lambda_r, \mu_s$  to ensure that  $\lambda'$  and  $\mu'$  are well-defined Young diagrams. Even when  $r \neq s$ , the dominance relation still holds because  $\lambda_r > \mu_s$ . By the same argument as above, we complete the proof.  $\square$

By Eq.(16), the above lemma says that  $\frac{\chi_\lambda(1,2)}{\dim S^\lambda}$  is strictly increasing with respect to the dominance order of  $\lambda$ . Lots of counterexamples occurs when this order fails to hold: e.g.,  $(3, 3)$  and  $(4, 1^2)$ .

Let us end this subsection with some explicit analysis on the dimension of  $S_n$  irreps of two-row Young diagram. In this circumstance, the hook length formula in I.1 can be further simplified as [2, 18]:

$$\dim S^\lambda = d_\lambda = \binom{n}{r} - \binom{n}{r-1} = \frac{n-2r+1}{n-r+1} \binom{n}{r}. \quad (18)$$

For binomial coefficient, we have another two useful bounds (assume  $n = 2m$ ) [21]:

$$\frac{2^n}{\sqrt{\pi(\frac{n}{2} + \frac{1}{3})}} \leq \binom{n}{n/2} \leq \frac{2^n}{\sqrt{\pi(\frac{n}{2} + \frac{1}{4})}}, \quad e^{-(\frac{n}{2}-r)^2/(n-r+1)} \leq \binom{n}{r} / \binom{n}{\frac{n}{2}} \leq e^{-(\frac{n}{2}-r)^2/(n-r)}. \quad (19)$$

Therefore, the ratio of  $\dim S^\lambda$  to the dimension of the entire Hilbert space is

$$\frac{1}{\sqrt{\pi(\frac{n}{2} + \frac{1}{3})}} \frac{n-2r+1}{n-r+1} \binom{n}{r} / \binom{n}{\frac{n}{2}} \leq \frac{\dim S^\lambda}{2^n} = \frac{1}{2^n} \frac{n-2r+1}{n-r+1} \binom{n}{r} \leq \frac{1}{\sqrt{\pi(\frac{n}{2} + \frac{1}{4})}} \frac{n-2r+1}{n-r+1} \binom{n}{r} / \binom{n}{\frac{n}{2}}. \quad (20)$$

A lower bound for general  $d$ -row Young diagram is also useful [22, 23]: suppose the first row  $\lambda_1, \lambda'_1$  of  $\lambda$  and its conjugate is upper bounded by  $\frac{n}{\alpha}$  for some  $\alpha > 1$ . Then

$$\dim S^\lambda \geq \frac{\alpha^n}{n^{d(d+2)/2}}. \quad (21)$$

We will use these results for specific cases in Section III B.

### B. Schur-Weyl Duality and CQA Architecture

We now make a brief review on  $S_n$ -Convolutional Quantum Alternating Ansätze and the group CQA proposed in [5] which is proved to form the exact  $k$ -design with  $SU(d)$  symmetry and motivates the definition of CQA ensemble in approximating unitary  $k$ -design.

In quantum systems there is a discrete set of translations corresponding to permuting the qudits as well as a continuous notion of translation corresponding to spatial rotations by elements of  $SU(d)$ . To be precise, let  $V$  be a  $d$ -dimensional complex Hilbert space with orthonormal basis  $\{e_1, \dots, e_d\}$ . The tensor product space  $V^{\otimes n}$  admits two natural representations: the *tensor product representation*  $\pi_{SU(d)}$  of  $SU(d)$  acting as

$$\pi_{SU(d)}(g)(e_{i_1} \otimes \dots \otimes e_{i_n}) := g \cdot e_{i_1} \otimes \dots \otimes g \cdot e_{i_n}, \quad (22)$$

where  $g \cdot e_{i_k}$  is the fundamental representation of  $SU(d)$ , and the *permutation representation*  $\pi_{S_n}$  of  $S_n$  acting as

$$\pi_{S_n}(\sigma)(e_{i_1} \otimes \dots \otimes e_{i_n}) := e_{i_{\sigma^{-1}(1)}} \otimes \dots \otimes e_{i_{\sigma^{-1}(n)}}. \quad (23)$$

We treat  $H = V^{\otimes n}$  as the Hilbert space of an  $n$ -qudit system. The so-called Schur-Weyl duality says that the action of  $SU(d)$  and  $S_n$  on  $V^{\otimes n}$  jointly decompose the space into irreducible representations of both groups in the form

$$V^{\otimes n} = \bigoplus_{\lambda} W_{\lambda} \otimes S^{\lambda}. \quad (24)$$

Recall that  $\lambda$  denotes a Young diagram. It corresponds not only to a unique  $S_n$  irrep  $S^{\lambda}$ , but also an  $SU(d)$  irrep  $W_{\lambda}$  in this setting [3, 4].

It should be noted that within an  $n$ -qudit system, only irreps corresponding to  $\lambda$  ranging over *Young diagrams of size  $n$  with at most  $d$  rows* can be found in the decomposition. Consequently,

$$\pi_{SU(d)} \cong \bigoplus_{\mu} W_{\mu} \otimes 1_{m_{SU(d), \mu}}, \quad \pi_{S_n} \cong \bigoplus_{\lambda} 1_{m_{S_n, \lambda}} \otimes S^{\lambda}, \quad (25)$$

where  $m_{SU(d), \mu} = \dim S^{\mu}$  and  $m_{S_n, \lambda} = \dim W_{\lambda}$ .

Given any operator  $A$  acting on the system, being  $SU(d)$  symmetric/invariant means

$$\pi_{SU(d)}(g)A = A\pi_{SU(d)}(g) \text{ or } g^{\otimes n}A = Ag^{\otimes n}. \quad (26)$$

One can check Eq.(22) and (23) that these permutation actions clearly commute with  $g^{\otimes n}$ . Furthermore Schur-Weyl duality, as well as double commutant theorem [3, 4], confirms that  $SU(d)$  symmetric operators are exactly built from permutations in the symmetric group  $S_n$ . That is, they can be written as linear combinations, like  $\sum c_i \sigma_i$ , of permutations.

Even decomposing the entire space into  $SU(d)$  irreps is quite conventional in physics. Quantum states living in these subspaces are actually permutation-invariant or  $S_n$  symmetric. Since our focuses are quantum circuits with  $SU(d)$  symmetry, we should decompose the entire Hilbert space with respect to  $S_n$  irreps (see [4, 5, 24] for more details). As a reminder, even the entire Hilbert space is decomposed into smaller subspaces, there is no reason to expect that related problems, like searching the ground state energy of  $SU(d)$  symmetric Hamiltonian or construing  $SU(d)$  symmetric random quantum circuit, would become easier. There are two reasons in general,

- (a) There are various inequivalent  $S_n$  irreps from the decomposition to deal with, and the total number is  $p(n, d)$ , which scales at most super-polynomially (Eq.(7)) with  $n$  and has no closed form to evaluate.
- (b) Even for qubits with  $d = 2$ , using the hook length formula from Definition I.1, we know that (cf.Eq.(18))

$$\dim S^{(m,m)} = \frac{(2m)!}{(m+1)!m!} = \frac{2^m}{m+1} \prod_{k=1}^m \frac{2k-1}{k} > \frac{2^m}{m+1} \quad (27)$$

for the  $S_n$  irrep of Young diagram  $\lambda = (m, m)$  on a  $2m$ -qubit system. One can find other examples with exponential large subspaces respecting the  $SU(d)$  symmetry [23], which still cause difficulties when approaching the problem.

We now introduce the mathematical definition of  $S_n$ -CQA ansatz:

**Definition I.10.** The  $S_n$ -CQA ansatz is defined as

$$\cdots \exp(-i \sum_{k,l} \beta_{kl} X_k X_l) \exp(-i\gamma H_S) \exp(-i \sum_{k,l} \beta'_{kl} X_k X_l) \exp(-i\gamma' H_S) \cdots, \quad (28)$$

where  $X_k X_l$  are product of YJM-elements, which is 4-local and still diagonal under Young basis (see Example.(4)). The Hamiltonian  $H_S$  is defined as the summation of adjacent transpositions  $\sum_{i=1}^{n-1} (i, i+1)$ .

Moreover, let us define the group generated by alternating exponentials from Eq.(28)

$$\text{CQA} = \left\langle \exp(-i \sum_{k,l} \beta_{kl} X_k X_l), \quad \exp(-i\gamma H_S) \right\rangle. \quad (29)$$

Obviously, CQA is contained in the group of  $SU(d)$  symmetric unitaries. To define this group, let  $U(S^\lambda)$  denote the unitary group acting on the representation space  $S^\lambda$ , i.e.,  $U(S^\lambda) \cong U(\dim S^\lambda)$ . A typical element  $g$  from the group of  $SU(d)$  symmetric unitaries is then a collection of unitaries:

$$g = \bigoplus_{\lambda} U_{\lambda}^{\oplus m_{S_n, \lambda}}, \quad (30)$$

where  $U_{\lambda} \in U(S^\lambda)$  and  $\lambda$  ranges over all Young diagrams of size  $n$  with at most  $d$  rows. For simplicity, we omit the multiplicities and denote this group by

$$\mathcal{H}_{\times} = U\left(\bigoplus_{\lambda} S^{\lambda}\right). \quad (31)$$

Equivalent copies of  $S_n$  irreps poses no more difficulties in computing  $k$ -fold channel/ $k$ th moment operator twirled through  $SU(d)$  symmetric unitaries in Section III A, but it is one of the obstacles when we calculate frame potential/dimension of the commutant of  $\mathcal{H}_{\times} = U(\bigoplus_{\lambda} S^{\lambda})$  in Section II C.

On the other hand, by restricting the phase factors to be 1 on each  $S^{\lambda}$ , we have the special unitary group  $SU(S^{\lambda})$  as well as  $S\mathcal{H}_{\times} = SU(\bigoplus_{\lambda} S^{\lambda})$  consisting of  $SU(d)$  symmetric unitaries with unit determinant on each  $S_n$  irrep block, i.e., unitaries with trivial relative phase factors with respect to. each irrep sector. It is proved in [5] that

$$S\mathcal{H}_{\times} \subsetneq \text{CQA} \subsetneq \mathcal{H}_{\times} \quad (32)$$

which establishes a theoretical guarantee in searching the ground state energy of  $SU(d)$  symmetric frustrated 2D Heisenberg model using  $S_n$ -CQA ansatz because relative phase factors can be ignored when we measure the expectation value in the experiment.

With the focus on locality, 2-local unitaries are proved to be universal to common quantum circuits [25], as well as approximate polynomial-designs [26, 27]. After imposing the  $SU(d)$  symmetry however, it is shown in [28–30] that when  $d \geq 3$ , 2-local  $SU(d)$  symmetric unitaries cannot even generate  $S\mathcal{H}_{\times}$ . The group CQA accomplishes this task by incorporating 4-local  $SU(d)$  symmetric unitaries, and we present in the following sections the mathematical details on using CQA to establish unitary  $k$ -design under  $SU(d)$  symmetry in both exact and approximate senses.



## II. CHARACTERIZING RANDOM CIRCUIT DESIGNS BY COMMUTANT UNDER GROUP REPRESENTATION

To study whether an ensemble forms a  $k$ -design in both exact and approximate sense, there are two deeply related two approaches: computing the frame potential of the ensemble, or analyzing the commutant algebra in the representation space. In this section, we illustrate these strategies in details, show their relationship mathematically (Proposition II.7) and finally move to determine the commutant of the group  $U(\bigoplus_\lambda S^\lambda)$  of  $SU(d)$  symmetric unitaries (Theorem II.8) and discuss the limitation of computing frame potential for Haar measure with the presence of  $SU(d)$  symmetry. These perspectives connect various approaches to understand unitary design such as using the tensor product expander [26, 27, 31, 32],  $k$ th moment operators channel [33, 34] or frame potential [35–40], from which we derive our results on  $SU(d)$  symmetric unitary design with in Section III and IV.

### A. Quantum $k$ -fold Channel

We first give definition of  $k$ -fold channel [34, 38] or  $k$ th-moment operator of a compact group  $G$ .

**Definition II.1.** Given a compact group  $G$  with the Haar measure  $\mu$  and a unitary representation  $\rho$  on the concerned Hilbert space  $H$ . For any operator  $M \in \text{End}(H^{\otimes k})$ , the  $k$ -fold channel twirled over  $G$  acting on  $M$  is:

$$T_k^G(M) = \int_G d\mu(g) \rho^{\otimes k}(g) M (\rho^{\otimes k}(g))^\dagger = \int_G dU U^{\otimes k} M U^{\dagger \otimes k}, \quad (33)$$

where we denote matrix representations of group elements simply by  $U, V$  on the RHS of the above identity. Despite its integral form, as a super-operator,  $T_k^G$  is merely a linear map acting on  $\text{End}(H^{\otimes k})$  and can be reformulated as the  $k$ th moment operator:

$$T_k^G = \int_G U^{\otimes k} \otimes \bar{U}^{\otimes k} dU. \quad (34)$$

Replacing  $G$  by an arbitrary ensemble  $\mathcal{E}$  with a precised measure  $\nu$ ,  $T_k^\mathcal{E}$  can be defined similarly when studying approximate  $k$ -design.

Since Haar measure is left-invariant,  $T_k(M)$  commutes with the  $k$ -fold tensor product representation  $\rho^{\otimes k}$  of  $G$ :

$$V^{\otimes k} T_k^G(M) V^{\dagger \otimes k} = \int_G (VU)^{\otimes k} M (UV)^{\dagger \otimes k} dU = T_k^G(M). \quad (35)$$

To put this identity in another way,  $T_k^G$  projects  $M$  into the *commutant algebra*:

$$\text{Comm}_k(G) := \{M \in \text{End}(H^{\otimes k}); U^{\otimes k} M = M U^{\otimes k}\}, \quad (36)$$

i.e., the subspace of all operators that commute with the tensor product representation  $\rho^{\otimes k}$ . The operator  $T_k^G$  is surjective since if  $M \in \text{Comm}(M)$ ,  $T_k^G(M) = M$  by definition. It is thus a *projector* from  $\text{End}(H^{\otimes k})$  onto  $\text{Comm}_k(G)$ . Then we have the following identity by either the invariance of Haar measure or the property of projector:

$$T_k^G(T_k^G(M)) = \int_G dU dV (VU)^{\otimes k} M (UV)^{\dagger \otimes k} = \int_G d(UV) (VU)^{\otimes k} M (UV)^{\dagger \otimes k} = T_k^G(M), \quad (37)$$

which further implies that  $T_k^G$  has eigenvalues either 0 or 1.

For the common case of unitary designs without any assumption on symmetries of the system,  $G = U(d^n) \equiv U(N)$  with  $\rho^{\otimes k}$  is given by the  $k$ -fold tensor products of fundamental representation of  $U(N)$ . Therefore, by the Schur-Weyl duality and double commutant theorem (cf. Schur-Weyl duality on an  $n$ -qudit system), the commutant algebra is isomorphic to the representation of the symmetric group algebra  $\mathbb{C}[S_k]$  which permutes elements from  $H^{\otimes k}$ . With the presence of  $SU(d)$  symmetry, the group of interests is replaced by  $U(\bigoplus_\lambda S^\lambda)$  defined in Section I B. We particularly denote by  $T_k^{\text{Haar}}$  the  $k$ -fold channel twirled over the group  $U(\bigoplus_\lambda S^\lambda)$  respecting symmetry.

To establish  $k$ -design with  $S_n$ -CQA, we will later analyze  $T_k^{\text{CQA}}$  and  $T_k^{\mathcal{E}_{\text{CQA}}}$  twirled over the group CQA and the ensemble  $\mathcal{E}_{\text{CQA}}$  and compare them with  $T_k^{\text{Haar}}$  in Section III B and Section IV B.



### B. Approximate $k$ -design and Random Walk on Group

The viewpoint that  $T_k^G$  is a projector to the commutant of  $G$  offers a convenient characterization for unitary  $k$ -design, with the usual definition [26, 34] (also see [31, 32, 38] for several alternative definitions and comparison on operator norms [41, 42]):

**Definition II.2.** For  $\epsilon > 0$ , an ensemble of unitaries  $\mathcal{E}$  is an  $\epsilon$ -approximate  $k$ -design if the diamond norm of the difference of  $k$ -fold channels satisfies

$$\|T_k^\mathcal{E} - T_k^G\|_\diamond \leq \epsilon. \quad (38)$$

**Lemma II.3.** Recall that  $T_k^\mathcal{E}$  is merely a linear map on  $\text{End}(H^{\otimes k})$ . With further conditions on the measure  $\nu$  of  $\mathcal{E}$  being specified,  $T_k^\mathcal{E}$  satisfies the following properties:

1. If  $\nu$  is left-invariant, then  $T_k^\mathcal{E}$  becomes a projector onto  $\text{Comm}_k(\mathcal{E})$ .
2. If  $\nu$  is invariant under inverse, i.e.,

$$\int_{\mathcal{E}} d\nu(g) f(g^{-1}) = \int_{\mathcal{E}} d\nu(g) f(g) \quad (39)$$

for any function  $f$  defined on  $\mathcal{E}$ , then  $T_k^\mathcal{E}$  is Hermitian.

Epecially when  $\mathcal{E}$  is taken as a certain compact subgroup of  $G$  with the restricted Haar measure, then both of the above properties hold.

We have seen the first property in Section II A. The second property is also straightforward by using  $U^{-1} = U^\dagger$  for unitary representation:

$$T_k^{\mathcal{E}\dagger} = \int_S V^{\dagger \otimes k} \bar{V}^{\dagger \otimes k} dV = \int_S (V^{-1})^{\otimes k} M (\bar{V}^{-1})^{\otimes k} dV = T_k^\mathcal{E}. \quad (40)$$

Most ensembles encountered in literature like [26, 27, 34], as well as our CQA ensemble defined in Section IV A, produces Hermitian  $k$ -fold channel which can be diagonalized with operator norm equal to its largest abstract value of its eigenvalues. This fact is used throughout the context in proving our results. The concept of frame potential works more general for non-Hermitian case, which we also use in Section III C to demonstrate that general ensembles approximating  $\text{SU}(d)$  symmetric  $k$ -design with arbitrary large  $k$  can never admit a constant locality.

Besides, applying the bi-invariance of Haar measure and Fubini theorem, which holds for well-behaved measures likes restricted Haar measures on compact subgroups, we note that  $T_k^\mathcal{E}$  commutes with  $T_k^G$ :

$$\begin{aligned} T_k^\mathcal{E} T_k^G(M) &= \int_{\mathcal{E}} \int_G V^{\otimes k} U^{\otimes k} M U^{\dagger \otimes k} V^{\dagger \otimes k} dU dV = \int_G U^{\otimes k} M U^{\dagger \otimes k} dU = T_k^G(M) \\ &= \int_{\mathcal{E}} \int_G U^{\otimes k} V^{\otimes k} M V^{\dagger \otimes k} U^{\dagger \otimes k} dU dV \\ &= \int_G \int_{\mathcal{E}} U^{\otimes k} V^{\otimes k} M V^{\dagger \otimes k} U^{\dagger \otimes k} dV dU = T_k^G T_k^\mathcal{E}(M). \end{aligned} \quad (41)$$

By Lemma II.3,  $T_k^G$  is always diagonalizable. Assume  $T_k^\mathcal{E}$  is Hermitian and hence diagonalizable, then they can be *simultaneously diagonalized*, e.g.,

$$T_k^G = \begin{pmatrix} 1 & & & \\ & 1 & & \\ & & 0 & \\ & & & 0 \end{pmatrix}, \quad T_k^\mathcal{E} = \begin{pmatrix} 1 & & & \\ & 1 & & \\ & & \lambda & \\ & & & \mu \\ & & & & \nu \end{pmatrix}. \quad (42)$$

Obviously, the eigenspace corresponding to the unit eigenvalue of  $T_k^G$  is exactly  $\text{Comm}_k(G)$  whose eigenvectors, by definition, also commute with the restricted representation on the ensemble  $\mathcal{E}$ . Therefore,

$$\text{Comm}_k(G) \subset \text{Comm}_k(\mathcal{E}). \quad (43)$$

as instantiate in Eq.(42). It is now clear that only when  $0 \leq |\lambda|, |\mu|, |\nu| < 1$ , applying  $T_k^\mathcal{E}$  many times, i.e., sampling from the ensemble into a circuit depth  $p$ , would approximate  $T_k^G$  in the sense of Definition II.2. Within this framework, evaluating

the upper bound of the *second largest abstract value* of these  $\lambda, \mu, \nu$  helps to determine the convergence speed of achieving unitary  $k$ -design through  $\mathcal{E}$ . The case when  $T_k^\mathcal{E}$  is non-Hermitian is tackled by calculating the frame potential introduced in the subsequent subsection.

As a basic application of this perspective, suppose  $\mathcal{E}$  is taken as a compact subgroup of  $G$ , e.g, an one-parameter subgroup, equipped with the Haar measure inherited from that of  $G$ . Then  $T_k^\mathcal{E}$  is also a projector and the eigenvalues  $\lambda, \mu, \nu$  exemplified above is either 0 or 1. Therefore,  $T_k^\mathcal{E} = T_k^G$  if and only if  $\text{Comm}_k(\mathcal{E}) = \text{Comm}_k(G)$  which further indicates the following simple but significant result:

**Theorem II.4.** *If the unitary ensemble  $\mathcal{E}$  is taken as a compact Lie subgroup of  $G$  with restricted Haar measure, then either  $\mathcal{E}$  forms exact unitary  $k$ -design or it can never form any design even in the approximate sense.*

As an immediate and insightful example, one-parameter subgroups generally do not even form approximate  $k$ -design when the ambient group  $G$  is of large dimension. However, ensembles consisting of various one-parameter subgroups may fulfill the task. With further condition being specified, we verify this in Section IV A for ensembles motivated by CQA.

We now review the relationship between unitary  $k$ -design and *random walks on compact groups* [43–45], which would elaborate the strategy of computing second largest eigenvalue with more deep insights from probability and representation theory of groups. To begin with, let us define the convergence of measures over groups:

**Definition II.5.** Suppose  $\{\mu_p\}$  is a sequence of probability densities/measures over a compact group  $G$ , then it *converges under the weak star topology*, or simply *converges weakly*, to the Haar measure  $\mu$ , denoted by  $\mu_p \xrightarrow{w} \mu$ , if for any continuous (and automatically bounded) function  $f$  defined on  $G$ ,

$$\lim_{p \rightarrow \infty} \int_G f(g) d\mu_p(g) = \int_G f(g) d\mu(g) \text{ or equivalently } \lim_{p \rightarrow \infty} \mathbb{E}_{\mu_p}(f) = \mathbb{E}_\mu(f). \quad (44)$$

Note that the limit is considered independently for each single function  $f$ . Requiring the *uniform convergence* for all  $f$  is somewhat too strong on continuous compact groups [43, 45].

In order to check whether  $\mu_p \rightarrow \mu$  in this sense, we have the following famous Lévy continuity theorem generalized from classical Euclidean space to compact group which translates the convergence of expectations by *Fourier transformation* to the convergence of certain operators acting on irreducible representations of  $G$ .

**Theorem II.6** (Lévy continuity theorem). [44] *Given any irrep  $\pi$  of the compact group  $G$  and any density function  $\nu$ , the operator*

$$\hat{\nu}(\pi) := \int_G \pi(g) d\nu(g) \quad (45)$$

*acting on the representation space of  $\pi$  is called the Fourier transform or characteristic function of  $\nu$ . The convergence of  $\mu_n \rightarrow \mu$  defined above is equivalent to the convergence of matrix entries  $\hat{\mu}_n(\pi)_{ij} \rightarrow \hat{\mu}(\pi)_{ij}$  for all inequivalent  $G$  irreps.*

Let us check the Fourier transformation of the Haar measure  $\mu$ :

$$\hat{\mu}(\pi) = \int_G \pi(g) d\mu(g) = \begin{cases} 1 & \pi \text{ is the trivial representation} \\ 0 & \text{otherwise} \end{cases}. \quad (46)$$

This is due to the so-called *Schur orthogonality* which we formally introduce and use in Section III A. Since  $\hat{\mu}_n(\pi) \equiv 1$  on the trivial representation, the operator norm

$$\left\| \bigoplus_\lambda \hat{\mu}_n(\pi) - \bigoplus_\lambda \hat{\mu}(\pi) \right\| \quad (47)$$

taking over all inequivalent  $G$  irreps or the second largest abstract value of eigenvalues of  $\bigoplus_\lambda \hat{\mu}_n(\pi)$  (if they are diagonalizable) determine whether and how fast  $\mu_n$  converges to  $\mu$ .

*Remark.* A *random walk* on the group  $G$  is simply a sequence  $\{S_n\}$  of *random variables*  $S_n = X_1 \cdots X_n$  for which  $X_i$  are *independent* random variable with values in the group  $G$  distributed according to the same density  $\nu$ . This induces a sequence of densities  $\{\nu^{*n}\}$  with which one can examine its convergence via the previous theorem.

On the other hand, on a quantum circuit, we define the  $k$ -fold channel

$$T_k^\mathcal{E} = \int_{\mathcal{E}} V^{\otimes k} \otimes \bar{V}^{\otimes k} dV \quad (48)$$

of an ensemble  $\mathcal{E}$  and compare it with  $T_k^G$ . The ensemble would be applied several times which imitates a random walk on the quantum circuit and we note that the tensor product  $V^{\otimes k} \otimes \bar{V}^{\otimes k}$  from the integral can be in principle decomposed further with respect to the irreps of  $G$ , therefore we may interpret  $T_k^{\mathcal{E}}$  as a *truncated* Fourier transform of the measure  $\nu$  associated to  $\mathcal{E}$ , which tells the reason to compute  $\|(T_k^{\mathcal{E}})^p - T_k^G\|$  as in the example of Eq.(42) from a viewpoint of random walk.

It should be careful that unitary  $k$ -design is a weaker concept than the convergence of measures. For instance,  $SU(N)$  is an exact  $k$ -design to  $U(N)$  for arbitrary  $k$ , but  $SU(N) \neq U(N)$  and hence there is no reason to say that the Haar measure of  $SU(N)$  converges to that of  $U(N)$ . Even comparing the integral with respect to these measures, there are still counterexamples: let  $\det$  denote the determinant function. Then

$$\int_{SU(N)} \det V dV = 1 \neq \int_{U(N)} \det U dU = 0. \quad (49)$$

The formal reason is that there is no guarantee that  $V^{\otimes k} \otimes \bar{V}^{\otimes k}$  encompasses all inequivalent irreps even when  $k \rightarrow \infty$ , e.g., the 1-dimensional representation  $\det$  given by taking determinant [1, 3]. However, unitary  $k$ -design is more practical and reasonably fits into the case of quantum computation where we twirl states or density matrices by unitaries as  $U^{\otimes k} \rho U^{\dagger \otimes k}$ . Henceforth, instead of worrying about the convergence of arbitrary function as in Eq.(44), we only focus on functions involves entries and their conjugates of  $U$  equally which can be expanded by homogeneous polynomials of these variables captured by unitary  $k$ -design [35]. Nevertheless, representation theory are still of great importance and used throughout this work.

### C. Frame Potential, Form factors, and $k$ -Invariance

We now show that the perspective of defining  $k$ -fold channel and computing their second largest eigenvalues are tightly related with the following two quantities: the *spectral form factor*  $R_{2k}^{\mathcal{E}}$  and the *frame potential*  $F_{\mathcal{E}}^{(k)}$  developed and used in recent physics literature [35–40]. The former is defined as

$$R_{2k}^{\mathcal{E}} := \int_{\mathcal{E}} dU |\text{tr}(U)|^{2k}. \quad (50)$$

Using the facts that traces interchange with integrals and the identity  $\text{tr}(U \otimes V) = \text{tr} U \text{tr} V$ , we get

$$R_{2k}^{\mathcal{E}} = \text{tr} \left( \int_{\mathcal{E}} U^{\otimes k} \otimes \bar{U}^{\otimes k} dU \right) = \text{tr} T_k^{\mathcal{E}}. \quad (51)$$

Especially when  $\mathcal{E} = G$ ,  $R_{2k}^G = \text{tr} T_k^G$  measures precisely the *dimension* of the commutant  $\text{Comm}_k(G)$  explained previously. For  $k$ -design without symmetry, we set  $G = U(d^n) \equiv U(N)$ . It is well-known by Schur-Weyl duality that  $R_{2k}^G = k!$  when  $k < d^n = N$  [3, 4]. In the most general setting for arbitrary large  $k$ ,  $R_{2k}^G$  is proved to be equal to the number of permutations having no *increasing subsequence* of length greater than  $d^n$  [46], which relates to the so-called *increasing subsequence problem* from combinatorics [2].

The frame potential characterizes the 2-norm distance between a given ensemble and the Haar random unitary:

$$F_{\mathcal{E}}^{(k)} = \int_{\mathcal{E}} dU dV \|\text{tr}(UV^{\dagger})\|^{2k} \quad (52)$$

Comparing with spectral form factor, frame potential is defined for a more general choices of the ensembles:

**Proposition II.7.** Given an arbitrary ensemble  $\mathcal{E}$ ,

$$F_{\mathcal{E}}^{(k)} = \text{tr}(T_k^{\mathcal{E} \dagger} T_k^{\mathcal{E}}). \quad (53)$$

As an immediate result, if  $T_k^{\mathcal{E}}$  is Hermitian,  $F_{\mathcal{E}}^{(k)} = \text{tr}((T_k^{\mathcal{E}})^2)$ . When  $\mathcal{E}$  is compact subgroup,

$$F_{\mathcal{E}}^{(k)} = R_{2k}^{\mathcal{E}}. \quad (54)$$

In either cases, the frame potential is lower-bounded by  $F_G^{(k)} = R_{2k}^G$ .

*Proof.* Just as we derive  $R_{2k}^{\mathcal{E}} = \text{tr} T_k^{\mathcal{E}}$  from above,

$$\begin{aligned} F_{\mathcal{E}}^{(k)} &= \int_{U, V \in \mathcal{E}} |\text{tr}(U^{\dagger} V)|^{2k} dV dU = \int_{U, V \in \mathcal{E}} \text{tr}((U^{\dagger} V)^{\otimes k} \otimes (\overline{U^{\dagger} V})^{\otimes k}) dV dU \\ &= \text{tr} \int_{U, V \in \mathcal{E}} (U^{\dagger} V)^{\otimes k} \otimes (\overline{U^{\dagger} V})^{\otimes k} dV dU = \text{tr} \int_{U \in \mathcal{E}} \int_{V \in \mathcal{E}} (U^{\dagger \otimes k} \otimes \bar{U}^{\dagger \otimes k}) (V^{\otimes k} \otimes \bar{V}^{\otimes k}) dV dU \\ &= \text{tr} (T_k^{\mathcal{E} \dagger} T_k^{\mathcal{E}}). \end{aligned} \quad (55)$$

When  $\mathcal{E}$  is taken as a compact subgroup of  $G$  with the restricted Haar measure,  $T_k^\mathcal{E} = T_k^{\mathcal{E}\dagger}$  becomes a projector by Lemma II.3. Then

$$F_\mathcal{E}^{(k)} = \text{tr}((T_k^\mathcal{E})^2) = \text{tr} T_k^\mathcal{E} = R_{2k}^\mathcal{E}. \quad (56)$$

Finally, no matter  $T_k^\mathcal{E}$  is Hermitian or not,  $T_k^{\mathcal{E}\dagger} T_k^\mathcal{E}$  is always diagonalizable with nonnegative eigenvalues. Let  $W_{k,\mathcal{E}}^{\lambda=1}$  denote its unit eigenspace, as the example of Eq.(42), for any  $M \in \text{Comm}_k(G)$ ,

$$\begin{aligned} U^{\otimes k} M &= U^{\otimes k} M, U^{\dagger \otimes k} M = U^{\dagger \otimes k} M \\ \implies T_k^{\mathcal{E}\dagger} T_k^\mathcal{E}(M) &= M \\ \implies F_G^{(k)} &= R_{2k}^G = \text{tr}(T_k^G) = \dim \text{Comm}_k(G) \leq \dim W_{k,\mathcal{E}}^{\lambda=1} \leq F_\mathcal{E}^{(k)}. \end{aligned} \quad (57)$$

This finishes the proof.  $\square$

Note that the last statement  $F_G^{(k)} \leq F_\mathcal{E}^{(k)}$  is verified directly using the bi-invariance of Haar measure in literature [36–40] when comparing the real Haar randomness with that assigned by the ensemble  $\mathcal{E}$ . Our method incorporates insights from commutant theory which will shows its usefulness in Section III C and IV A.

We now introduce the  $k$ -invariance [39] which characterizes how invariant it is under the Haar random unitary. For a given ensemble,  $k$ -invariance  $I_\mathcal{E}^{(k)}$  is defined by

$$I_\mathcal{E}^{(k)} = F_\mathcal{E}^{(k)} - \tilde{F}_\mathcal{E}^{(k)} \quad (58)$$

where  $\tilde{\mathcal{E}}$  is obtained from averaging  $\mathcal{E}$  over the Haar measure

$$\tilde{\mathcal{E}} = \left\{ \int_G dW (W U W^\dagger) : U \in \mathcal{E} \right\} \quad (59)$$

By simialr methods used above,

$$\begin{aligned} F_{\tilde{\mathcal{E}}}^{(k)} &= \text{tr} \left( \left( \int_{\tilde{\mathcal{E}}} d\tilde{U} \int_{\tilde{\mathcal{E}}} d\tilde{V} \left( \tilde{U}^{\dagger \otimes k} \otimes \tilde{U}^{\dagger \otimes k} \right) (V^{\otimes k} \otimes \bar{V}^{\otimes k}) \right) \right) \\ &= \text{tr} \left( \int_{\mathcal{E}} dU \int_G dW \int_{\mathcal{E}} dV \int_G dX \left( (W U^\dagger W^\dagger)^{\otimes k} \otimes (\overline{W U^\dagger W^\dagger})^{\otimes k} \right) \left( (X V X^\dagger)^{\otimes k} \otimes (\overline{X V X^\dagger})^{\otimes k} \right) \right) \\ &= \text{tr} \left( (T_k^G T_k^{\mathcal{E}\dagger} T_k^G) (T_k^G T_k^\mathcal{E} T_k^G) \right) = \text{tr} \left( T_k^G T_k^{\mathcal{E}\dagger} T_k^\mathcal{E} T_k^G \right) = \text{tr}(T_k^G). \end{aligned} \quad (60)$$

Obviously, the  $k$ -invariance  $I_\mathcal{E}^{(k)} \geq 0$ . If  $\mathcal{E}$  is an exact  $k$ -design,  $I_\mathcal{E}^{(k)} = 0$ . We say that any ensemble for which  $I_\mathcal{E}^{(k)} = 0$  is  $k$ -invariant.

*Remark.* With the previous introduction on commutant, eigenvalues or spectral of  $k$ -fold channel and frame potential, we now reveal their relationship. Given an arbitrary ensemble  $\mathcal{E}$  with measure  $\nu$ , we sample unitaries from the ensemble  $\mathcal{E}$  into a circuit depth  $p$ , or we take a  $p$  steps random walk via the ensemble, which by definition yields the twirling channel  $(T_k^\mathcal{E})^p$ . We also assume that  $T_k^\mathcal{E}$  is Hermitian with nonnegative eigenvalues (*positive semidefinite*). This assumption holds for all CQA ensembles defined in Section IV A. If  $T_k^\mathcal{E}$  is exotically non-Hermitian, we consider the operator  $T_k^{\mathcal{E}\dagger} T_k^\mathcal{E}$  instead.

With this assumption, in the language of commutant theory, we evaluate the *second largest eigenvalue*  $\lambda$  of  $T_k^\mathcal{E}$ . It has been shown in [26, 31, 32] that to obtain an  $\epsilon$ -approximate  $k$ -design  $\|(T_k^\mathcal{E})^p - T_k^G\|_\diamond \leq \epsilon$ ,

$$p = \frac{1}{\log 1/\lambda} \log \frac{N^{2k}}{\epsilon}. \quad (61)$$

Since for large  $x$ ,  $x \leq (x+1) \log(x+1)$ ,

$$\frac{1}{\log \frac{1}{\lambda}} = \frac{1}{\log \frac{1-\lambda}{\lambda} + 1} \leq \frac{\frac{1-\lambda}{\lambda} + 1}{\frac{1-\lambda}{\lambda}} = \frac{1}{1-\lambda} \implies p \leq \frac{1}{1-\lambda} \log \frac{N^{2k}}{\epsilon}. \quad (62)$$

Therefore, a polynomial *spectral gap* between first and second largest eigenvalues of  $T_k^\mathcal{E}$  guarantees an efficient random circuit scheme (also see [41, 42]).

On the other hand, suppose we turn to estimate the frame potential  $F_{\mathcal{E}}^{(k)}(p)$  for each step  $p$ . Then the inequality

$$\|(T_k^{\mathcal{E}})^p - T_k^G\|_{\diamond}^2 \leq N^{2k} \left( F_{\mathcal{E}}^{(k)}(p) - F_G^{(k)} \right) \quad (63)$$

can be applied to bound the difference under diamond norm [38–40]. By Proposition II.7, knowing both the second largest eigenvalue  $\lambda$  and  $F_G^{(k)} = \dim \text{Comm}_k(G)$  is sufficient to bound

$$F_{\mathcal{E}}^{(k)}(p) = \text{tr}((T_k^{\mathcal{E}})^{2p}) = \sum_i \lambda_i^{2p}, \quad (64)$$

where  $\lambda_i$  denote eigenvalues of  $T_k^{\mathcal{E}}$ . Conversely, knowing  $F_{\mathcal{E}}^{(k)}(p)$  for all  $p \in \mathbb{N}$  determines these eigenvalues  $\lambda_i$  uniquely by the so-called *moment problem* studied in number theory and algebraic geometry [47]. Even it is generally impossible to solve  $\lambda_i$  explicitly in Eq.(64), this consideration finally relates the concepts of frame potential, commutant, operator traces and eigenvalues together in approximating  $k$ -design.

#### D. Commutant of the Group $U(\bigoplus_\lambda S^\lambda)$ of $SU(d)$ Symmetric Unitaries

In later sections proving our main results on unitary  $k$ -design under  $SU(d)$  symmetry, we always adopt the approach using  $S_n$  representation theory and analyzing commutant and eigenvalues, instead of computing the frame potential. At the end of this section, we explain the potential difficulty of working with frame potential at the presence of  $SU(d)$  symmetry and describe the commutant of  $U(\bigoplus_\lambda S^\lambda)$  with a explicit spanning set, which stands at the center for our computation of  $T_{k=2}^{\text{CQA}}(M)$  to analyze several related applications in [48].

To motivate the following proof, we first consider the commutant algebra  $\text{Comm}_k(U(d^n))$  for a generic  $n$ -qudit system  $H = V^{\otimes n}$  with no symmetry. It is well-known by Schur-Weyl duality and double commutant theorem [3, 4] that

$$\text{Comm}_k(U(d^n)) = \text{span}\{\sigma, \sigma \in S_k\}, \quad (65)$$

where  $\sigma$  should be understood as the permutation on the  $k$ -fold tensor product  $H^{\otimes k}$  (cf. permutations on  $n$  qudits). Let us move furthermore to express  $\sigma$  explicitly. To this end, we note that any  $M \in \text{Comm}_k(U(N))$  is just an element from  $\text{End}(H^{\otimes k})$  which possess a standard basis given by tensor products of matrix units, i.e., matrices  $E_{ij}$  with unit entry in the position  $(i, j)$  and zero entries elsewhere. Under computational basis  $\{|i\rangle\}_{i=1}^N$ ,

$$E_{ij} = |i\rangle \langle j|. \quad (66)$$

Then it is straightforward to check by definition that

$$\sum_{i,j} E_{ii} \otimes E_{jj}, \quad \sum_{i,j} E_{ij} \otimes E_{ji}, \quad \sum_{i,j,k,r,s} E_{is} \otimes E_{jk} \otimes E_{kr} \otimes E_{rj} \otimes E_{si} \quad (67)$$

correspond respectively to the identity matrix, the transposition  $(1, 2)$  on the first two indices, and the permutation  $(15)(234)$  which swaps the first and fifth indices while translates the second, third and forth indices cyclically. Note that we define these operators on  $H^{\otimes k}$  for arbitrary  $k$ , but we omit the cumbersome tensor products with identity matrix  $I$  in the above expression. A general permutation  $\sigma$  of cycle type  $\mu = (\mu_1, \dots, \mu_r) \vdash k$  (Definition I.3) can be written out following this procedure: when there is a basis vector label  $i$  appearing as a covariant/contravariant index of some matrix unit from the tensor product, it should be assigned again as a contravariant/covariant index. Except using computational basis, permutations can also be expanded by (generalized) Pauli matrices with nice properties being used in several applications [48]. Any of these expansions are significant to study common unitary  $k$ -design [26, 33, 36].

We now discuss the more involved case for  $\text{Comm}_k(U(\bigoplus_\lambda S^\lambda))$ . Recall that as we study  $SU(d)$  symmetric quantum circuit, the entire Hilbert space  $H = V^{\otimes n}$  of qudits decomposes by Schur-Weyl duality into irreps  $S^\lambda$  of  $S_n$  with multiplicities  $m_{S_n, \lambda}$  (Section IB):

$$H \cong \bigoplus_{\lambda} I_{m_{S_n, \lambda}} \otimes S^\lambda. \quad (68)$$

We also introduced in Section I A spanning these irreps by Young-Yamanouchi basis. Thus we change from computational basis  $\{|i\rangle\}$  to Young basis  $\{|\alpha_T, m\rangle\}$ , with  $\alpha_T$  labeling a basis vector and  $m$  recording the irrep multiplicity by Schur transform [4, 5, 24] and redefine the matrix unit as

$$E_{(\alpha_T, m), (\alpha_{T'}, m')} = |\alpha_T, m\rangle \langle \alpha_{T'}, m'|. \quad (69)$$

It turns out that the commutant  $\text{Comm}_k(U(\bigoplus_\lambda S^\lambda))$  is spanned by "permutations" generalized from Eq.(67) using  $E_{(\alpha_T, m), (\alpha_{T'}, m')}$ . As the simplest but enlightening example, we have

$$\sum_{T_1, T_2} E_{(\alpha_{T_1}, m_1), (\alpha_{T_1}, m'_1)} \otimes E_{(\alpha_{T_2}, m_2), (\alpha_{T_2}, m'_2)} \quad (70)$$

generalized from  $\sum_{i,j} E_{ii} \otimes E_{jj}$ . However, Eq.(70) no longer represents the identity matrix because the summation is taken within two  $S_n$  irreps labeled by the Young diagrams of  $T_1, T_2$ , but not over the entire space  $H^{\otimes k}$ . Besides, the multiplicity indices can vary arbitrarily: there is *no need* to require  $m_1 = m'_1$  or  $m_2 = m'_2$ . We only couple each basis vector label in pair as covariant and contravariant indices. Moreover, when  $k = 2$  or  $5$ ,

$$\sum_{T_1, T_2} E_{(\alpha_{T_1}, m_1), (\alpha_{T_2}, m_2)} \otimes E_{(\alpha_{T_2}, m'_2), (\alpha_{T_1}, m'_1)}, \quad (71)$$

$$\begin{aligned} \sum_{T_1, T_2, T_3, T_4, T_5} E_{(\alpha_{T_1}, m_1), (\alpha_{T_5}, m_5)} \otimes E_{(\alpha_{T_2}, m_2), (\alpha_{T_3}, m_3)} \\ \otimes E_{(\alpha_{T_3}, m'_3), (\alpha_{T_4}, m_4)} \otimes E_{(\alpha_{T_4}, m'_4), (\alpha_{T_2}, m'_2)} \otimes E_{(\alpha_{T_5}, m'_5), (\alpha_{T_1}, m'_1)}, \end{aligned} \quad (72)$$

show how to generalize the left two examples from Eq.(67). With all these preparation, we prove the following theorem:

**Theorem II.8.** *The commutant  $\text{Comm}_k(U(\bigoplus_\lambda S^\lambda))$  is spanned by a generalized form of permutations exemplified in Eq.(70) and Eq.(71).*

*Proof.* By definition, matrix representations  $U$  of group elements  $g \in U(\bigoplus_\lambda S^\lambda)$  are just collections of unitary matrices acting on inequivalent  $S_n$  irrep blocks with identical copies on the multiplicity spaces (Eq.(30)). Thus the conjugation action of  $U(\bigoplus_\lambda S^\lambda)$  on any simple tensor product of matrix units is given by,

$$(U_1 E_{(\alpha_{T_1}, m_1), (\alpha_{T_2}, m_2)} U_2^\dagger) \otimes (U_3 E_{(\alpha_{T_3}, m_3), (\alpha_{T_4}, m_4)} U_4^\dagger) \otimes \cdots \otimes (U_{2k-1} E_{(\alpha_{T_{2k-1}}, m_{2k-1}), (\alpha_{T_{2k}}, m_{2k})} U_{2k}^\dagger) \quad (73)$$

where  $U_i$  are unitaries acting on decomposed  $S_n$  irreps spanned by  $\{|\alpha_{T_i}\rangle\}$ . A generic element  $M \in \text{End}(H^{\otimes k})$  is a linear combination of simple tensor products of matrix units:

$$M = \sum_{T_i, M_i} c_{T_i, M_i} E_{(\alpha_{T_1}, m_1), (\alpha_{T_2}, m_2)} \otimes E_{(\alpha_{T_3}, m_3), (\alpha_{T_4}, m_4)} \otimes \cdots \otimes E_{(\alpha_{T_{2k-1}}, m_{2k-1}), (\alpha_{T_{2k}}, m_{2k})}, \quad (74)$$

as they form a standard basis for  $\text{End}(H^{\otimes k})$ . Belonging to  $\text{Comm}_k(U(\bigoplus_\lambda S^\lambda))$  means being invariant under the conjugate action for arbitrary  $U = \rho(g)$ .

We first select  $U_i$  as arbitrary diagonal phase matrices. Then the conjugate action accounts for scalar products with phase factors on each simple tensor. Since these simple tensors are linearly independent, being invariant under phase change implies such invariance for individual simple tensor from Eq.(74), which leads to the requirement on coupling basis vector labels in pairs of covariant and contravariant indices. For instance, when  $k = 2$ , phase-change invariant simple tensors are of the following forms:

$$(U_1 E_{(\alpha_{T_1}, m_1), (\alpha_{T_1}, m'_1)} U_1^\dagger) \otimes (U_2 E_{(\alpha_{T_2}, m_2), (\alpha_{T_2}, m'_2)} U_2^\dagger) \quad (75)$$

or

$$(U_1 E_{(\alpha_{T_1}, m_1), (\alpha_{T_2}, m_2)} U_2^\dagger) \otimes (U_2 E_{(\alpha_{T_2}, m'_2), (\alpha_{T_1}, m'_1)} U_1^\dagger). \quad (76)$$

With this example, let  $U_1$  be matrices exchanging arbitrary rows and columns like

$$U_1 = \begin{pmatrix} 1 & 0 & 0 \\ 0 & 0 & 1 \\ 0 & 1 & 0 \end{pmatrix} \quad (77)$$

while we set  $U_2$  being the identity matrix. Conjugated by this kind of  $U(\bigoplus_\lambda S^\lambda)$  group elements, the basis vector label  $\alpha_{T_1}$  varies arbitrarily inside the  $S_n$  irrep acted on by  $U_1$ . Therefore, being invariant indicates that we should take summations over  $T_1, T_2$  which yield:

$$\sum_{T_1, T_2} E_{(\alpha_{T_1}, m_1), (\alpha_{T_1}, m'_1)} \otimes E_{(\alpha_{T_2}, m_2), (\alpha_{T_2}, m'_2)} \quad (78)$$

and

$$\sum_{T_1, T_2} E_{(\alpha_{T_1}, m_1), (\alpha_{T_2}, m_2)} \otimes E_{(\alpha_{T_2}, m'_2), (\alpha_{T_1}, m'_1)}. \quad (79)$$

However, these consideration have no influence on the choices of multiplicity labels  $m_i$  and that is why they are assigned arbitrarily.

We still need to prove that operators  $M$  spanned with the above requirements commutes all other unitaries from  $U(\bigoplus_\lambda S^\lambda)$ . This is done by arguing through the Lie algebra  $\mathfrak{g} = \mathfrak{L}(U(\bigoplus_\lambda S^\lambda))$  consisting of

$$E \otimes I \otimes \cdots \otimes I + I \otimes E \otimes \cdots \otimes I + \cdots I \otimes \cdots \otimes I \otimes E \in \text{End}(H^{\otimes k}) \quad (80)$$

with  $E$  being an anti-Hermitian matrix respecting the decomposition of  $H^{\otimes k}$  under  $SU(d)$  symmetry. We expand  $E$  by matrix units and examine the commutativity: Using the example:

$$M = \sum_{T_1, T_2} E_{(\alpha_{T_1}, m_1), (\alpha_{T_2}, m_2)} \otimes E_{(\alpha_{T_2}, m'_2), (\alpha_{T_1}, m'_1)}, \quad (81)$$

we have

$$(E_{(\alpha_T, m), (\alpha_{T'}, m')} \otimes I)M = \sum_{T_2} E_{(\alpha_T, m), (\alpha_{T_2}, m_2)} \otimes E_{(\alpha_{T_2}, m'_2), (\alpha_{T'}, m')} = M(I \otimes E_{(\alpha_T, m), (\alpha_{T'}, m')}) \quad (82)$$

by contracting the same tensor indices. Analogously,  $(I \otimes E_{(\alpha_T, m), (\alpha_{T'}, m')})M = M(E_{(\alpha_T, m), (\alpha_{T'}, m')} \otimes I)$  and hence  $M$  commutes with the Lie algebra elements. Generally case for arbitrary  $k$  is deduced similarly and we complete the proof.  $\square$

*Remark.* With this theorem, let us try to compute the frame potential  $F_{\text{Haar}}^{(k)}$  for  $G = U(\bigoplus_\lambda S^\lambda)$ . The simplest case is  $k = 1$ , when  $\text{Comm}_k(U(\bigoplus_\lambda S^\lambda))$  is spanned by

$$\sum_T E_{(\alpha_T, m), (\alpha_T, m')} \quad (83)$$

for each  $S_n$  irrep appearing in the decomposition and with arbitrary copies. When the system consists of  $n$ -qubits, Schur-Weyl duality says that there are  $p(n, 2) = \lfloor \frac{n}{2} \rfloor + 1$  inequivalent  $S_n$  irreps corresponding to two-row Young diagrams in the decomposition. Moreover, the multiplicity of the irrep  $S^\lambda$  with  $\lambda = (n - r, r)$  is  $n - 2r + 1$ . Therefore, for qubits,

$$F_{\text{Haar}}^{(1)} = \dim \text{Comm}_{k=1}(U(\bigoplus_\lambda S^\lambda)) = \sum_{0 \leq r \leq \lfloor n/2 \rfloor} (n - 2r + 1)^2. \quad (84)$$

When  $k = 2$ ,

$$\begin{aligned} F_{\text{Haar}}^{(2)} = \dim \text{Comm}_{k=2}(U(\bigoplus_\lambda S^\lambda)) &= (n+1)^4 + 2 \sum_{1 \leq r \leq \lfloor n/2 \rfloor} (n - 2r + 1)^4 \\ &+ 2 \sum_{0 \leq r \neq s \leq \lfloor n/2 \rfloor} (n - 2r + 1)^2 (n - 2s + 1)^2, \end{aligned} \quad (85)$$

where the first two terms in the RHS appears when four indices of basis vectors  $\alpha_T$  from Eq.(70) are all selected from an equivalent  $S_n$  irrep. As the trivial irrep ( $r = 1$ ) of  $S_n$  is 1-dimensional with no freedom for exchanging indices, we separate it from the second term. The third term counts the case when two pairs of indices are chosen from two inequivalent  $S_n$  irreps. Then general case follows as above.

For qudits, the number of inequivalent  $S_n$  irreps is  $p(n, d)$  which denotes the number of Young diagrams with  $n$  boxes and at most  $d$  rows (Definition I.4). Unfortunately, there is no closed formula for  $p(n, d)$ , except the asymptotic formula due to Ramanujan, Hardy and Uspensky [12, 13], and later developed bounds in [16, 17] Consequently, it may not be easy to calculate the frame potential  $F_{\text{Haar}}^{(k)}$  for the group of  $SU(d)$  symmetric unitaries, no to mention comparing it with  $F_{\mathcal{E}}^{(k)}$  in (63). To bypass this obstacle to some extent, we would work exclusively with commutant algebra  $\text{Comm}_k(U(\bigoplus_\lambda S^\lambda))$  in the following context to present our main results.



### III. ESTABLISHING EXACT $k$ -DESIGN WITH $SU(d)$ SYMMETRY BY CQA

We elucidate our result on exact  $k$ -design with the presence of  $SU(d)$  symmetry in this section. We prove that, for a general  $n$ -qudit system, the group CQA generated by unitary time evolution of SWAPs and second order YJM-elements is an exact  $k$  design with  $SU(d)$  symmetry for  $k = \Omega(n^2)$  (Theorem III.4). We verify that in order to extend this result for arbitrary large  $k$ , non-local unitaries are indispensable (Theorem III.6), which is significantly different from the case with no symmetry where 2-local unitaries are always enough to approximate Haar randomness [26, 27, 34]. At the price of increasing locality, we also provide a constructive way to achieve arbitrary  $k$ -design by employing  $k$ th-order YJM-elements (Theorem III.11). Proofs in this section are largely based on group representation theory [1, 3] and Okounkov-Vershik approach [4, 9].

#### A. Comparison of the $k$ -fold Channels $T_k^{SU}$ and $T_k^{\text{Haar}}$

It is easy to see by definition that for arbitrary  $N$  and  $k$ ,  $SU(N)$  is an exact  $k$ -design for  $U(N)$ :

$$T_k^{SU(N)} = \int_{SU(N)} V^{\otimes k} \otimes \bar{V}^{\otimes k} d\nu = \int_{U(N)} U^{\otimes k} \otimes \bar{U}^{\otimes k} d\mu = T_k^{U(N)}. \quad (86)$$

where  $\nu$  is the restricted Haar measure from  $\mu$  on  $SU(N)$ . Apparently, any *global phase* from  $U \in U(N)$  would get canceled after taking the tensor product  $U \otimes \bar{U}$  and hence the above integrals are identical. However, this is in general not true for  $T_k^{SU}, T_k^{\text{Haar}}$  – the  $k$ -fold channels twirled over the groups  $SU(\bigoplus_\lambda S^\lambda)$ ,  $U(\bigoplus_\lambda S^\lambda)$  respectively. Intuitively speaking, with the entire Hilbert space  $H = V^{\otimes n}$  of  $n$ -qudits being decomposed into various  $S_n$  irreps, the integrand in calculating  $T_k^{SU}, T_k^{\text{Haar}}$  becomes intricate with tensor products of various sub-matrices defined on these irrep sectors (see Section I B). In this subsection, we prove rigorously when  $SU(\bigoplus_\lambda S^\lambda)$  fails to form an exact design of  $U(\bigoplus_\lambda S^\lambda)$ , which paves the way for understanding more advanced cases involving YJM-elements and CQA later.

To motivate our statement, we assume the simplest nontrivial case when there are only two inequivalent  $S_n$  irreps decomposed from the system:  $S^{\lambda_1}$  and  $S^{\lambda_2}$  of dimension  $d_1$  and  $d_2$  respectively. Then  $g \in SU(\bigoplus_\lambda S^\lambda)$  is represented as (cf. Eq.(30) and Theorem II.8)

$$\begin{pmatrix} V_1 & \\ & V_2 \end{pmatrix} = V_1 \oplus V_2, \quad (87)$$

where  $V_i \in SU(d_i)$  and we write  $U_i = e^{-i\phi} V_i \in U(d_i)$  if  $g$  is taken from  $U(\bigoplus_\lambda S^\lambda)$ . Then the integrand

$$g^{\otimes k} \otimes \bar{g}^{\otimes k} = (V_1 \oplus V_2)^{\otimes k} \otimes (\bar{V}_1 \oplus \bar{V}_2)^{\otimes k} \quad (88)$$

can be expanded as the following direct sums of tensor products:

$$(V_1^{\otimes r} \otimes V_2^{\otimes k-r} \otimes \bar{V}_1^{\otimes s} \otimes \bar{V}_2^{\otimes k-s}) \oplus \cdots \oplus (V_2^{\otimes r'} \otimes V_1^{\otimes k-r'} \otimes \bar{V}_2^{\otimes s'} \otimes \bar{V}_1^{\otimes k-s'}). \quad (89)$$

As a result,  $T_k^{SU}$ , as well as  $T_k^{\text{Haar}}$ , is just a direct sum of integrals with these tensor products:

$$\left( \int_{SU(\bigoplus_\lambda S^\lambda)} V_1^{\otimes r} \otimes U_2^{\otimes k-r} \otimes \bar{V}_1^{\otimes s} \otimes \bar{U}_2^{\otimes k-s} d\mu_1 d\mu_2 \right) \oplus \cdots \oplus \left( \int_{SU(\bigoplus_\lambda S^\lambda)} V_2^{\otimes r'} \otimes U_1^{\otimes k-r'} \otimes \bar{V}_2^{\otimes s'} \otimes \bar{U}_1^{\otimes k-s'} d\mu_1 d\mu_2 \right) \quad (90)$$

Being different from Eq.(86), each integral is evaluated on both  $SU(d_1)$  and  $SU(d_2)$  under our assumption that the space decomposes as  $S^{\lambda_1} \oplus S^{\lambda_2}$ . We now show by representation theory that one can always find certain  $r, s$  such that

$$\int_{SU(\bigoplus_\lambda S^\lambda)} V_1^{\otimes r} \otimes V_2^{\otimes k-r} \otimes \bar{V}_1^{\otimes s} \otimes \bar{V}_2^{\otimes k-s} d\nu_1 d\nu_2 \neq 0 = \int_{U(\bigoplus_\lambda S^\lambda)} U_1^{\otimes r} \otimes U_2^{\otimes k-r} \otimes \bar{U}_1^{\otimes s} \otimes \bar{U}_2^{\otimes k-s} d\mu_1 d\mu_2. \quad (91)$$

With lots of similar counterexamples from other direct sum components from Eq.(89), we conclude that  $T_k^{SU} \neq T_k^{\text{Haar}}$  generally.

To handle integrals over various compact groups, we first rearrange  $U_1^{\otimes r} \otimes U_2^{\otimes k-r} \otimes \bar{U}_1^{\otimes s} \otimes \bar{U}_2^{\otimes k-s}$  to  $(U_1^{\otimes r} \otimes \bar{U}_1^{\otimes s}) \otimes (U_2^{\otimes k-r} \otimes \bar{U}_2^{\otimes k-s})$  and then apply Fubini theorem to evaluate

$$\left( \int U_1^{\otimes r} \otimes \bar{U}_1^{\otimes s} d\mu_1 \right) \otimes \left( \int U_2^{\otimes k-r} \otimes \bar{U}_2^{\otimes k-s} d\mu_2 \right). \quad (92)$$

Rearrangements are invertible on tensor products and hence to obtain the evidence in Eq.(91), we just need to check whether the above integral vanishes on  $\text{SU}(\bigoplus_\lambda S^\lambda)$  or  $\text{U}(\bigoplus_\lambda S^\lambda)$ .

When we integrate over  $\text{U}(\bigoplus_\lambda S^\lambda)$ , the answer is immediate: unless  $r = s$ ,

$$\int_{\text{U}(d_1)} (U_1^{\otimes r} \otimes \bar{U}_1^{\otimes s}) d\mu_1 = \int_{\text{SU}(d_1)} \frac{1}{2\pi} \int_0^{2\pi} e^{-i(r-s)\phi} (V_1^{\otimes r} \otimes \bar{V}_1^{\otimes s}) d\phi d\nu_1 \quad (93)$$

equals zero because  $\int_0^{2\pi} e^{-i(r-s)\phi} d\phi = 0$  (cf. Lemma III.3).

When we integrate over  $\text{SU}(\bigoplus_\lambda S^\lambda)$ , setting  $r = s$  yields the same result as over  $\text{U}(\bigoplus_\lambda S^\lambda)$ . Thus counterexamples occur when  $r \neq s$ . The crucial observation to spot them is noting that each integrand, like  $V_1^{\otimes r} \otimes \bar{V}_1^{\otimes s}$ , is an element from the tensor product of the fundamental and conjugate representations of  $\text{SU}(d_1)$  and it can be further decomposed into a direct sum of irreps:

$$V_1^{\otimes r} \otimes \bar{V}_1^{\otimes s} \sim \bigoplus_\alpha W_\alpha. \quad (94)$$

Recall that we applied this observation to interpret  $T_k^\mathcal{E}$  as a truncated Fourier transform of its associated measure  $\nu$  in Section II B. On the other hand, the so-called *Schur orthogonality* [1, 3] asserts that for any compact group  $G$  with irreps  $\pi_\alpha, \pi_\beta$ ,

$$\int_G \pi_\alpha(g)_{ij} \overline{\pi_\beta(g)}_{kl} = \begin{cases} 0, & \pi_\alpha \not\cong \pi_\beta \\ \frac{1}{\dim \pi_1} \delta_{ij} \delta_{kl}, & \pi_\alpha \cong \pi_\beta \end{cases} \quad (95)$$

To apply these facts, we first expand high order tensor products like  $V_1^{\otimes r} \otimes \bar{V}_1^{\otimes s}$  by Eq.(94). Then

$$\int_{\text{SU}(d_1)} (V_1^{\otimes r} \otimes \bar{V}_1^{\otimes s}) d\nu_1 = \int_{\text{SU}(d_1)} \bigoplus_\alpha V_\alpha d\nu_1 = \bigoplus_\alpha \int_{\text{SU}(d_1)} V_\alpha \otimes \mathbf{1} d\nu_1, \quad (96)$$

where  $\mathbf{1}$  denotes the identity matrix from the trivial representation. By Schur orthogonality, the integral is nonzero, and hence leads to a counterexample, as long as the decomposition of Eq.(94) bears the trivial representation.

**Example.** As a concrete example, suppose  $d_1 \leq k, d_2 = 1$ . Let  $r = d_1$  and  $s = 0$ . Then

$$(V_1^{\otimes r} \otimes \bar{V}_1^{\otimes s}) \otimes (V_2^{\otimes k-r} \otimes \bar{V}_2^{\otimes k-s}) = V_1^{\otimes d_1} \otimes \mathbf{1}^{\otimes 2k-d_1}. \quad (97)$$

Moreover, it can be shown by the so-called *Littlewood-Richardson rule* illustrated in the following lemma that for any  $d$ , the  $d$ -fold tensor product representation of  $\text{SU}(d)$  contains the trivial representation (e.g.,  $d = 2, 3$  familiar in quantum angular momentum and quark theory). Therefore,

$$\int_{\text{SU}(d_1)} V_1^{\otimes d_1} d\nu_1 \otimes \int_{\text{SU}(1)} \mathbf{1}^{\otimes 2k-d_1} d\nu_2 \neq 0 = \int_{\text{U}(d_1)} U_1^{\otimes d_1} d\mu_1 \otimes \int_{\text{U}(1)} e^{-i(k-d_1)\phi} e^{ik\phi} d\mu_2. \quad (98)$$

Note that the 1-dimensional representation of  $\text{U}(1)$  is given by  $e^{-i\phi}$ .

This integral inconsistency truly happens in a generic  $n$ -qudit system. To explain the reason, we recite the following basic fact from  $S_n$  representation theory: *when  $n \geq 5$ , except the 1-dimensional trivial representation and sign representation, there is no irrep with dimension lower than  $n - 1$*  [2, 49, 50]. When  $n = 4$  for instance, the statement fails as there is a two dimensional irrep of Young diagram  $\lambda = (2, 2)$  (by hook length formula in Definition I.1).

It is natural to assume there are more than 5 qudits in a concerned system. Recall that by Schur-Weyl duality, only these  $S_n$  irreps corresponding to Young diagrams of size  $n$  and at most  $d$  rows appears when decomposing the system with  $\text{SU}(d)$  symmetry.

- (a) In common cases with  $d < n$ , the above counterexample cannot happen for  $k < n - 1$  because there is no  $S_n$  irrep, except the trivial one, having dimension no larger than  $k < n - 1$ . We also prove in the following lemma that it is impossible to find *any other* kinds of counterexamples in this case.
- (b) In the theoretical limit with  $d \geq n$ , the inconsistency always exists because we can select  $V_1, V_2$  from the trivial and sign representations respectively. Even they are just 1-dimensional, the phase factors are integrated independently and the integral vanishes like the RHS of Eq.(98).

**Lemma III.1.** *Let  $r \neq s \leq k < d$  with  $r, s, k, d$  being defined before. The tensor product  $V^{\otimes r} \otimes \bar{V}^{\otimes s}$  for  $V \in \text{SU}(d)$  cannot be decomposed into the trivial representation. Therefore, the integration of Eq.(94) always vanishes over  $\text{SU}(d)$ . Trivial representations only appears when  $k \geq d$ .*

*Proof.* The proof is based on the method of recording  $U(d)$  irreps by Young diagrams and results from Littlewood–Richardson Rule. We recommend the interested readers to [1, 3] for more details. For our purpose, it suffices to assume the facts:

1. the fundamental representation of  $U(d)$  is denoted by the one-box Young diagram (1).
2. the conjugate representation corresponds to the Young diagram  $(1^{d-1})$  of  $d - 1$  boxes in one column.
3. the trivial representation is given by the Young diagram  $(1^d)$  of  $d$  boxes in one column.

Other  $U(d)$  irreps are also expressed by Young diagrams under certain conditions. Especially, Littlewood–Richardson Rule says that the Young diagram of each irrep decomposed from  $U_1^{\otimes r} \otimes \bar{U}_1^{\otimes s}$  contains  $r + s(d - 1)$  boxes (but may be allocated with different rows or columns). As long as this number can be divided by  $d$ , the trivial representation (restricted back to  $SU(d)$ ) appears in the decomposition.

Thus for  $k < d$ , we consider the following two cases:

1.  $r > s$ : then  $r + s(d - 1) = (r - s) + sd$ . Since  $r, s \leq k < d$ ,  $d$  cannot divide  $r - s$ .
2.  $r < s$ : then  $r + s(d - 1) = rd + (s - r)(d - 1)$ . Assume  $d$  divides  $(s - r)(d - 1)$ . Since the greatest common divisor of  $d - 1$  and  $d$  is just 1, this requires  $s - r$  to be divided by  $d$  which is impossible.

When  $k \geq d$ , there are several ways to produce the trivial representation from tensor product as in the previous example.  $\square$

With the above argumentation, we turn to analyze the real case where matrix representations of elements from  $SU(\bigoplus_\lambda S^\lambda)$  and  $U(\bigoplus_\lambda S^\lambda)$  consist of various submatrix blocks from inequivalent  $S_n$  irreps with possible equivalent copies as

$$\bigoplus_\lambda V_\lambda^{\oplus m_{S_n, \lambda}}, \quad \bigoplus_\lambda U_\lambda^{\oplus m_{S_n, \lambda}}. \quad (99)$$

When expanding the tensor product and integrating, equivalent copies of  $V_\mu$  are obviously identical. Inequivalent sub-matrices are arranged as the preceding procedure and they are integrated independently. Then integrals of coupled fundamental and conjugate representations on one  $S_n$  sector ( $r = s$  in our previous illustration) are always the same for both  $SU(\bigoplus_\lambda S^\lambda)$  and  $U(\bigoplus_\lambda S^\lambda)$ , inconsistency may appear otherwise for  $S_n$  blocks of specific dimensions violating Lemma III.1. With Theorem II.4, we conclude that

**Theorem III.2.** *Suppose  $d < n$ . If  $k < n - 1$ , then the group  $SU(\bigoplus_\lambda S^\lambda)$  with restricted Haar measure forms an exact  $k$ -design of  $U(\bigoplus_\lambda S^\lambda)$ . Otherwise, it fails to be a  $k$ -design even in the approximate sense.*

## B. Comparison of the $k$ -fold Channels $T_k^{\text{CQA}}$ and $T_k^{\text{Haar}}$

In the last subsection, we show that  $k$ -fold order channel  $T_k^{SU} = T_k^{\text{Haar}}$  only when  $d < n$  and  $k < n - 1$ . On the other hand, the group CQA possesses the accessibility to part of phase factors due to the employment of YJM-elements (Definition I.2), which would alleviate this problem to some extent. We are now going to make this point clear. As a reminder, results from [51, 52] point out that the commutant subspace  $\text{Comm}_2(H)$  of a Lie subgroup  $H$  of any compact semisimple group  $G$  is strictly larger than  $\text{Comm}_2(G)$  and hence  $H$  can never be a unitary 2-design. However, the ambient Lie group  $U(\bigoplus_\lambda S^\lambda)$  considered here is not semisimple because they have nontrivial centers, or informally, elements with nontrivial phase factors (Theorem I.6), so the assertion is not applicable to our case.

Following the method from Section III A, we first check the integral defining  $T_k^{\text{CQA}}$  by representation theory. To begin with, we apply the main theoretical result in one related work of us [5]:

$$SU(\bigoplus_\lambda S^\lambda) \subset \text{CQA} \quad (100)$$

Thus by Theorem II.4 and III.2,

$$\text{Comm}_k(SU(\bigoplus_\lambda S^\lambda)) \supset \text{Comm}_k(\text{CQA}) \supset \text{Comm}_k(U(\bigoplus_\lambda S^\lambda)) \quad (101)$$

and CQA constitutes an exact  $k$ -design to  $U(\bigoplus_\lambda S^\lambda)$  for all  $k < n - 1$  and  $d < n$ . With nontrivial phase factors given by YJM-elements, the statement now holds for larger  $k$ . To be precise, let us consider the Lie algebra of CQA which is proved in [5] to satisfy

$$\mathfrak{L}(\text{CQA}) = \mathfrak{L}(SU(\bigoplus_\lambda S^\lambda)) \oplus \mathfrak{z}, \quad (102)$$

where  $\mathfrak{z}$  is a subspace spanned by

$$ic_\sigma = \bigoplus_\lambda i \frac{\text{tr}_\lambda(\sigma)}{\dim S^\lambda} I_\lambda = \bigoplus_\lambda i \frac{\chi_\lambda(\sigma)}{\dim S^\lambda} I_\lambda \quad (103)$$

with  $\sigma$  being any 2-cycle, 3-cycle and (2, 2)-cycle (Definition I.3). Intuitively, second order YJM-elements produce these cycles. Let  $H$  denote the integral Lie group formed by taking exponentials of elements from  $\mathfrak{z}$ , we define the map

$$f : \text{SU}(\bigoplus_\lambda S^\lambda) \times H \rightarrow \text{CQA} \text{ by } f(g, h) = gh. \quad (104)$$

Obviously,  $f$  is a Lie group homomorphism because  $\text{SU}(\bigoplus_\lambda S^\lambda)$  commute with  $H$  by definition. Then it is natural to evaluate the integral defining  $T_k^{\text{CQA}}$  using  $f$  as a "change of variables". However,  $f$  is surjective but not an isomorphism. A more familiar case is that  $\text{SU}(d) \times \text{U}(1) \not\cong \text{U}(d)$ . Even though, we still have the following lemma:

**Lemma III.3.**  $\text{Comm}_k(\text{SU}(\bigoplus_\lambda S^\lambda) \times H) = \text{Comm}_k(\text{CQA})$ . Therefore, if we denote by  $\{c_i\}$  a basis of  $\mathfrak{z}$ , then

$$\begin{aligned} T_k^{\text{CQA}} &= T_k^{\text{SU}(\bigoplus_\lambda S^\lambda) \times H} = \int_{\text{SU}(\bigoplus_\lambda S^\lambda) \times H} f(g)^{\otimes k} \otimes \overline{f(g)}^{\otimes k} d\mu(g) \\ &= \int_{\gamma_j} \int_{\text{SU}(\bigoplus_\lambda S^\lambda)} (e^{-i \sum_j \gamma_j c_j} V)^{\otimes k} \otimes (e^{i \sum_j \gamma_j c_j} \bar{V})^{\otimes k} dV d\gamma \\ &= \int_{\gamma_j} (e^{-i \sum_j \gamma_j c_j})^{\otimes k} \otimes (e^{i \sum_j \gamma_j c_j})^{\otimes k} d\gamma \int_{\text{SU}(\bigoplus_\lambda S^\lambda)} V^{\otimes k} \otimes \bar{V}^{\otimes k} dV. \end{aligned} \quad (105)$$

*Proof.* Since  $f$  defined above is a group homomorphism, it formally endows the product group  $\text{SU}(\bigoplus_\lambda S^\lambda)$  a representation on  $H = V^{\otimes n}$ , then it is legal to define  $\text{Comm}_k(\text{SU}(\bigoplus_\lambda S^\lambda) \times H)$  as the commutant of  $\text{Im} f$  which is exactly equal to  $\text{CQA} = \text{Comm}_k(\text{CQA})$ . Since we integrate with respect to the Haar measure of  $\text{SU}(\bigoplus_\lambda S^\lambda)$ ,  $T_k^{\text{SU}(\bigoplus_\lambda S^\lambda) \times H}$  is a Hermitian projector (Lemma II.3) and equals  $T_k^{\text{CQA}}$ .  $\square$

Let us recheck the example of Eq.(98) after adding YJM-elements

**Example.** Suppose  $k = n - 1$ , the expansion of  $V^{\otimes k} \otimes \bar{V}^{\otimes k}$  always contains the term  $V_1^{\otimes n-1} \otimes \mathbf{1}^{\otimes n-1}$  where  $V_1$  is an arbitrary unitary (of unit determinant) acting on the  $(n - 1)$ -dimensional  $S_n$  irrep block with  $\mathbf{1}$  being taken from the trivial irrep. Then

$$\int_{\text{SU}(n-1)} V_1^{\otimes n-1} d\nu_1 \otimes \int_{\text{SU}(1)} \mathbf{1}^{\otimes n-1} d\nu_2 \neq 0 = \int_{\text{U}(n-1)} U_1^{\otimes n-1} d\nu_1 \otimes \int_{\text{U}(1)} e^{i(n-1)\phi} d\nu_2 \quad (106)$$

by Schur orthogonality and Littlewood-Richardson rule. However, it can be seen in Eq.(105) that the integral over CQA has one more term of phase factors  $e^{-i \sum_{j=1}^N \gamma_j c_j}$  given by the Lie algebra  $\mathfrak{z}$  which would cancel the above inconsistency ultimately.

Let us integrate the phase factors provided by first order YJM-elements consisting of merely 2-cycles. As introduced in Section I A,  $c_\tau = c_{\tau'}$  for any 2-cycles  $\tau, \tau'$ . We also compute by Eq.(12) that

$$\frac{\text{tr}_{(n)}(\tau)}{\dim S^{(n)}} = 1 = -\frac{\text{tr}_{(1)}(\tau)}{\dim S^{(1^n)}}, \quad \frac{\text{tr}_{(n-1,1)}(\tau)}{\dim S^{(n-1,1)}} = \frac{n-3}{n-1} = -\frac{\text{tr}_{(2,1^{n-2})}(\tau)}{\dim S^{(2,1^{n-2})}}, \quad (107)$$

where  $\lambda = (n), (1^n), (n-1, 1), (2, 1^{n-2})$  denote the trivial, sign, fundamental and conjugate representation of  $S_n$  respectively (Definition I.1). Let  $I_\lambda$  denote the identity matrix on the  $S^\lambda$  irrep block, the phase integral accompanied with  $V_1^{\otimes n-1} \otimes \mathbf{1}^{\otimes n-1}$  includes

$$\frac{1}{2\pi} \int_0^{2\pi} \left( (e^{-i \frac{n-3}{n-1} \gamma I_{(n-1,1)}})^{\otimes n-1} \otimes (e^{i \gamma I_{(n)}})^{\otimes n-1} \right) d\gamma = \frac{1}{2\pi} \int_0^{2\pi} e^{i2\gamma} I d\gamma = 0. \quad (108)$$

**Theorem III.4.** Suppose  $n \geq 9$  and  $d < n$ . The following statement holds for exact  $k$ -design with  $\text{SU}(d)$  symmetry:

1. For an arbitrary  $n$ -qudit system, the group CQA generated by 4-local  $\text{SU}(d)$  symmetric Hamiltonians forms an exact  $k$ -design to  $\text{U}(\bigoplus_\lambda S^\lambda)$  for all  $k < \frac{1}{2}n(n-3)$ .
2. For an  $n$ -qubit system ( $d = 2$ ) with large  $n$ , CQA is an exact  $k$ -design for all  $k < n^3$ .

*Proof.* The first claims is elaborated from the previous example. Recall in Eq.(30) that any  $g \in \text{CQA}$  consists of various unitaries defined on  $S_n$  irrep sectors decomposed from the entire Hilbert space  $H$ , so we expand  $g^{\otimes k} \otimes \bar{g}^{\otimes k}$  as Eq.(89) before calculating the integral. When  $n \geq 9$ , the third minimal dimension of these irrep blocks is  $\frac{1}{2}n(n-3)$  [49] and Lemma III.1 says that the concerned integral of  $\text{SU}(S^\lambda)$  over this sub-block is always consistent with that of  $\text{U}(S^\lambda)$  when  $k \leq \frac{1}{2}n(n-3)$ . Inconsistency is seen when even lower dimensional irrep blocks get involved and we need to check that phase integral like Eq.(108) would remedy the problem.

Since we assume  $d < n$ ,  $S_n$  irreps with dimension lower than  $\frac{1}{2}n(n-3)$  are just the 1-dimensional trivial irrep and the  $(n-1)$ -dimensional fundamental irrep with its conjugate. With respect to these three irreps, let us denote by  $\phi_i, \psi_i$  with  $i = 1, 2, 3$  the phase factors of 2-cycle, 3-cycle (or  $(2, 2)$ -cycle) given by YJM-elements in CQA. As a reminder

$$\phi_1 = \psi_1 = 1, \quad \phi_2 = \frac{n-3}{n-1} = -\phi_3. \quad (109)$$

Explicit formula for  $\psi_2, \psi_3$  can be found in [18, 20]. It suffice to know that  $\psi_2 = \psi_3$  for present. By definition, they are combined as

$$\begin{aligned} & \phi_1(r_1 - s_1) + \phi_2(r_2 - s_2) + \phi_3(r_3 - s_3), \\ & \psi_1(r_1 - s_1) + \psi_2(r_2 - s_2) + \psi_3(r_3 - s_3). \end{aligned} \quad (110)$$

in a expansion of  $g^{\otimes k} \otimes \bar{g}^{\otimes k}$  with  $r_i, s_i$  being the tensor folds of the mentioned three irreps. Since  $\sum_i r_i = \sum_i s_i = k$ , we rewrite them as

$$\begin{aligned} & (\phi_1 - \phi_3)(r_1 - s_1) + (\phi_2 - \phi_3)(r_2 - s_2), \\ & (\psi_1 - \psi_3)(r_1 - s_1) + (\psi_2 - \psi_3)(r_2 - s_2). \end{aligned} \quad (111)$$

Note that  $(\psi_1 - \psi_3)(r_1 - s_1) + (\psi_2 - \psi_3)(r_2 - s_2) = (\psi_1 - \psi_3)(r_1 - s_1)$  and only when  $r_i = s_i$  for all  $i$ , they yield trivial phase. Therefore, under the assistance of phase integrals,  $T_k^{\text{CQA}} = T_k^{\text{Haar}}$  for all  $k = \frac{1}{2}n(n-3)$ . One may check the extreme case for  $d \geq m$  where the 1-dimensional sign representation adheres. Then counterexample can be found for  $k = 2(n-4)$ .

For the case of qubits, we argue by  $S_n$  character formula on two-row Young diagrams (Schur-Weyl duality) which raises the bound to  $n^3$ . Our strategy is counting the number of inequivalent irrep blocks appearing in each specific term from the expansion. For instance, there are terms bearing two and three inequivalent irreps which we rearrange as:

$$(V_1^{\otimes r} \otimes \bar{V}_1^{\otimes s} \otimes (V_2^{\otimes k-r} \otimes \bar{V}_2^{\otimes k-s}), \quad (V_1^{\otimes r_1} \otimes \bar{V}_1^{\otimes s_1} \otimes (V_2^{\otimes r_2} \otimes \bar{V}_2^{\otimes s_2}) \otimes (V_3^{\otimes k-r_1-r_2} \otimes \bar{V}_3^{\otimes k-s_1-s_2})). \quad (112)$$

The first type has been exemplified many times in the previous contexts. We still use  $\phi_1, \phi_2$  denote the phase factor induced by any 2-cycle transposition, for  $V_1, V_2$  respectively. As two-row Young diagrams ( $d = 2$  for qubits) are totally ordered, Lemma I.9 implies that  $\phi_1 \neq \phi_2$ .

As before, we examine the situation when  $r \neq s$ , because when  $r = s$ , the integrals over  $\text{U}(\bigoplus_\lambda S^\lambda)$  and  $\text{SU}(\bigoplus_\lambda S^\lambda)$  are identical (see context below Eq.(92)). For arbitrary  $k$ , the phase integral like Eq.(108) must vanish since

$$\phi_1(r-s) + \phi_2(k-r-(k-s)) = (\phi_1 - \phi_2)(r-s) \neq 0. \quad (113)$$

Therefore, any possible inconsistency between  $T_k^{\text{CQA}}$  and  $T_k^{\text{Haar}}$  should be spotted on expanded terms with at least three inequivalent irrep blocks. We tackle this case making use of the phase factors produced by  $\left(\frac{2}{n(n-1)} \sum_{l=1}^n X_l\right)^2$ . It turns out that they are just power of  $\phi_i$  given by 2-cycles (see Eq.(15)). All these phase factors are combined as

$$\begin{aligned} & (\phi_1 - \phi_3)(r_1 - s_1) + (\phi_2 - \phi_3)(r_2 - s_2), \\ & (\phi_1^2 - \phi_3^2)(r_1 - s_1) + (\phi_2^2 - \phi_3^2)(r_2 - s_2). \end{aligned} \quad (114)$$

Unless  $r_i = s_i$ , the above equations have no homogeneous solution. Therefore, counterexamples occurs with at least four inequivalent irreps emerging. Let  $d$  is the fourth lowest dimensions of these irreps. Then Lemma III.1 comes to require that  $k \geq d$ .

To derive this forth lowest dimension  $d$ , we compute by hook length formula in Definition I.1 that

$$\dim S^{(n-2,2)} = \frac{n(n-3)}{2}, \quad \dim S^{(n-3,3)} = \frac{n(n-1)(n-5)}{6}, \quad \dim S^{(n-4,4)} = \frac{n(n-1)(n-2)(n-7)}{24}. \quad (115)$$

For  $S_n$  irreps of two-row Young diagrams, their dimensions also satisfy the following identity (see the end of Section I A)

$$\dim S^{(n-r,r)} = \binom{n}{r} - \binom{n}{r-1} \quad (116)$$

with  $0 \leq r \leq \lfloor n/2 \rfloor$  and  $\binom{n}{-1} = 0$  by convention. For  $r > 4$ ,

$$\binom{n}{r} - \binom{n}{r-1} = \frac{n-2r+1}{n-r+1} \binom{n}{r} \geq \frac{1}{n+1} \binom{n}{r}. \quad (117)$$

Since the binomial coefficients are increasing when  $r \leq \lfloor n/2 \rfloor$ , for large  $n$  the fourth lowest dimensions among these irreps is lower bounded by  $n^3$ , which finishes the proof.  $\square$

*Remark.* We introduce one related result proved in [28, 29, 53, 54]: the group

$$\text{eSWAP} = \langle e^{-i\theta_{rs}(r,s)} \rangle \quad (118)$$

generated by all  $\frac{1}{2}n(n-1)$  transpositions contains  $SU(\bigoplus_{\lambda} S^{\lambda})$  on qubits ( $d=2$ ).

- (a) Since eSWAP contains 2-cycles, technique from the above theorem can be applied to show that eSWAP forms an exact  $k$ -design for all  $k < n^2$  on an  $n$ -qubit system.
- (b) To achieve the restricted universality on  $SU(\bigoplus_{\lambda} S^{\lambda})$ , transpositions  $(i, j)$  acting on arbitrary qubits from the system are used. However, to approximate unitary  $k$ -design with  $k < n^2$ , we show in Section IV A that the ensemble  $\mathcal{E}_{\text{SWAP}}$  consisting of merely nearest-neighbor SWAPs  $(i, i+1)$  are sufficient.

Note that the restricted universality or  $k$ -design fails to hold on eSWAP when  $d \geq 3$  with rigorous verification from [28–30, 53, 54], we also provide an explicit numerical evidence by integrating expansions of  $k$ -fold channels (likes Eq.(112)) on a certain  $S_n$  irreps.

As a reminder, it is still possible to refine the bound on  $k$  provided above: we use phase factors given by the square of sum of all YJM-elements  $(\sum_{l=1}^n X_l)^2$ , but there are still other kinds of second-order YJM-elements  $X_k X_l$  and the lower bound on  $S_n$  irreps could be modified. However, this requires a more sophisticated treatment to compute  $S_n$  characters and estimate the hook length formula. Both of which are deep inside combinatorics and representation theory [18–20, 23, 49, 55], and out the scope of this paper. More importantly, we prove in the next subsection that any ensemble with a bounded locality on its unitaries would finally cease to be an exact  $k$ -design for large  $k$ . Being different from the common case with no concerning on the symmetry, it is now impossible to achieve the arbitrary large  $k$ -design, simply by local unitaries.

### C. Circuit Locality for Universality and Unitary $k$ -design with $SU(d)$ Symmetry

For practical reason, implementation with local gates is desirable for most quantum computation problems. It is well-known that 2-local unitaries are universal to generate any quantum circuits for both qubits and qudits [25] as well as in forming approximate  $k$ -design [26, 27, 34]. Under  $SU(d)$  symmetry, the group CQA consisting of 4-local generators are found to be universal when ignoring relative phase factors [5] and proved to be  $SU(d)$ -symmetric exact  $k$ -design for  $k = \Omega(n^2)$ . We now explore the situation for arbitrary large  $k$  where we have to replenish even more phase factors and operators with a bounded locality can never fulfill this task finally.

To begin with, we first discuss the locality needed to achieve universality with all phase factors being taken into account, i.e., generating  $U(\bigoplus_{\lambda} S^{\lambda})$  rather than  $SU(\bigoplus_{\lambda} S^{\lambda})$ . This question has been addressed in [53, 54] for qubits as a "no-go" theorem. We prove the case for general qudits by  $S_n$  representation theory as a preparation to describe the main result on  $k$ -design. Recall that the number of  $S_n$  irreps corresponding to Young diagrams with at most  $d$  rows is given by the partition function  $p(n, d)$  in Definition I.4. Any *finite or infinite* set  $S$  of  $N$ -local  $SU(d)$  symmetric unitaries on an  $n$ -qudit system is said to be *exactly universal* if  $\langle S \rangle$  is itself a Lie group equal to  $U(\bigoplus_{\lambda} S^{\lambda})$ . It is *approximately universal* if  $\overline{\langle S \rangle} = U(\bigoplus_{\lambda} S^{\lambda})$ .

**Theorem III.5.** *In either exact or approximate sense, the locality  $N$  of unitaries from  $S$  is at least  $\Omega(\log p(n, d))$ .*

*Proof.* We first consider exact universality. Let  $\mathcal{V}_N$  be the group generated by all  $N \geq 4$   $SU(d)$  symmetric unitaries. It is shown in [30, 53, 54] that the Lie algebra of this group is spanned by arbitrary complex linear combination  $H = \sum_i c_i \sigma_i$  of permutations  $\sigma_i$  supported on  $N$  qudits as long as the combination is anti-Hermitian. Then  $H = (H - c_H) + c_H$  with

$$c_H = \bigoplus_{\lambda} \frac{\text{tr}_{\lambda} H}{\dim S^{\lambda}} I_{\lambda} \quad (119)$$

being defined by trace of  $H$  in each irrep block  $S^{\lambda}$  ( $S_n$  characters) with multiplicities (cf. Eq.(103)). Since  $H$  is anti-Hermitian,  $\text{tr}_{\lambda} H$  must be a real linear combination of  $\text{tr}_{\lambda} \sigma$  times the imaginary unit.



The group  $\mathcal{V}_N$  contains CQA by definition and hence its Lie algebra can be written as [5]:

$$\mathfrak{L}(\text{SU}(\bigoplus_{\lambda} S^{\lambda})) \oplus \mathfrak{z}_N, \quad (120)$$

where  $\mathfrak{z}_N$  is spanned by  $ic_{\sigma}$  for all  $N$ -local  $\sigma$ . As introduced in Section I A,  $c_{\sigma} = c_{\sigma'}$  for  $\sigma, \sigma'$  of the same cycle type (see Definition I.3) and they act as a scalar matrix in any equivalent  $S_n$  irrep. Let us record these scalars in the following matrix:

$$C_n = \begin{pmatrix} c_{11} & \cdots & c_{1p(n)} \\ \vdots & \ddots & \vdots \\ c_{p(n)1} & \cdots & c_{p(n)p(n)} \end{pmatrix}, \quad (121)$$

where the column indices labels inequivalent irreps and row indices represent different cycle type because the number of inequivalent irreps equals the number  $p(n)$  of partitions of  $m$ , which is also the number of different cycle types. The key point to prove our statement is realizing that the above matrix is invertible, or equivalently, the column vectors form a basis for phase factors from inequivalent  $S_n$  irreps: recall in Theorem I.6, we present three different center bases for phase factors and one used here is just a rescale of  $c_{\lambda}$  by the number of all permutations  $\sigma$  of the given cycle type  $\lambda$ . In the real case when we only have  $N$ -local permutations,  $\mathfrak{z}_N$  defined above is spanned by the first  $p(N)$  column vectors of  $C_n$ .

On the other hand, Schur-Weyl duality says that only  $S_n$  irreps corresponding to Young diagrams with no more than  $d$  rows can be found in the qudits system. Therefore, the Lie algebra of  $U(\bigoplus_{\lambda} S^{\lambda})$  is spanned by  $\mathfrak{L}(\text{SU}(\bigoplus_{\lambda} S^{\lambda}))$  with column vectors from a certain invertible  $p(n, d) \times p(n, d)$  submatrix from  $C_n$ , but there is in general no way to locate this submatrix as computing the entries  $c_{ij}$  of  $C_n$  requires evaluating  $S_n$  characters and computing  $p(n, d)$  in precise is also formidable. Even though, there is the following simple necessary condition for  $\mathcal{V}_N$  to be universal:

$$p(N) \geq p(n, d) \implies N = \Omega(\log p(n, d)), \quad (122)$$

where we use the exponential lower bound on  $p(N)$  given below Definition I.4. When  $d = 2$ , the required locality is at least  $\log n$  (Theorem III.7 in the subsequent section has a precise bound for qubits). In the extreme case when  $d \geq n$  however, reconstructing  $U(\bigoplus_{\lambda} S^{\lambda})$  demands  $\sigma$  of any cycle type, including gates permuting all qudits.

To deal with approximate universality, assume the locality  $N$  of a (finite or infinite) generating set  $S$  is less than  $\Omega(\log p(n, d))$ . Since  $\mathcal{V}_N$  is a compact subgroup and since  $S \subset \mathcal{V}_N$ ,

$$\overline{\langle S \rangle} \subset \mathcal{V}_N \subsetneq U(\bigoplus_{\lambda} S^{\lambda}), \quad (123)$$

which leads to a contradiction.  $\square$

We now prove main result on the locality of exact  $k$ -design for arbitrary large  $k$ .

**Theorem III.6.** *Given any finite or infinite  $SU(d)$  symmetric ensemble  $\mathcal{E}$  on qudits, if it forms an exact/approximate  $k$ -design to  $U(\bigoplus_{\lambda} S^{\lambda})$  for  $k \rightarrow \infty$ , then the locality of the ensemble is at least  $\Omega(\log p(n, d))$ .*

*Proof.* Simialr to the previous proof, we first assume that  $\mathcal{E} = \mathcal{V}_N$  with  $N \geq 4$  and then we decompose its Lie algebra into  $\mathfrak{L}(\text{SU}(\bigoplus_{\lambda} S^{\lambda})) \oplus \mathfrak{z}_N$ . By Lemma III.3, we compute  $T_k^{\mathcal{V}_N}$  by

$$\begin{aligned} & \int_{\gamma_j} \int_{\text{SU}(\bigoplus_{\lambda} S^{\lambda})} (e^{-i \sum_j \gamma_j c_j} V)^{\otimes k} \otimes (e^{i \sum_j \gamma_j c_j} \bar{V})^{\otimes k} dV d\gamma \\ &= \int_{\gamma_j} (e^{-i \sum_j \gamma_j c_j})^{\otimes k} \otimes (e^{i \sum_j \gamma_j c_j})^{\otimes k} d\gamma \int_{\text{SU}(\bigoplus_{\lambda} S^{\lambda})} V^{\otimes k} \otimes \bar{V}^{\otimes k} dV, \end{aligned} \quad (124)$$

where  $c_i$  can be seen as the column vectors  $(c_{ij})$  from Eq.(121). To analyze the above integral, we first expand  $V^{\otimes k} \otimes \bar{V}^{\otimes k}$  with respect to  $S_n$  irrep blocks and then apply Littlewood-Richardson rule and Schur orthogonality as we did in Section III A: let

$$(r_1, \dots, r_{p(n, d)}, s_1, \dots, s_{p(n, d)}) \quad (125)$$

denote the tensor product orders of unitaries  $V_i$  and  $\bar{V}_i$  on the block  $S^{\lambda_i}$  expanded from  $V^{\otimes k} \otimes \bar{V}^{\otimes k}$ , so  $\sum_i r_i = \sum_i s_i = k$  and  $r_i, s_i$  are non-negative. Then the following conditions is asked by Lemma III.1:

$$d_i |r_i - s_i| \text{ for all } i, \text{ and } r_{i_0} \neq s_{i_0} \quad (126)$$



for at least one  $i_0$ . As discussed in Section III A integral of these tensor product orders is nonzero over  $SU(\bigoplus_\lambda S^\lambda)$  but vanishes over  $U(\bigoplus_\lambda S^\lambda)$ .

Then we turn to show that the phase integral involving  $e^{-i \sum_j \gamma_j c_j}$  is also nonzero for large  $k$  which implies that  $T_k^{\mathcal{V}_N} = T_k^{\text{Haar}}$ . By definition, multiplying with the tensor product orders  $r_i, s_i$ , these phases are combined as the following matrix product

$$(r_1 - s_1, r_2 - s_2, \dots, r_{p(n,d)} - s_{p(n,d)}) \begin{pmatrix} c_{11} & \cdots & c_{1p(N)} \\ c_{21} & \cdots & c_{2p(N)} \\ \vdots & & \vdots \\ c_{p(n,d)1} & \cdots & c_{p(n,d)p(N)} \end{pmatrix} \quad (127)$$

If each combined coefficient is zero, taking exponential only yields the identity matrix and the phase integral ends up to be nonzero. Since  $\sum_i r_i - \sum_i s_i = 0$ , this situation happens if we can find a *nontrivial integral solution* to the following linear system:

$$(x_1, x_2, \dots, x_{p(n,d)}) \begin{pmatrix} 1 & c_{11} & \cdots & c_{1p(N)} \\ 1 & c_{21} & \cdots & c_{2p(N)} \\ \vdots & \vdots & & \vdots \\ 1 & c_{p(n,d)1} & \cdots & c_{p(n,d)p(N)} \end{pmatrix} = 0. \quad (128)$$

By Proposition I.7,  $c_{ij}$  are rational number and then by Gaussian elimination procedure, such a solution always exists when  $p(N) < p(n,d) - 1$ . Let

$$r_i = \begin{cases} d_1 \cdots d_{p(n,d)} \cdot x_i, & x_i > 0 \\ 0, & x_i \leq 0 \end{cases}, \quad s_i = \begin{cases} 0, & x_i > 0 \\ -d_1 \cdots d_{p(n,d)} \cdot x_i, & x_i \leq 0 \end{cases} \quad (129)$$

It satisfies all the above conditions from Eq.(126) with  $k \geq d_1 \cdots d_{p(n,d)}$  and  $T_k^{\mathcal{V}_N} \neq T_k^{\text{Haar}}$ .

Given a generic  $SU(d)$ -symmetric ensemble  $\mathcal{E}$  of  $N$ -local unitaries, it must be contained in  $\mathcal{V}_N$  by definition. Analogous to the proof made in Proposition II.7, any  $M \in \text{Comm}_k(\mathcal{V}_N)$  is a unit eigenvector of  $T_k^{\mathcal{E}\dagger} T_k^{\mathcal{E}}$ , no matter  $T_k^{\mathcal{E}}$  is Hermitian or not. This further indicates that

$$F_{(k)}^{\mathcal{E}} = \text{tr}(T_k^{\mathcal{E}\dagger} T_k^{\mathcal{E}}) \geq \text{tr}(T_k^{\mathcal{V}_N}) = F_{(k)}^{\mathcal{V}_N}. \quad (130)$$

Therefore, if  $\mathcal{E}$  forms an  $\epsilon$ -approximate  $k$ -design for arbitrary  $k$  in the sense of (63),  $\mathcal{V}_N$  will also do, which forces the locality  $N$  to be  $\Omega(\log p(m, d))$ .  $\square$

#### D. High Order CQA Group for Arbitrary Unitary Design with $SU(d)$ Symmetry

This subsection is a theoretical description on how to achieve  $k$ -design for arbitrary  $k$  at the price of increasing operator locality. As clarified in the previous context,  $\text{CQA} \supset SU(\bigoplus_\lambda S^\lambda)$ . Even though, there are still independent relative phase factors which cannot be manipulated through CQA or  $SU(\bigoplus_\lambda S^\lambda)$  and thus prevent these two subgroups being universal or  $k$ -design for arbitrary  $k$ . To replenish phase factors, a direct implementation of  $\Pi_\mu := \frac{1}{n!} \sum_{\sigma \in S_n} \chi_\mu(\sigma) \sigma$  introduced in Theorem I.6 demands  $n!$  permutations from  $S_n$  and is thus infeasible. Simply adding  $\sigma \in S_n$  with high locality produces  $c_\sigma$  defined in Eq.(103) as phase factors. However, as explained in Theorem III.4 and III.5, there is still a huge obstacle in determining whether  $\{c_\sigma\}$  spans the necessary independent phases from the system. Therefore, we turn to use YJM-elements.

Let us first consider the case when  $d = 2$  on qubits where we apply the technique of summing YJM-elements introduced in Section I A. Except Jucys-Murphy theorem (Theorem I.6), we can construct a more simple basis for the center of  $\mathbb{C}[S_n]$  by YJM-elements on any  $n$ -qubit system with only two-row Young diagrams.

**Theorem III.7.** *Let us consider  $P_l = (\sum_{i=1}^n X_i)^l$ . The set  $\{P_l\}$  with  $l = 0, \dots, \lfloor \frac{n}{2} \rfloor$  constitutes a basis of the center of  $\mathbb{C}[S_n]$  restricted to the permutation representation on  $n$ -qubit system with two-row Young diagrams.*

*Proof.* The reason that we set  $l = 0, \dots, \lfloor \frac{n}{2} \rfloor$  is that there are  $p(n, 2) = \lfloor \frac{n}{2} \rfloor + 1$  different two-row Young diagrams or inequivalent irreps decomposed from an  $n$ -qubit system (see Definition I.4). Accordingly, a center basis consists of  $p(n, 2)$  basis elements as mentioned in Theorem III.5. The most natural basis elements for the center are orthonormal projections:

$$\Pi_\lambda = \frac{\dim S^\lambda}{n!} \sum_{g \in S_n} \bar{\chi}_\lambda(g) \rho_\lambda(\sigma) \quad (131)$$

defined in Theorem I.6 by  $S_n$  characters. However, it is unclear how to efficiently encode them into a quantum circuit because we need summing over the symmetric group with  $n!$  elements.

By Eq.(15) and (16), we have

$$P_l = \sum_{i=0}^{\lfloor n/2 \rfloor} (\alpha_\lambda)^i \Pi_{\lambda_i}, \quad (132)$$

where  $\alpha_\lambda$  is the sum of all components of content vectors of  $\lambda$ . Then we consider the following *Vandermonde matrix*:

$$V(\alpha_{\lambda_i}) = \begin{pmatrix} 1 & 1 & \cdots & 1 \\ \alpha_{\lambda_0} & \alpha_{\lambda_1} & \cdots & \alpha_{\lambda_{\lfloor n/2 \rfloor}} \\ \vdots & \vdots & \ddots & \vdots \\ \alpha_{\lambda_0}^{\lfloor n/2 \rfloor} & \alpha_{\lambda_1}^{\lfloor n/2 \rfloor} & \cdots & \alpha_{\lambda_{\lfloor n/2 \rfloor}}^{\lfloor n/2 \rfloor} \end{pmatrix} \quad (133)$$

It can be easily seen that the row entries of  $V(\alpha_{\lambda_i})$  are just coefficients of the linear expansion in Eq.(132). In the language of linear algebra, the matrix  $V(\alpha_{\lambda_i})$  transforms  $\{\Pi_{\lambda_i}\}$  to  $\{P_l\}$ .

There is no doubt that  $\{\Pi_{\lambda_i}\}$  is a basis. If the transformation  $V(\alpha_{\lambda_i})$  is invertible,  $\{P_l\}$  is also qualified as a basis. The invertibility of  $V(\alpha_{\lambda_i})$  is revealed by its determinant which equals

$$V(\alpha_{\lambda_i}) = (-1)^{((\lfloor n/2 \rfloor + 1))((\lfloor n/2 \rfloor)) / 2} \Pi_{s < t} (\alpha_{\lambda_s} - \alpha_{\lambda_t}). \quad (134)$$

Since we concern only two-row Young diagram at present, Lemma I.9 says that the dominance relation in Definition I.8 is totally ordered and hence,  $\alpha_{\lambda_s} - \alpha_{\lambda_t} \neq 0$  as long as  $\lambda_s \neq \lambda_t$ . Therefore the Vandermonde matrix is invertible, which confirms the statement.  $\square$

The trick of using Vandermonde matrix is also used as a crucial step [5] to identify that the Lie algebra of CQA contains that of  $SU(\bigoplus_\lambda S^\lambda)$ . In proving Theorem III.5, we mentioned that it is generally unclear how to determine a  $p(n, d) \times p(n, d)$  invertible submatrix from Eq.(121) constituting a center basis on a generic qudits system. When  $d = 2$ , with the above technique involving properties of YJM-elements and content vectors, we know that all cycles generated by YJM-elements up to  $\lfloor n/2 \rfloor$ th order are indispensable. Consequently, the largest required locality on generators is  $2\lfloor n/2 \rfloor$  and hence

**Corollary III.8.** *On an  $n$ -qubit system, any  $SU(d)$  symmetric universal generating set  $S$  needs unitaries acting on all qubits when  $n$  is being even, on  $n - 1$  qubits when  $n$  is odd.*

There is a method proposed in [53] using ancilla qubits, which helps to restore the locality for  $SU(d)$  symmetric universality. The case on general qudits is still unknown due to the difficulties to find the aforementioned  $p(n, d) \times p(n, d)$  invertible submatrix. Instead of the universality, our focus in this paper is the unitary  $k$  design under  $SU(d)$  symmetry. We now prove that  $T_k^{\text{CQA}^{(k)}} = T_k^{\text{Haar}}$  with  $k$ th order YJM-elements. Recall that in Section III B, we verified that

$$\begin{aligned} T_k^{\text{CQA}} &= \int_{\gamma_j} \int_{SU(\bigoplus_\lambda S^\lambda)} (e^{-i \sum_j \gamma_j c_j} V)^{\otimes k} \otimes (e^{i \sum_j \gamma_j c_j} \bar{V})^{\otimes k} dV d\gamma \\ &= \int_{\gamma_j} (e^{-i \sum_j \gamma_j c_j})^{\otimes k} \otimes (e^{i \sum_j \gamma_j c_j})^{\otimes k} d\gamma \int_{SU(\bigoplus_\lambda S^\lambda)} V^{\otimes k} \otimes \bar{V}^{\otimes k} dV. \end{aligned} \quad (135)$$

Rewriting the phase integral under basis  $\{P_l\}$ , we obtain

$$\bigoplus_{\lambda_1, \dots, \lambda_k, \mu_1, \dots, \mu_k} \int_0^{2\pi} d\gamma_0 \cdots d\gamma_k \bigotimes_{i=1, \dots, k} e^{-i(\sum_l \gamma_l \alpha_{\lambda_i}^l) I_{\lambda_i}} \bigotimes_{j=1, \dots, k} e^{i(\sum_l \gamma_l \alpha_{\mu_j}^l) I_{\mu_j}}. \quad (136)$$

We illustrated in previous subsections that the integrals expanded from  $T_k^{\text{Haar}}$  vanish unless  $\{\lambda_1, \dots, \lambda_k\} = \{\mu_1, \dots, \mu_k\}$ . Note that the equality on sets contains the situations with equivalent copies of any  $\lambda_i, \mu_j$  and any reordering on these irreps when taking tensor products. To show  $T_k^{\text{CQA}^{(k)}} = T_k^{\text{Haar}}$ , we simply check the phase integral by now (cf. Theorem III.6). The above expansion on each variable  $\gamma_l$  reads  $(\alpha_{\mu_0}^l + \cdots + \alpha_{\mu_k}^l) - (\alpha_{\lambda_0}^l + \cdots + \alpha_{\lambda_k}^l)$ . The total integral will vanish if there exists some  $l > 0$  such that the difference is nonzero (it equals zero for  $\gamma_0$  since  $l = 0$ ). To inspect the situation, let us consider the following linear equations for any given integers  $p_1, \dots, p_k$ :

$$\begin{aligned} \alpha_0 + \alpha_1 + \cdots + \alpha_k &= p_1, \\ \alpha_0^2 + \alpha_1^2 + \cdots + \alpha_k^2 &= p_2, \\ &\vdots \\ \alpha_0^k + \alpha_1^k + \cdots + \alpha_k^k &= p_k. \end{aligned} \quad (137)$$

As encountered in Section IID, it is known as the *moment problem* and using basic algebraic geometry [47], we know that Eq. (137) admits, up to permutation, a unique solution  $\{\alpha_l\}$ . Since  $\alpha_\lambda \neq \alpha_\mu$  for distinct two-row Young diagrams  $\lambda, \mu$  by Lemma I.9, this unique solution must correspond to a particular set of Young diagrams and we can conclude with the following theorem:

**Theorem III.9.** *For any  $k$ , the  $k$ th order CQA $^{(k)}$  forms  $SU(2)$ -symmetric exact  $k$ -design. Since CQA becomes universal with  $\lfloor n/2 \rfloor$  order YJM-elements, CQA $^{(\lfloor n/2 \rfloor)}$  forms  $SU(2)$ -symmetric exact  $k$ -design for arbitrary large  $k$ .*

Note that the above analysis only remains true for qubits, as even in the case of qutrits  $d = 3$ , the dominance relation ceases to be a total ordering and there are lots of examples violating the central condition  $\alpha_\lambda \neq \alpha_\mu$  for  $\lambda \neq \mu$  used in the preceding proofs. Even though, we are still able to generalize the result to arbitrary qudits making use of YJM-elements and Okounkov-Vershik approach [9] to compare  $\text{Comm}_k(\text{CQA})$  and  $\text{Comm}_k(\text{U}(\bigoplus_\lambda S^\lambda))$  introduced in Section IA and II. As a motivation, we first consider the following example.

**Example.** Let us examine that CQA forms 1-design in a different way from Theorem III.4. By definition, CQA contains the YJM-elements  $X_i$ . As the main result in [9], Okounkov and Vershik successfully verified that YJM-elements  $X_i \in \mathbb{C}[S_n]$  generate so-called *Gelfand-Tsetlin subalgebra*  $\text{GZ}_n \subset \mathbb{C}[S_n]$ . To put it in a more elementary way, let us consider the direct sum of all inequivalent  $S_n$  irreps. Then finite linear combinations and products of the matrix representations of  $X_i$ , e.g., Eq.(4), yields arbitrary diagonal matrices on the representation space. This claim is stronger than Theorem I.6 where phases matrices are constant scalars in each  $S_n$  irrep block.

Then our proof follows: for any  $M \in \text{Comm}_1(\text{CQA})$ . It commutes with any group elements from  $SU(\bigoplus_\lambda S^\lambda)$ . More importantly, it commutes with any YJM-elements which forces it to commute with arbitrary diagonal matrix including those phase matrices. Therefore,  $\text{Comm}_1(\text{CQA}) = \text{Comm}_1(\text{U}(\bigoplus_\lambda S^\lambda))$ .

With the same assumption, let us check what happens for  $k = 2$ , since

$$M \cdot (\exp(-itX_j))^{\otimes 2} = (\exp(-itX_j))^{\otimes 2} \cdot M \quad (138)$$

for arbitrary  $j = 1, \dots, n$  and  $t \in \mathbb{R}$ , taking derivatives we obtain

$$[M, X_j \otimes I + I \otimes X_j] = 0, \quad (139)$$

where  $[\cdot, \cdot]$  is the Lie bracket. The necessary condition presented above for  $M \in \text{Comm}_1(\text{U}(\bigoplus_\lambda S^\lambda))$  now converts to:

$$[M, D \otimes I + I \otimes D] = 0, \quad (140)$$

where  $D$  is an arbitrary diagonal matrix. Unfortunately, there is no guarantee that finite linear combinations and products of  $\{X_j \otimes I + I \otimes X_j\}$  produces  $D \otimes I + I \otimes D$ . For instance,

$$(X_i \otimes I + I \otimes X_i) \cdot (X_j \otimes I + I \otimes X_j) = (X_i X_j) \otimes I + I \otimes (X_i X_j) + X_i \otimes X_j + X_j \otimes X_i \quad (141)$$

contains undesired terms like  $X_i \otimes X_j + X_j \otimes X_i$ . Lemma III.10 proved in the following claims that adding second order YJM-elements fixes this problem and generalizes to arbitrary  $k > 1$ .

**Lemma III.10.** *Let us consider the tensor product representation on  $H^{\otimes k}$  of an  $n$ -qudit system  $H = V^{\otimes n}$ . Taking all matrix representations of  $X_{i_1} \cdots X_{i_s}$  for  $1 \leq i_1, \dots, i_s \leq n$  and  $s \leq k$ :*

$$(X_{i_1} \cdots X_{i_s}) \otimes I \otimes \cdots \otimes I + I \otimes (X_{i_1} \cdots X_{i_s}) \otimes \cdots \otimes I + I \otimes I \otimes \cdots \otimes (X_{i_1} \cdots X_{i_s}) \quad (142)$$

*is sufficient to generate  $D \otimes I \otimes \cdots \otimes I + I \otimes D \otimes \cdots \otimes I + I \otimes I \otimes \cdots \otimes D$  for arbitrary diagonal matrix  $D$  on the representation space.*

*Proof.* With the notation from representation theory, let

$$\rho(X_{i_1} \cdots X_{i_r}) := (X_{i_1} \cdots X_{i_r}) \otimes I \otimes \cdots \otimes I + I \otimes (X_{i_1} \cdots X_{i_r}) \otimes \cdots \otimes I + I \otimes I \otimes \cdots \otimes (X_{i_1} \cdots X_{i_r}), \quad (143)$$

where  $\rho$  is actually the  $k$ -fold tensor product representation of the Lie algebra  $\mathfrak{gl}(H)$ . We also denote by  $(X_{i_1} \cdots X_{i_r})^\alpha, \alpha = 1, 2, \dots, k$  the single term

$$I \otimes \cdots \otimes I \otimes (X_{i_1} \cdots X_{i_r}) \otimes I \cdots \otimes I \quad (144)$$

with  $X_{i_1} \cdots X_{i_r}$  be located at the  $\alpha$ th tensor product.

When  $k = 1$ , obviously,

$$\rho(X_{i_1} \cdots X_{i_r}) = \rho(X_{i_1} \cdots X_{i_{r-2}} X_{i_{r-1}}) \rho(X_{i_r}). \quad (145)$$

When  $k = 2$ , it is straightforward to check that

$$\begin{aligned} 2\rho(X_{i_1} \cdots X_{i_r}) &= \rho(X_{i_1} \cdots X_{i_{r-2}} X_{i_{r-1}}) \rho(X_{i_r}) + \rho(X_{i_1} \cdots X_{i_{r-2}} X_{i_r}) \rho(X_{i_{r-1}}) \\ &\quad + \rho(X_{i_1} \cdots X_{i_{r-2}}) \rho(X_{i_{r-1}} X_{i_r}) - \rho(X_{i_1} \cdots X_{i_{r-2}}) \rho(X_{i_{r-1}}) \rho(X_{i_r}). \end{aligned} \quad (146)$$

Thus we argue by induction that as long as we employ all first and second order YJM elements,  $\rho(X_{i_1} \cdots X_{i_r})$  for arbitrary  $r > 2$  can be generated.

When  $k = 3$ , we first rewrite Eq.(146) on  $H^{\otimes 3}$  for  $r = 1$ :

$$\begin{aligned} 2\rho(X_{i_1} \cdots X_{i_{r-1}}) &= \rho(X_{i_1} \cdots X_{i_{r-3}} X_{i_{r-2}}) \rho(X_{i_{r-1}}) + \rho(X_{i_1} \cdots X_{i_{r-3}} X_{i_{r-1}}) \rho(X_{i_{r-2}}) \\ &\quad + \rho(X_{i_1} \cdots X_{i_{r-3}}) \rho(X_{i_{r-2}} X_{i_{r-1}}) - \rho(X_{i_1} \cdots X_{i_{r-3}}) \rho(X_{i_{r-2}}) \rho(X_{i_{r-1}}) \\ &\quad + \sum_{\alpha \neq \beta \neq \gamma} (X_{i_1} \cdots X_{i_{r-3}})^\alpha (X_{i_{r-2}})^\beta (X_{i_{r-1}})^\gamma. \end{aligned} \quad (147)$$

The last term emerges because tensor products with three nontrivial components are allowed in  $H^{\otimes 3}$ . Multiplying both sides with  $\rho(X_{i_r})$  and noting that

$$\begin{aligned} &\sum_{\alpha \neq \beta \neq \gamma} (X_{i_1} \cdots X_{i_{r-3}})^\alpha (X_{i_{r-2}})^\beta (X_{i_{r-1}})^\gamma \rho(X_{i_r}) \\ &= \sum_{\alpha \neq \beta \neq \gamma} \left( (X_{i_1} \cdots X_{i_{r-3}} X_{i_r})^\alpha (X_{i_{r-2}})^\beta (X_{i_{r-1}})^\gamma + (X_{i_1} \cdots X_{i_{r-3}})^\alpha (X_{i_{r-2}} X_{i_r})^\beta (X_{i_{r-1}})^\gamma \right. \\ &\quad \left. + (X_{i_1} \cdots X_{i_{r-3}})^\alpha (X_{i_{r-2}})^\beta (X_{i_{r-1}} X_{i_r})^\gamma \right), \end{aligned} \quad (148)$$

we have

$$\begin{aligned} &\rho(X_{i_1} \cdots X_{i_{r-3}}) \rho(X_{i_{r-2}}) \rho(X_{i_{r-1}}) \rho(X_{i_r}) \\ &= \sum_{\alpha \neq \beta \neq \gamma} \left( (X_{i_1} \cdots X_{i_{r-3}} X_{i_r})^\alpha (X_{i_{r-2}})^\beta (X_{i_{r-1}})^\gamma + (X_{i_1} \cdots X_{i_{r-3}})^\alpha (X_{i_{r-2}} X_{i_r})^\beta (X_{i_{r-1}})^\gamma \right. \\ &\quad \left. + (X_{i_1} \cdots X_{i_{r-3}})^\alpha (X_{i_{r-2}})^\beta (X_{i_{r-1}} X_{i_r})^\gamma \right) \\ &\quad + \rho(X_{i_1} \cdots X_{i_{r-3}} X_{i_{r-2}}) \rho(X_{i_{r-1}}) \rho(X_{i_r}) + \rho(X_{i_1} \cdots X_{i_{r-3}} X_{i_{r-1}}) \rho(X_{i_{r-2}}) \rho(X_{i_r}) \\ &\quad + \rho(X_{i_1} \cdots X_{i_{r-3}}) \rho(X_{i_{r-2}} X_{i_{r-1}}) \rho(X_{i_r}) \\ &\quad - 2\rho(X_{i_1} \cdots X_{i_{r-1}}) \rho(X_{i_r}). \end{aligned} \quad (149)$$

Again, we rewrite (146) on  $H^{\otimes 3}$ , but for  $\rho(X_{i_1} \cdots X_{i_{r-3}} X_{i_r}) \rho(X_{i_{r-2}}) \rho(X_{i_{r-1}})$ :

$$\begin{aligned} 2\rho(X_{i_1} \cdots X_{i_r}) &= \rho(X_{i_1} \cdots X_{i_{r-3}} X_{i_{r-2}} X_{i_r}) \rho(X_{i_{r-1}}) + \rho(X_{i_1} \cdots X_{i_{r-3}} X_{i_{r-1}} X_{i_r}) \rho(X_{i_{r-2}}) \\ &\quad + \rho(X_{i_1} \cdots X_{i_{r-3}} X_{i_r}) \rho(X_{i_{r-2}} X_{i_{r-1}}) - \rho(X_{i_1} \cdots X_{i_{r-3}} X_{i_r}) \rho(X_{i_{r-2}}) \rho(X_{i_{r-1}}) \\ &\quad + \sum_{\alpha \neq \beta \neq \gamma} (X_{i_1} \cdots X_{i_{r-3}} X_{i_r})^\alpha (X_{i_{r-2}})^\beta (X_{i_{r-1}})^\gamma. \end{aligned} \quad (150)$$

Recall that YJM-elements commute with each other, so there is no difference between the LHS term from above and that from Eq.(146). Similarly,

$$\begin{aligned} 2\rho(X_{i_1} \cdots X_{i_r}) &= \rho(X_{i_1} \cdots X_{i_{r-3}} X_{i_{r-2}} X_{i_r}) \rho(X_{i_{r-1}}) + \rho(X_{i_1} \cdots X_{i_{r-3}} X_{i_{r-1}}) \rho(X_{i_{r-2}} X_{i_r}) \\ &\quad + \rho(X_{i_1} \cdots X_{i_{r-3}}) \rho(X_{i_{r-2}} X_{i_{r-1}} X_{i_r}) - \rho(X_{i_1} \cdots X_{i_{r-3}}) \rho(X_{i_{r-2}} X_{i_r}) \rho(X_{i_{r-1}}) \\ &\quad + \sum_{\alpha \neq \beta \neq \gamma} (X_{i_1} \cdots X_{i_{r-3}})^\alpha (X_{i_{r-2}} X_{i_r})^\beta (X_{i_{r-1}})^\gamma, \\ 2\rho(X_{i_1} \cdots X_{i_r}) &= \rho(X_{i_1} \cdots X_{i_{r-3}} X_{i_{r-1}} X_{i_r}) \rho(X_{i_{r-2}}) + \rho(X_{i_1} \cdots X_{i_{r-3}} X_{i_{r-2}}) \rho(X_{i_{r-1}} X_{i_r}) \\ &\quad + \rho(X_{i_1} \cdots X_{i_{r-3}}) \rho(X_{i_{r-2}} X_{i_{r-1}} X_{i_r}) - \rho(X_{i_1} \cdots X_{i_{r-3}}) \rho(X_{i_{r-1}} X_{i_r}) \rho(X_{i_{r-2}}) \\ &\quad + \sum_{\alpha \neq \beta \neq \gamma} (X_{i_1} \cdots X_{i_{r-3}})^\alpha (X_{i_{r-1}} X_{i_r})^\beta (X_{i_{r-2}})^\gamma, \end{aligned} \quad (151)$$

where third-order YJM-elements  $\rho(X_{i_{r-2}}X_{i_{r-1}}X_{i_r}), \rho(X_{i_{r-2}}X_{i_{r-1}}X_{i_r})$  are used for  $k = 3$ . Substituting these identities into Eq.(149), we find the formula crafting  $\rho(X_{i_1} \cdots X_{i_r})$  when  $k = 3$ . Expanding it on  $H^{\otimes 4}$  and using the procedure described above, we prove the claim by induction and then leverage Okounkov-Vershik theorem [9].  $\square$

We finally conclude that

**Theorem III.11.** *For a general  $n$ -qudit system, the  $k$ th order CQA group*

$$CQA^{(k)} = \left\langle \exp(-i \sum_{i_1, \dots, i_k} \beta_{i_1 \dots i_k} X_{i_1} \cdots X_{i_k}), \exp(-i\gamma H_S) \right\rangle, \quad (152)$$

where  $H_S$  is the summation of all adjacent transpositions (see Section IB), forms the exact  $k$ -design with  $SU(d)$  symmetry, i.e.,  $T_k^{CQA^{(k)}} = T_k^{Haar}$ .

#### IV. APPROXIMATING UNITARY $k$ -DESIGN WITH $SU(d)$ SYMMETRY BY CQA ENSEMBLES

After discussing exact  $k$ -design via rigorous group representation theory, it is now of interests to check how to approximate the  $k$ -fold channel or  $k$ th moment operator of  $U(\bigoplus_{\lambda} S^{\lambda})$  in practice. In the following context, we define a series of ensembles  $\mathcal{E}$  sampling through one-parameter subgroups or time evolution of YJM-elements (Definition IV.1) and prove that they are approximate  $k$ -design in Theorem IV.6. We then analyze the efficiency of approximation, i.e., the scaling behavior of the needed circuit depth  $p$  with the system size  $n$ . Mathematically, this requires to bound the second largest eigenvalue of  $T_k^{\mathcal{E}}$  or evaluate its frame potential. However, as introduced in the main text and Section II D in this supplementary material, most widely known theories developed or used in [26, 34, 38, 40, 56–59] are invalid under  $SU(d)$  symmetry. We present more details in the following with several theoretical and numerical approaches built on  $S_n$  representation theory [2–4],

##### A. CQA Ensemble and Its Variants

Let us now define various sampling strategies of  $SU(d)$  symmetric unitaries on a quantum circuit by the CQA model. The most basic method is sampling from the *one-parameter subgroups* of transpositions, i.e.,

$$\{\exp(-it(i, j)); t \in \mathbb{R}\} \subset U(\bigoplus_{\lambda} S^{\lambda}). \quad (153)$$

Since the eigenvalues of any  $(i, j)$  are just  $\pm 1$ , the one-parameter subgroup is compact and isomorphic with the circle  $S^1 \cong U(1)$ . Then it suffices to restrict  $t \in [0, 2\pi]$ . As a reminder, there is no guarantee that an arbitrary one-parameter subgroups is compact, e.g.,

$$\left\{ \begin{pmatrix} e^{-it} & 0 \\ 0 & e^{-iat} \end{pmatrix}, t \in \mathbb{R} \right\} \subset SU(2), \quad (154)$$

with  $a$  being an irrational number, is non-compact and in order to sample each element from it,  $t$  has to be taken from the whole  $\mathbb{R}$ . Analogously, we may sample on the following subgroup defined by second order YJM-elements:

$$\{\exp(-i \sum_{k,l} \beta_{kl} X_k X_l); \beta_{kl} \in \mathbb{R}\} \subset U(\bigoplus_{\lambda} S^{\lambda}). \quad (155)$$

Again, since the eigenvalues of YJM-elements are integers (see Eq.(4)) and since they commute with each other, the subgroup is compact and isomorphic with a certain torus as a product of  $S^1 \cong U(1)$ . Then  $\beta_{kl} \in [0, 2\pi]$ .

On the other hand, we could sample local  $SU(d)$ -symmetric unitaries supported on arbitrary  $N$  qudits in an abstract sense. By Schur-Weyl duality, when  $N = 2$ , this sampling method is identical with that in Eq.(153). Later we illustrate how to sample some 4-local unitaries explicitly as the CQA model is generated by 4-local unitaries.

**Definition IV.1.** The *CQA ensemble* is defined as follows in each step of the random walk on the quantum circuit (see remark in Section II B):

1. We first sample an element parameterized as  $\exp(-i \sum_{k,l} \beta_{kl} X_k X_l)$  by second order YJM-elements with  $\beta_{kl} \in [0, 1]$ .
2. Then we randomly select an integer  $j \in \{1, \dots, n-1\}$  and then sample an element from the one-parameter subgroup determined by  $\exp(-it(j, j+1))$  with  $t \in [0, 2\pi]$ .

3. We sample again from the subgroup defined by  $\exp(-i \sum_{k,l} \beta_{kl} X_k X_l)$ .

**Definition IV.2.** In each step of the random walk, we randomly select four integers  $i_1, i_2, i_3, i_4$  from  $1, 2, \dots, n$  and then uniformly sample a 4-local  $SU(d)$  symmetric unitary supported on these qudits labeled by these integers. This assembles the  $\mathcal{V}_4$  ensemble.

**Definition IV.3.** Forgetting the YJM-elements, the *SWAP ensemble*  $\mathcal{E}_{\text{SWAP}}$  in each step of the random walk only samples  $\exp(-it(j, j+1))$  as a *1-dimensional chain* in the language of quantum many body theory or samples  $\exp(-it(i, j))$  with arbitrary  $1 \leq i, j \leq n$  knowing as *all-to-all interaction random circuits*.

Based on discussions from Section III, it is natural to anticipate that the first two ensembles defined above approximate unitary  $k$ -design with  $k < n$ . The third one only works for qubits and we explicitly show a counterexample on qutrits  $d = 3$  after proving these facts mathematically.

**Lemma IV.4.** The  $k$ -fold channel  $T_k^{\mathcal{E}_{\text{CQA}}}$  defined in each step of the CQA ensemble satisfies

$$T_k^{\mathcal{E}_{\text{CQA}}} = T_k^{\text{YJM}} \frac{1}{n-1} (T_k^{(1,2)} + \dots + T_k^{(n-1,n)}) T_k^{\text{YJM}}, \quad (156)$$

where  $T_k^{\text{YJM}}, T_k^{(j,j+1)}$  are the  $k$ -fold channels twirled over tori (Eq.(155)) and circles (Eq.(153)) respectively. The operators  $T_k^{\mathcal{E}_{\text{CQA}}}$  is positive semidefinite with eigenvalues being bounded in  $[0, 1]$ . Similar results hold for  $T_k^{\mathcal{E}_{\mathcal{V}_4}}$  and  $T_k^{\mathcal{E}_{\text{SWAP}}}$ .

*Proof.* By definition,

$$\begin{aligned} T_k^{\mathcal{E}_{\text{CQA}}}(M) &= \int_{\mathcal{E}_{\text{CQA}}} V^{\otimes k} M V^{\dagger \otimes k} dV \\ &= \sum_{j=1}^{n-1} \frac{1}{n-1} \int \left( V_{\text{YJM}} V_{(j,j+1)} V_{\text{YJM}} \right)^{\otimes k} M \left( V_{\text{YJM}} V_{(j,j+1)} V_{\text{YJM}} \right)^{\dagger \otimes k} dV_{\text{YJM}} dV_{(j,j+1)} \\ &= (T_k^{\text{YJM}} \frac{1}{n-1} (T_k^1 + \dots + T_k^{n-1}) T_k^{\text{YJM}})(M). \end{aligned} \quad (157)$$

Since  $T_k^{(i,j)}, T_k^{\text{YJM}}$  are twirled over compact subgroups, they are Hermitian projectors (see Section II A). Then by basic linear algebra,  $T_k^{\mathcal{E}_{\text{CQA}}}$  is positive semidefinite with largest eigenvalue be bounded by 1.  $\square$

**Lemma IV.5.** Let  $\text{Comm}_k(\text{YJM})$  denote the commutant of the torus defined in Eq.(155) with  $\text{Comm}_k(i, j)$  be defined analogously. The following identity of commutant holds for any  $k$ :

$$\text{Comm}_k(\text{YJM}) \cap \bigcap_{1 \leq j \leq n-1} \text{Comm}_k(j, j+1) = \text{Comm}_k(\text{CQA}) \quad (158)$$

$$\bigcap_{1 \leq j \leq n-1} \text{Comm}_k(j, j+1) = \bigcap_{1 \leq i < j \leq n} \text{Comm}_k(i, j) = \text{Comm}(\text{eSWAP}). \quad (159)$$

*Proof.* The statement holds trivially for  $k = 1$  by the definitions of CQA and eSWAP (see Remark in Section III B). Let  $k = 2$ , since any unitary  $U \in \text{CQA}$  is a finite product as

$$\exp(-i \sum_{k,l} \beta_{kl} X_k X_l) \exp(-i \gamma \sum_j (j, j+1)) \dots \exp(-i \sum_{k,l} \beta'_{kl} X_k X_l) \exp(-i \gamma' \sum_j (j, j+1)), \quad (160)$$

the tensor product

$$\begin{aligned} U \otimes U &= (\exp(-i \sum_{k,l} \beta_{kl} X_k X_l))^{\otimes 2} (\exp(-i \gamma \sum_j (j, j+1)))^{\otimes 2} \dots \\ &\quad \dots (\exp(-i \sum_{k,l} \beta'_{kl} X_k X_l))^{\otimes 2} (\exp(-i \gamma' \sum_j (j, j+1)))^{\otimes 2}. \end{aligned} \quad (161)$$

By the identity

$$(\exp A) \otimes (\exp B) = \exp(A \otimes I + I \otimes B), \quad (162)$$

for any  $M \in \text{Comm}_2(1, 2) \cap \dots \cap \text{Comm}_2(n-1, n) \cap \text{Comm}_2(\text{YJM})$ , proving  $M$  commutes with  $U \otimes U$  for any  $U \in \text{CQA}$  is equivalent to show that  $M$  commutes with  $A \otimes I + I \otimes A$  with  $A$  be taken from the Lie algebra of CQA (a similar trick is also used in Theorem III.10).

By assumption,

$$[M, (j, j+1) \otimes I + I \otimes (j, j+1)] = 0, \quad [M, X_k X_l \otimes I + I \otimes X_k X_l] = 0. \quad (163)$$

On the other hand, due to the definition of tensor product representation, the following identity holds for any matrices  $A, B \in \text{End}(V)$ :

$$[A \otimes I + I \otimes A, B \otimes I + I \otimes B] = [A, B] \otimes I + I \otimes [A, B]. \quad (164)$$

Therefore,  $M$  commutes with the tensor product representation of transpositions and YJM-elements, which span the Lie algebra of CQA and hence the proof follows. The converse direction is obvious.

For eSWAP, we have the following argumentation:

$$\begin{aligned} & [M, (i, i+1) \otimes I + I \otimes (i, i+1)] = 0 \\ \implies & [M, ((i, i+1) \otimes I + I \otimes (i, i+1))^2] = 2[M, (i, i+1) \otimes (i, i+1) + I \otimes I] = 0 \\ \implies & [M, (j, j+1) \otimes (j, j+1)] = 0 \\ \implies & [M, (j, j+2) \otimes I + I \otimes (j, j+2)] \\ & = [M, (j+1, j+2) \otimes (j, j+1)((j, j+1) \otimes I + I \otimes (j, j+1))(j, j+1) \otimes (j+1, j+2)] = 0. \end{aligned} \quad (165)$$

Inductively, we derive that  $M$  commutes with  $(i, j) \otimes I + I \otimes (i, j)$  for any  $i \neq j$ . The case for general  $k$  can be demonstrated similarly.  $\square$

**Theorem IV.6.** *The ensembles  $\mathcal{E}_{\text{CQA}}$  forms an approximate  $k$ -design to the group CQA. Analogously,  $\mathcal{E}_{\mathcal{V}_4}$  and  $\mathcal{E}_{\text{SWAP}}$  approximate  $k$ -design to  $\mathcal{V}_4$  and eSWAP respectively.*

*Proof.* As mentioned in Section II B, from the perspective of commutant theory and operator eigenvalues,  $\mathcal{E}_{\text{CQA}}$  approximate CQA as  $k$ -design if and only if  $T_k^\mathcal{E}$  and  $T_k^{\text{CQA}}$  share the same unit eigenspace. For compact groups like CQA, this is just the commutant algebra  $\text{Comm}_k(\text{CQA})$  by invariance of Haar measure. However, for a general ensemble like  $\mathcal{E}_{\text{CQA}}$ , we can only say by definition that the unit eigenspace  $W_{k, \mathcal{E}_{\text{CQA}}}^{\lambda=1}$  contains  $\text{Comm}_k(\mathcal{E}_{\text{CQA}})$ . We need to demonstrate following identity:

$$\text{Comm}_k(\text{CQA}) \supset W_{k, \text{CQA}}^{\lambda=1}. \quad (166)$$

To this end, let  $M$  be any (super-)operator such that  $T_k^{\mathcal{E}_{\text{CQA}}}(M) = M$ . That is,  $M \in W_{k, \mathcal{E}_{\text{CQA}}}^{\lambda=1}$ . By Lemma IV.4,

$$T_k^{\text{YJM}}(M) = T_k^{\text{YJM}} T_k^{\mathcal{E}_{\text{CQA}}}(M) = (T_k^{\text{YJM}})^2 \frac{1}{n-1} (T_k^{(1,2)} + \dots + T_k^{(n-1,n)}) T_k^{\text{YJM}}(M) = T_k^{\mathcal{E}_{\text{CQA}}}(M) = M, \quad (167)$$

which means that  $M \in \text{Comm}_k(\text{YJM})$ . Then

$$T_k^{\mathcal{E}_{\text{CQA}}}(M) = T_k^{\text{YJM}} \frac{1}{n-1} \frac{1}{n-1} (T_k^{(1,2)} + \dots + T_k^{(n-1,n)}) T_k^{\text{YJM}}(M) = T_k^{\text{YJM}} \frac{1}{n-1} (T_k^{(1,2)} + \dots + T_k^{(n-1,n)})(M). \quad (168)$$

Assume there is a certain  $i_0 \in \{1, \dots, n-1\}$  such that  $M \notin \text{Comm}_k(i_0, i_0+1)$ . Since  $T_k^{(i_0, i_0+1)}$  is a Hermitian projector, its operator norm is exactly 1 and then

$$\frac{1}{n-1} \left\| (T_k^{(1,2)} + \dots + T_k^{(n-1,n)})(M) \right\| \leq \frac{1}{n-1} \sum_{j=1}^{n-1} \|T_k^{j,j+1}(M)\| < \|M\|, \quad (169)$$

which contradicts the fact that  $T_k^{\mathcal{E}_{\text{CQA}}}(M) = M$ . Therefore,

$$M \in \text{Comm}_k(1, 2) \cap \dots \cap \text{Comm}_k(n-1, 1) \cap \text{Comm}_k(\text{YJM}) = \text{Comm}_k(\text{CQA}) \quad (170)$$

by Lemma IV.5. Since  $T_k^{\mathcal{E}_{\text{CQA}}}$  is positive semidefinite, any other non-unit eigenvalues are strictly bounded in  $[0, 1)$ . As we instantiated in Eq.(42),  $\mathcal{E}_{\text{CQA}}$  approximates CQA as  $k$ -designs.

As a reminder, the above inequality may not hold for non-Hermitian projectors likes

$$Pv = \begin{pmatrix} 1 & 0 \\ 1 & 0 \end{pmatrix} \begin{pmatrix} 1 \\ 0 \end{pmatrix} = \begin{pmatrix} 1 \\ 1 \end{pmatrix}. \quad (171)$$

The norm of the image even increases.  $\square$



Together with Theorem (III.4) III.11, we conclude in this subsection that:

**Corollary IV.7.** *The ensemble  $\mathcal{E}_{\text{CQA}}$ , as well as  $\mathcal{E}_{\mathcal{V}_d}$ , forms an approximate  $k$ -design to  $\text{U}(\bigoplus_{\lambda} S^{\lambda})$  on general qudits for all  $k < \frac{1}{2}n(n-3)$ . Employing higher order YJM-elements in constructing the ensemble would approximate higher unitary design. The ensemble  $\mathcal{E}_{\text{SWAP}}$  forms an approximate  $k$ -design to  $\text{U}(\bigoplus_{\lambda} S^{\lambda})$  on qubits for  $k < n^2$ .*

*Remark.* It is always desirable to use  $\mathcal{E}_{\text{SWAP}}$  as it involves 2-local unitaries and most of our numerical computations are based on  $\mathcal{E}_{\text{SWAP}}$ . However, we keep in mind that  $\mathcal{E}_{\text{SWAP}}$  cannot approximate unitary  $k$ -design when  $d > 2$  and  $k > 1$  [30] and present how to spot counterexamples explicitly by  $S_n$  representation theory, which may provide a deep understanding on this topic.

Following the results from [28, 29] which asserts that eSWAPs cannot generate  $\text{SU}(S^{\lambda})$  if  $\lambda = (\lambda_i)$  is not a hook, i.e.,  $\lambda_2 > 1$  and equals its conjugate (see Eq.(12)), we take

$$\lambda_0 = \begin{array}{|c|c|c|} \hline & & \\ \hline & & \\ \hline & & \\ \hline \end{array} = \lambda'_0 \quad (172)$$

which uniquely corresponds to an  $S_6$  irrep sector (with copies) decomposed from the six-qudit system and  $d$  must be larger than 2. Recall that in Section III B we compare  $T_k^{\text{Haar}}$  and  $T_k^{\text{CQA}}$  by expanding those tensor products  $V^{\otimes k} \otimes \bar{V}^{\otimes k}$  with respect to  $S_n$  irrep sectors and then taking integral.

For approximate design, we are also able to expand  $T_k^{\mathcal{E}_{\text{SWAP}}}$  by different irrep blocks. Especially, we can compute the number of unit eigenvalues of restricted on

$$\frac{1}{2\pi} \int_0^{2\pi} (e^{-it(1,2)}|_{S^{\lambda_0}})^{\otimes k} \otimes (e^{it(1,2)}|_{S^{\lambda_0}})^{\otimes k} dt. \quad (173)$$

When  $k = 2$  for instance, we compute by Young orthogonal form that the above matrix has *three* unit eigenvalues. On the other hand, it is straightforward to see by Theorem II.8 that the corresponding expanded term from  $T_k^{\text{Haar}}$

$$\int_{\text{U}(S^{\lambda_0})} (U_{S^{\lambda_0}})^{\otimes 2} \otimes (\bar{U}_{S^{\lambda_0}})^{\otimes 2} d(U_{S^{\lambda_0}}). \quad (174)$$

only has *two* unit eigenvalues (see Eq.(70)) resembling the commutant of a common 2-design with no prescribed symmetry. Therefore,  $(T_2^{\mathcal{E}_{\text{SWAP}}})^p$  can never converge to  $T_2^{\text{Haar}}$  because it strictly has more unit eigenvalues. Taking  $T_2^{\text{YJM}} T_2^{\mathcal{E}_{\text{SWAP}}} T_2^{\text{YJM}}$  by  $T_2^{\text{YJM}}$  resolves this problem and makes the eigenvectors coincide. Other counterexamples can be found in a similar manner on Young diagrams like  $\lambda_0$  and a comprehensive explanation on the numerical computation of the eigensystem of Eq.(173) is given in the subsequent subsection.

## B. Several Attempts to Evaluate the Convergence Speed of $\mathcal{E}_{\text{CQA}}$

An important question to address now is how quickly the aforementioned ensembles converge to an  $\epsilon$ -approximate  $\text{SU}(d)$ -symmetric  $k$ -designs. This is also referred to as the *scrambling speed* in quantum chaos [36, 37, 39]. We now compute the second largest eigenvalue for  $k = 1, 2$  and discuss the difficulties for general case in the meantime.

Since any transposition or SWAP  $\tau = (i, j) \in S_n$  satisfies  $\tau^2 = I$ , its time evolution can be expanded by Euler identity:

$$e^{-i\theta\tau} = \cos \theta I - i \sin \theta \tau. \quad (175)$$

Then

$$T_{k=1}^{\tau} = \frac{1}{2\pi} \int_0^{2\pi} e^{-i\theta\tau} \otimes e^{i\theta\tau} d\theta = \frac{1}{2\pi} \int_0^{2\pi} (\cos \theta I - i \sin \theta \tau) \otimes (\cos \theta I + i \sin \theta \tau) d\theta = \frac{1}{2} (I \otimes I + \tau \otimes \tau), \quad (176)$$

and

$$\begin{aligned} T_{k=2}^{\tau} &= \frac{1}{2\pi} \int_0^{2\pi} (e^{-i\theta\tau})^{\otimes 2} \otimes (e^{i\theta\tau})^{\otimes 2} d\theta = \frac{1}{2\pi} \int_0^{2\pi} (\cos \theta I + i \sin \theta \tau)^{\otimes 2} \otimes (\cos \theta I - i \sin \theta \tau)^{\otimes 2} d\theta \\ &= \frac{1}{2\pi} \int_0^{2\pi} \left( \cos^4 \theta I \otimes I \otimes I \otimes I + \sin^4 \theta \tau \otimes \tau \otimes \tau \otimes \tau + \cos^2 \theta \sin^2 \theta (I \otimes \tau \otimes I \otimes \tau + I \otimes \tau \otimes \tau \otimes I \right. \\ &\quad \left. + \tau \otimes I \otimes I \otimes \tau + \tau \otimes I \otimes \tau \otimes I - I \otimes I \otimes \tau \otimes \tau - \tau \otimes \tau \otimes I \otimes I) \right) d\theta \\ &= \frac{1}{8} (3IIII + 3\tau\tau\tau\tau + I\tau I\tau + I\tau\tau I + \tau I I\tau + \tau I\tau I - II\tau\tau - \tau\tau II), \end{aligned} \quad (177)$$

where we omit the tensor product notation in the end for conciseness. Expansion of  $T_k^\tau$  for general  $k$  can be evaluated by  $\sin^2 \theta + \cos^2 \theta = 1$  and

$$\frac{1}{2\pi} \int_0^{2\pi} \cos^{2k} \theta d\theta = \frac{1}{2\pi} \int_0^{2\pi} \sin^{2k} \theta d\theta = \frac{1}{2^{2k}} \binom{2k}{k}, \quad (178)$$

$$\frac{1}{2\pi} \int_0^{2\pi} \cos^{2k-1} \theta \sin \theta d\theta = \frac{1}{2\pi} \int_0^{2\pi} \cos \theta \sin^{2k-1} \theta d\theta = 0. \quad (179)$$

We now rigorously analyze the magnitude of the second largest eigenvalue of  $T_{k=1}^{\mathcal{E}_{\text{CQA}}}$  for 1-design. Even it is the simplest case, an elaborated treatment shed the light on how to conduct numerical computations for larger  $k$  and uncover the main obstacles when tackling unitary  $k$ -design with  $\text{SU}(d)$  symmetry mathematically.

#### Using Quantum Many Body Theory

As in proving Lemma IV.5, Eq.(176) indicates that

$$M \in \text{Comm}_1(\mathcal{E}_{\text{SWAP}}) \subset \text{End}(V^{\otimes n}) \quad (180)$$

commutes with all adjacent transpositions  $\tau = (j, j+1)$  and hence commute with the group  $S_n$ . Therefore, it is sufficient to employ

$$T_k^{\mathcal{E}_{\text{SWAP}}} = \frac{1}{n} (T_k^{(1,2)} + \dots + T_k^{(n-1,n)} + T_k^{(1,n)}) \quad (181)$$

to approximate the 1-design for either qubits or general qudits. Obviously, determining the second largest eigenvalue of the positive semidefinite operator  $T_k^{\mathcal{E}_{\text{SWAP}}}$  is equivalent to find the *spectral gap* of

$$H := n(I - T_k^{\mathcal{E}_{\text{SWAP}}}) = \sum_i (I - T_k^{(i,i+1)}) = \sum_i P_i, \quad (182)$$

which is further tantamount to find some  $\gamma = \Delta(H) > 0$  such that

$$H^2 \geq \gamma H. \quad (183)$$

This observation brings us to apply a classical method due to Knabe [56] which was originally devised to estimate the spectral gap of 1-dimensional quantum spin chain with *periodic boundary condition*. As a brief introduction, let us define the *bulk Hamiltonian* consisting of all  $P_j, \dots, P_{m+j-1}$  terms from Eq.(182):

$$h_{m,j} = \sum_{i=j}^{m+j-1} P_i. \quad (184)$$

It can be seen by Eq.(176) and (177) that for any  $j, j', h_{m,j}$  and  $h_{m,j'}$  are similar because  $h_{m,j'}$  can be transformed from  $h_{m,j}$  simply by tensor products of permutations  $\sigma \in S_n$ . Thus,

$$\Delta(h_{m,j}) = \Delta(h_{m,j'}) \text{ for all } j, j' \quad (185)$$

and we say that the system is *permutation-invariant*. The improved Knabe local gap theory [59] says that

$$\Delta(H) \geq \frac{5(m^2 + 3m + 1)}{6(m^2 + 2m - 3)} \left( \Delta(h_{m,j}) - \frac{6}{(m+1)(m+2)} \right). \quad (186)$$

To obtain a valid lower bound on the gap, we shall find a certain  $m = 2, 3, \dots$  such that  $\Delta(h_{m,j}) > \frac{6}{(m+1)(m+2)}$ .

Let  $m = 2$ , it suffices to compute the gap of

$$P_1 + P_2 = 2I - T_{k=1}^{(1,2)} - T_{k=1}^{(2,3)} = I - \frac{1}{2} \left( (1,2)^{\otimes 2} + (2,3)^{\otimes 2} \right). \quad (187)$$

by permutation-invariance of  $h_{2,j}$ . We present a simple but crucial observation to build our computational method:

**Observation.** The symmetric group  $S_3$  only admits the 1-dimensional trivial and sign irreps and the 2-dimensional fundamental irrep labeled by  $(3), (1^3), (2, 1)$  respectively. The Young orthogonal forms (see Eq.(5)) of  $\tau = (1, 2)$  and  $(2, 3)$  on the direct sum of all these irreps are given as

$$(1, 2) = \begin{pmatrix} 1 & 0 & 0 & 0 \\ 0 & 1 & 0 & 0 \\ 0 & 0 & -1 & 0 \\ 0 & 0 & 0 & -1 \end{pmatrix}, \quad (2, 3) = \begin{pmatrix} 1 & 0 & 0 & 0 \\ 0 & -\frac{1}{2} & \frac{\sqrt{3}}{2} & 0 \\ 0 & \frac{\sqrt{3}}{2} & \frac{1}{2} & 0 \\ 0 & 0 & 0 & -1 \end{pmatrix}. \quad (188)$$

Then for arbitrary  $n \geq 3$  and  $j = 1, \dots, n$ ,  $\Delta(h_{2,j})$  equals the gap of

$$I - \frac{1}{2} \left( \begin{pmatrix} 1 & 0 & 0 & 0 \\ 0 & 1 & 0 & 0 \\ 0 & 0 & -1 & 0 \\ 0 & 0 & 0 & -1 \end{pmatrix}^{\otimes 2} + \begin{pmatrix} 1 & 0 & 0 & 0 \\ 0 & -\frac{1}{2} & \frac{\sqrt{3}}{2} & 0 \\ 0 & \frac{\sqrt{3}}{2} & \frac{1}{2} & 0 \\ 0 & 0 & 0 & -1 \end{pmatrix}^{\otimes 2} \right). \quad (189)$$

The underlying reason is due to  $S_n$  branching rule: given any  $S_n$  irrep  $S^\lambda$  with  $\lambda \vdash n$ . Obviously,  $S_{n-1}$  also acts on it by the natural embedding into the first  $n-1$  nodes of  $S_n$ . As a representation of  $S_{n-1}$ ,  $S^\lambda$  further decomposes into irreps corresponding to Young diagrams  $\mu \vdash n-1$ , which are sub-diagram of  $\lambda$  with one box being deleted. Inductively, we can decompose  $S_{n-1}$  irreps on  $S_{n-2}$  and so forth (see [1–4] for more details). For the present example, given an arbitrary large  $n$ -qudit system, the matrix representations of  $(1, 2)$  and  $(2, 3)$ , based on the branching rule, are just repetitions of sub-blocks from Eq.(188). Even these sub-blocks may repeat with different times, (formally,  $S_3$  irreps with different multiplicities may emerge), it causes no difference in computing the spectrum of  $h_{2,1} = P_1 + P_2$  and hence the gap.

Exact diagonalization gives us  $\Delta(h_{2,j}) = \frac{1}{2}$  which is just unable to use Eq.(186), so we continue to test the case for  $m = 3$  with the following Young orthogonal forms of direct sums of  $S_4$  irreps:

$$(1, 2) = \begin{pmatrix} 1 & 0 & 0 & 0 & 0 & 0 & 0 & 0 & 0 & 0 \\ 0 & 1 & 0 & 0 & 0 & 0 & 0 & 0 & 0 & 0 \\ 0 & 0 & -1 & 0 & 0 & 0 & 0 & 0 & 0 & 0 \\ 0 & 0 & 0 & 1 & 0 & 0 & 0 & 0 & 0 & 0 \\ 0 & 0 & 0 & 0 & -1 & 0 & 0 & 0 & 0 & 0 \\ 0 & 0 & 0 & 0 & 0 & 1 & 0 & 0 & 0 & 0 \\ 0 & 0 & 0 & 0 & 0 & 0 & 1 & 0 & 0 & 0 \\ 0 & 0 & 0 & 0 & 0 & 0 & 0 & 1 & 0 & 0 \\ 0 & 0 & 0 & 0 & 0 & 0 & 0 & 0 & -1 & 0 \\ 0 & 0 & 0 & 0 & 0 & 0 & 0 & 0 & 0 & -1 \end{pmatrix}, \quad (2, 3) = \begin{pmatrix} 1 & 0 & 0 & 0 & 0 & 0 & 0 & 0 & 0 & 0 \\ 0 & -\frac{1}{2} & \frac{\sqrt{3}}{2} & 0 & 0 & 0 & 0 & 0 & 0 & 0 \\ 0 & \frac{\sqrt{3}}{2} & \frac{1}{2} & 0 & 0 & 0 & 0 & 0 & 0 & 0 \\ 0 & 0 & 0 & 1 & 0 & 0 & 0 & 0 & 0 & 0 \\ 0 & 0 & 0 & 0 & \frac{1}{2} & \frac{\sqrt{3}}{2} & 0 & 0 & 0 & 0 \\ 0 & 0 & 0 & 0 & \frac{\sqrt{3}}{2} & -\frac{1}{2} & 0 & 0 & 0 & 0 \\ 0 & 0 & 0 & 0 & 0 & 0 & -\frac{1}{2} & \frac{\sqrt{3}}{2} & 0 & 0 \\ 0 & 0 & 0 & 0 & 0 & 0 & \frac{\sqrt{3}}{2} & \frac{1}{2} & 0 & 0 \\ 0 & 0 & 0 & 0 & 0 & 0 & 0 & 0 & -1 & 0 \\ 0 & 0 & 0 & 0 & 0 & 0 & 0 & 0 & 0 & -1 \end{pmatrix}, \quad (3, 4) = \begin{pmatrix} 1 & 0 & 0 & 0 & 0 & 0 & 0 & 0 & 0 & 0 \\ 0 & 1 & 0 & 0 & 0 & 0 & 0 & 0 & 0 & 0 \\ 0 & 0 & -1 & 0 & 0 & 0 & 0 & 0 & 0 & 0 \\ 0 & 0 & 0 & -\frac{1}{3} & 0 & \frac{2\sqrt{2}}{3} & 0 & 0 & 0 & 0 \\ 0 & 0 & 0 & 0 & 1 & 0 & 0 & 0 & 0 & 0 \\ 0 & 0 & 0 & \frac{2\sqrt{2}}{3} & 0 & \frac{1}{3} & 0 & 0 & 0 & 0 \\ 0 & 0 & 0 & 0 & 0 & 0 & -1 & 0 & 0 & 0 \\ 0 & 0 & 0 & 0 & 0 & 0 & 0 & -\frac{1}{3} & \frac{2\sqrt{2}}{3} & 0 \\ 0 & 0 & 0 & 0 & 0 & 0 & 0 & \frac{2\sqrt{2}}{3} & \frac{1}{3} & 0 \\ 0 & 0 & 0 & 0 & 0 & 0 & 0 & 0 & 0 & -1 \end{pmatrix} \quad (190)$$

Note that these matrices are made up from sub-matrices defined on inequivalent  $S_m$  irreps. To avoid tensor product of large matrices as above, we take insights from Section III A computing with sub-matrices.

We now describe the bad situation for 2-design where we compute by Eq.(177) involving 4-fold tensor products. As in the previous case,  $\Delta(h_{m,j}) < \frac{6}{(m+1)(m+2)}$  for  $m = 2, 3, 4, 5, 6$ . For larger  $m$ , although we can expand the tensor product by  $S_m$  irreps, it immediately becomes hard to diagonalize  $h_{m,j}$  because a single irrep may scale exponentially (see (20) and (21)), no to mention its 4-fold tensor product. Instead of finding the complete spectra, we examine Eq.(177) where  $\tau$  are restricted to *part of*  $S_n$  irreps with moderate dimensions like those assigned on  $S^{(m)} \otimes S^{(m-1,1)} \otimes S^{(m-2,2)} \otimes S^{(m-1,1)}$ . Unavoidably, as reported in the numerical part of the main text, there are eigenvalues smaller than  $\frac{6}{(m+1)(m+2)}$  and this indicates that the  $\Delta(h_{m,j})$  could not cross that local gap threshold for larger  $m$ . This decay of  $\Delta(h_{m,j})$  is also the evidence to rule out the possibility of using *Nachtergaele's martingale method* [57] which detects constant gaped ( $\Omega(n^{-1})$  after normalization) 1-dimensional quantum spin chains.

*Remark.* It is still of interests whether Knabe local gap theory applies to the CQA ensemble on general qudits with

$$T_k^{\mathcal{E}_{\text{CQA}}} = T_k^{\text{YJM}} \left( \frac{1}{n-1} \sum_{1 \leq j \leq n-1} T_k^{\tau_j} \right) T_k^{\text{YJM}}. \quad (191)$$

The answer is negative because we cannot define a bulk Hamiltonian  $h_{m,j}$  as Eq.(184) requiring  $m < n$  as the interaction range of terms in  $h_{m,j}$ . Given  $\tau_1 = (i, i+1), \tau_2 = (j, j+1)$  with  $i+1 < j$ , due to the intertwining with  $T_k^{\text{YJM}}, T_k^{\text{YJM}} T_k^{\tau_1} T_k^{\text{YJM}}$  and  $T_k^{\text{YJM}} T_k^{\tau_2} T_k^{\text{YJM}}$  no longer commute.

To clarify this, let us restrict ourselves to the case when  $k = 2$  on a simple tensor product like  $S^{\lambda \otimes 4}$  with Young basis element  $|\alpha_T\rangle$  (we temporally omit the multiplicity index). Let  $|\alpha_{T_r}\rangle$ ,  $r = 1, 2, 3, 4$  being basis vectors where  $\tau_1, \tau_2$  acting according to the following orthogonal form:

$$(i, i+1)|\alpha_{T_1}\rangle = \frac{1}{r_1}|\alpha_{T_1}\rangle + \sqrt{1 - \frac{1}{r_1^2}}|\alpha_{T_2}\rangle, \quad (i, i+1)|\alpha_{T_2}\rangle = \frac{1}{r_1}|\alpha_{T_2}\rangle + \sqrt{1 - \frac{1}{r_1^2}}|\alpha_{T_3}\rangle, \quad (192)$$

$$(j, j+1)|\alpha_{T_1}\rangle = \frac{1}{r_2}|\alpha_{T_1}\rangle + \sqrt{1 - \frac{1}{r_2^2}}|\alpha_{T_3}\rangle, \quad (j, j+1)|\alpha_{T_2}\rangle = \frac{1}{r_2}|\alpha_{T_2}\rangle + \sqrt{1 - \frac{1}{r_2^2}}|\alpha_{T_4}\rangle. \quad (193)$$

Such a basis vector can be taken from the following Young tableau for instance:

$$\begin{array}{|c|c|c|c|c|c|c|c|c|c|} \hline 1 & 3 & 5 & \dots & \dots & i+1 & \dots & \dots & j+1 & \dots & \dots & n \\ \hline 2 & 4 & \dots & \dots & i & \dots & \dots & j & \dots & \dots & n-1 & \\ \hline \end{array} \quad (194)$$

Then one can check by definition that

$$\begin{aligned} & \left\langle E_{|\alpha_{T_1}\rangle, |\alpha_{T_3}\rangle} \otimes E_{|\alpha_{T_3}\rangle, |\alpha_{T_1}\rangle}, (T_k^{\text{YJM}} T_k^{\tau_2} T_k^{\text{YJM}})(T_k^{\text{YJM}} T_k^{\tau_1} T_k^{\text{YJM}}) E_{|\alpha_{T_1}\rangle, |\alpha_{T_1}\rangle} \otimes E_{|\alpha_{T_2}\rangle, |\alpha_{T_2}\rangle} \right\rangle \\ & \neq \left\langle E_{|\alpha_{T_1}\rangle, |\alpha_{T_3}\rangle} \otimes E_{|\alpha_{T_3}\rangle, |\alpha_{T_1}\rangle}, (T_k^{\text{YJM}} T_k^{\tau_1} T_k^{\text{YJM}})(T_k^{\text{YJM}} T_k^{\tau_2} T_k^{\text{YJM}}) E_{|\alpha_{T_1}\rangle, |\alpha_{T_1}\rangle} \otimes E_{|\alpha_{T_2}\rangle, |\alpha_{T_2}\rangle} \right\rangle, \end{aligned} \quad (195)$$

which proves the non-commutativity.

*Remark.* With very similar reason, we find that the martingale method [57] is also unavailable when studying the spectral gap of  $T_k^{\mathcal{E}_{\text{CQA}}}$  for general qudits. Adjusting notations in [57] to our case, we set

$$H_{\Lambda_m} = \sum_{i=1}^m I - T_k^{\text{YJM}} T_k^{\tau_i} T_k^{\text{YJM}}, \quad H_{\Lambda_m \setminus \Lambda_{m-l}} = \sum_{i=m-l+1}^m I - T_k^{\text{YJM}} T_k^{\tau_i} T_k^{\text{YJM}}, \quad (196)$$

where  $l \leq m \leq n$ . Let  $G_m, G_{\Lambda_m \setminus \Lambda_{m-l}}$  denote the operator that projects vectors into the ground state space of  $H_m, H_{\Lambda_m \setminus \Lambda_{m-l}}$  respectively. Assume  $m_1 \leq m_2 - l$ , violating the requirement in [57]  $G_{m_1}$  and  $G_{\Lambda_{m_2} \setminus \Lambda_{m_2-l}}$  do not commute with a similar inequality as Eq.(195):

$$\begin{aligned} & \left\langle E_{|\alpha_{T_1}\rangle, |\alpha_{T_3}\rangle} \otimes E_{|\alpha_{T_3}\rangle, |\alpha_{T_1}\rangle}, (G_{m_1} G_{\Lambda_{m_2} \setminus \Lambda_{m_2-l}}) E_{|\alpha_{T_1}\rangle, |\alpha_{T_1}\rangle} \otimes E_{|\alpha_{T_2}\rangle, |\alpha_{T_2}\rangle} \right\rangle \\ & \neq \left\langle E_{|\alpha_{T_1}\rangle, |\alpha_{T_3}\rangle} \otimes E_{|\alpha_{T_3}\rangle, |\alpha_{T_1}\rangle}, (G_{\Lambda_{m_2} \setminus \Lambda_{m_2-l}} G_{m_1}) E_{|\alpha_{T_1}\rangle, |\alpha_{T_1}\rangle} \otimes E_{|\alpha_{T_2}\rangle, |\alpha_{T_2}\rangle} \right\rangle, \end{aligned} \quad (197)$$

where the Young basis vectors are selected for example as

$$\begin{array}{|c|c|c|c|c|c|c|c|c|c|} \hline 1 & 3 & 5 & \dots & \dots & i+1 & \dots & \dots & j+1 & j+2 & j+3 & \dots & n \\ \hline 2 & 4 & \dots & \dots & i & \dots & \dots & j & \dots & \dots & \dots & \dots & \\ \hline \end{array} \quad (198)$$

*Using Properties of YJM-elements*

There is a potential approach using  $S_n$  representation theory [4, 9] with no dependence on the numerical calculation of local gaps. Replacing  $\mathcal{E}_{\text{SWAP}}$  defined by 1-dimensional adjacent transposition chain by the ensemble consisting of time evolutions of  $(1, n), (2, n), \dots, (n-1, n)$  (which is a *star* graphically). By Eq.(176),

$$\begin{aligned} T_{k=1}^{X_n} &= \frac{1}{n-1} (T_{k=1}^{(1,n)} + T_{k=1}^{(2,n)} + \dots + T_{k=1}^{(n-1,n)} + T_k^{(1,n)}) \\ &= \frac{1}{2} I + \frac{1}{2(n-1)} ((1, 2)^{\otimes 2} + (2, n)^{\otimes 2} + \dots + (n-1, n)^{\otimes 2}). \end{aligned} \quad (199)$$

Since each  $(i, j)^{\otimes 2}$  is just given by the tensor product representation of  $S_n$  on the  $n$ -qudit system,  $T_{k=1}^{X_n}$  is interpreted as the matrix representation of elements from the group algebra  $\mathbb{C}[S_n]$ . Checking carefully by definition, we see that  $T_{k=1}^{X_n}$  is just the representation of the  $n$ th YJM-element  $X_n$  (multiplying with the normalization factor  $\frac{1}{n-1}$ ) and hence the notation. As a remarkably property of YJM-elements mentioned in Section IA, their eigenvalues can be directly read off as components of

content vectors of standard Young tableaux. For  $X_n$ , the largest possible eigenvalue is  $n - 1$  and the second largest one is  $n - 2$  corresponding to eigenstates (Young basis vectors) with the following standard tableaux:

$$\begin{array}{|c|c|c|} \hline 1 & 2 & 3 \\ \hline \end{array} \dots \begin{array}{|c|c|} \hline n-1 & n \\ \hline \end{array} \quad \begin{array}{|c|c|c|} \hline 1 & 2 & 3 \\ \hline n & & \end{array} \dots \begin{array}{|c|} \hline n-1 \\ \hline \end{array} \quad (200)$$

Taking the normalization factor, we have

$$\lambda_2(T_{k=1}^{X_n}) \leq 1 - \frac{1}{n-1} \quad \text{and} \quad \Delta(T_{k=1}^{X_n}) \geq \frac{1}{n-1}. \quad (201)$$

Using (62) from the Remark of Section II C, we conclude that when

$$p \geq (n-1) \left( 2n \log d + \log \frac{1}{\epsilon} \right) \quad (202)$$

the aforementioned ensemble forms an  $\epsilon$ -approximate 1-design. For  $k > 1$  however, Eq.(177) generally does not induce a well-defined tensor product representation of YJM-elements and we are expected to see more sophisticated treatment of  $S_n$  representation theory addressing this problem.

Instead, let  $\mathcal{E}_{S_n}$  denote the ensemble consists of merely 2-local SWAPs. In each step of the random walk, we select  $(i, n)$  randomly as above Eq.(199) and then toss a fair coin. With probability  $\frac{1}{2}$ , we apply  $(i, j)$ . Otherwise, we apply the identity channel. Then

$$T_k^{\mathcal{E}_{S_n}} = \frac{1}{n-1} \sum_{i=1}^{n-1} \frac{1}{2} (I^{\otimes k} + (i, n)^{\otimes k}) \quad (203)$$

whose spectral gap is exactly the same as  $T_{k=1}^{X_n}$  discussed above, which is independent of  $k$  by properties of YJM-elements. Since SWAPs generate  $S_n$ , using simialr arguments from Theorem IV.6 the ensemble  $\mathcal{E}_{S_n}$  approximates the group design of  $S_n \subseteq \text{U}(\bigoplus_{\lambda} S^{\lambda})$  where the spectral gap of  $\mathcal{E}_{\text{CQA}}$  decreases manifestly for  $k > 1$  as we described before. Except our method using YJM-elements, studying the general Haar randomness over  $S_n$  is a fairly classical topic in probability theory with lots of profound techniques and results, i.e., determining the mixing time of repeated random SWAPs [43, 45, 60].

#### Using Random Circuits with all-to-all Interaction

Except the 1-dimensional chain ( $\mathcal{E}_{\text{SWAP}}$ ) or the star ( $\mathcal{E}_{X_n}$ ) discussed above, we may heuristically employ all kinds of transpositions  $(i, j)$  in defining the ensemble, which is referred to as *random circuits with all-to-all interactions*, and is graphically depicted as the *complete graph* over  $n$ -qudits. As mentioned in Section IV A, by Schur-Weyl duality, this is simply the  $\mathcal{V}_2$  ensemble (cf. Definition IV.2) with

$$T_k^{\mathcal{E}_{\mathcal{V}_2}} = \frac{2}{(n-1)n} \sum_{1 \leq i < j \leq n} T_k^{(i,j)}. \quad (204)$$

Analogous to the Kanbe's original derivation of 1-dimensional local gap threshold [56], we have the following lemma for complete graph:

**Lemma IV.8.** *Let*

$$H := \frac{2}{n(n-1)} (I - T_k^{\mathcal{E}_{\mathcal{V}_2}}) = \sum_{1 \leq i < j \leq n} (I - T_k^{(i,j)}) = \sum_{1 \leq i < j \leq n} P_k^{(i,j)} \quad (205)$$

and let  $h_r = \sum_{i,j \neq r} P_k^{(i,j)}$  be a local bulk Hamiltonian supported the  $n - 1$  vertices except  $r$ . Suppose  $\Delta(h_r) = \gamma_{n-1}$ , then the gap of  $H$  is lower bounded by  $\frac{1}{n-3}((n-2)\gamma_{n-1} - 1)$ . More generally, given any collection of  $m$  qubits, and let  $h_{i_1, \dots, i_m} = \sum_{i < j \in \{i_1, \dots, i_m\}} P_k^{(i,j)}$  then

$$\gamma_n \geq 1 + \frac{n-2}{m-2} (\gamma_m - 1). \quad (206)$$

*Proof.* It is widely known that the inequality  $H^2 \geq \gamma_n H$  is equivalent to say that  $\gamma_n$  is the (lower bound of) gap of  $H$ . Expanding  $H^2$  directly, we have

$$H^2 - \frac{1}{n-3} \sum_{1 \leq r \leq n} h_r^2 + \frac{1}{n-3} H \geq 0. \quad (207)$$

With the assumption on local gap of  $h_r$ ,

$$H^2 \geq \frac{1}{n-3} \sum_{1 \leq r \leq n} h_r^2 - \frac{1}{n-3} H \quad (208)$$

$$\geq \frac{1}{n-3} \sum_{1 \leq r \leq n} \gamma_{n-1} h_r - \frac{1}{n-3} H = \frac{1}{n-3} (n-2) \gamma_{n-1} H - H = \frac{1}{n-3} ((n-2) \gamma_{n-1} - 1) H. \quad (209)$$

As the inequality

$$\gamma_n \geq \frac{1}{n-3} ((n-2) \gamma_{n-1} - 1) \Leftrightarrow (n-3) \gamma_n \geq (n-2) \gamma_{n-1} - (n-2) + (n-3) \Leftrightarrow \frac{\gamma_n - 1}{\gamma_{n-1} - 1} \geq \frac{n-2}{n-3} \quad (210)$$

holds generally for all  $n$ , then by induction, we conclude that  $\gamma_n \geq 1 + (n-2) \gamma_3$  for the lowest possible  $m = 3$ .  $\square$

*Remark.* According to this lemma, if  $\gamma_m \geq 1$ ,  $\gamma_n \geq 1$  for all  $n \geq m$ . However if  $\gamma_m < 1$ , the bound of  $\gamma_n$  would finally decrease to a non-positive number and become invalid. Our numerical computation using Young orthogonal form shows that for  $m = 3, \dots, 10$ , the gap of the bulk Hamiltonian locally supported on  $m$ -qubits is always  $\frac{1}{2}$  which does not satisfy the above lemma but leave one conjecture to prove this hold for arbitrary number of qubits. Due to this constant gap conjecture, we should examine again the validity of martingale method [57]. Let

$$H_{\Lambda_m} = \sum_{1 \leq i < j \leq m} I - T_k^{(i,j)}, \quad H_{\Lambda_m \setminus \Lambda_{m-l}} = \left( \sum_{j=1}^{m-l} I - T_k^{(j, m-l+1)} + \dots + \sum_{j=1}^{m-1} I - T_k^{(j, m)} \right) \quad (211)$$

with  $G_{\Lambda_m}, G_{\Lambda_m \setminus \Lambda_{m-l}}$  being projections into the ground state subspace. One can also see by definition that  $G_{\Lambda_m} = G_{\Lambda_m \setminus \Lambda_{m-l}}$ .

Let  $m_1 \leq m_2 - l$  as in the previous remark, we check the commutativity of these projections but on  $S_{m_2}$  irrep blocks like  $S^\lambda \otimes 2 \otimes S^{\mu \otimes 2}$  with  $\lambda \neq \mu$ . Given Young basis elements  $|\alpha_{T_1}\rangle, |\alpha_{T_2}\rangle$  of  $S^\lambda, S^\mu$  respectively, according to our illustration in Section II D),

$$\begin{aligned} & \left\langle E_{|\alpha_{T_1}\rangle, |\alpha_{T_2'}\rangle} \otimes E_{|\alpha_{T_2}\rangle, |\alpha_{T_1'}\rangle}, G_{\Lambda_{m_2} \setminus \Lambda_{m_2-l}} G_{\Lambda_{m_1}} E_{|\alpha_{T_1}\rangle, |\alpha_{T_1}\rangle} \otimes E_{|\alpha_{T_2}\rangle, |\alpha_{T_2}\rangle} \right\rangle \\ &= \left\langle E_{|\alpha_{T_1}\rangle, |\alpha_{T_2'}\rangle} \otimes E_{|\alpha_{T_2}\rangle, |\alpha_{T_1'}\rangle}, G_{\Lambda_{m_2}} G_{\Lambda_{m_1}} E_{|\alpha_{T_1}\rangle, |\alpha_{T_1}\rangle} \otimes E_{|\alpha_{T_2}\rangle, |\alpha_{T_2}\rangle} \right\rangle = 0 \\ &\neq \left\langle E_{|\alpha_{T_1}\rangle, |\alpha_{T_2'}\rangle} \otimes E_{|\alpha_{T_2}\rangle, |\alpha_{T_1'}\rangle}, G_{\Lambda_{m_1}} G_{\Lambda_{m_2} \setminus \Lambda_{m_2-l}} E_{|\alpha_{T_1}\rangle, |\alpha_{T_1}\rangle} \otimes E_{|\alpha_{T_2}\rangle, |\alpha_{T_2}\rangle} \right\rangle, \end{aligned} \quad (212)$$

where the standard tableaux corresponding to the above Young basis elements can be taken like (for  $m_1 = 3, m_2 = 6$ )

$$T_1 = \begin{array}{|c|c|c|c|} \hline 1 & 3 & 5 & 6 \\ \hline 2 & 4 & & \\ \hline \end{array}, \quad T_2 = \begin{array}{|c|c|c|c|c|c|} \hline 1 & 2 & 4 & 5 & 6 \\ \hline 3 & & & & \\ \hline \end{array}, \quad T_2' = \begin{array}{|c|c|c|c|} \hline 1 & 2 & 5 & 6 \\ \hline 3 & 4 & & \\ \hline \end{array}, \quad T_1' = \begin{array}{|c|c|c|c|c|c|} \hline 1 & 3 & 4 & 5 & 6 \\ \hline 2 & & & & \\ \hline \end{array}. \quad (213)$$

There is a also recursion relation for non-local gap developed in [34] to bound the second largest eigenvalue of random circuits with all-to-all interactions with no concerning on the symmetry. As mentioned in the main text, since it is generally impossible to rewrite a generalized permutation (also see Section II D) into an  $n$ -fold tensor product, the upcoming strategy using induction on the number of qudits is elusive in our case due to the necessity to obey  $S_n$  branching rule like in (212).

### C. Numerical Methods on Qudits

After clarifying cases on qubits using  $\mathcal{E}_{\text{SWAP}}$  in the preceding subsection, we describe how to compute (partial) spectra of  $T_k^{\mathcal{E}_{\text{CQA}}}$  or  $T_k^{\mathcal{E}_{\text{V4}}}$  with higher order YJM-elements or cycles from  $S_n$ , which is indispensable for qudits with  $d > 2$ .

For YJM-elements, since they are diagonal matrices with explicit diagonal entries (see Section I A),

$$T_k^{\text{YJM}} = \int_0^{2\pi} (e^{-i \sum_{i,j} \beta_{ij} X_i X_j})^{\otimes k} \otimes (e^{i \sum_{i,j} \beta_{ij} X_i X_j})^{\otimes k} d\beta_{ij} = \prod_{i,j} \int_0^{2\pi} (e^{-i \beta_{ij} X_i X_j})^{\otimes k} \otimes (e^{i \beta_{ij} X_i X_j})^{\otimes k} d\beta_{ij} \quad (214)$$

where  $\prod_{i,j}$  refers to matrix product here, is straightforwardly calculated. This is how we compare the spectral of

$$T_6^{\text{YJM}} \frac{1}{5} (T_6^{1,2} + \dots T_6^{5,6}) T_6^{\text{YJM}} \quad \text{and} \quad T_6^{1,2} + \dots T_6^{5,6} \quad (215)$$

expanding on the  $k$ -fold tensor product of the irrep sector  $S^{(3,2,1)}$  in the end of Section IV A, which demonstrates the necessity of using second order YJM-elements to approximate unitary  $k$ -design on general qudits.

However, conjugated with YJM-elements ( $T_k^{\text{YJM}}$ ) always breaks the permutation-invariance of  $k$ -fold channel of the concerned ensemble. For instance, there is no reason to say that

$$T_k^{\text{YJM}} (T_k^{i,i+1} + T_k^{i+1,i+2}) T_k^{\text{YJM}} \quad \text{and} \quad T_k^{\text{YJM}} (T_k^{j,j+1} + T_k^{j+1,j+2}) T_k^{\text{YJM}} \quad (216)$$

are similar matrices and hence computing local gaps for the first few terms from  $T_k^{\mathcal{E}_{\text{CQA}}}$  does not even suffice to launch Kanbe's theory, as well as any other theory depending the permutation-invariance. This is why we mention in Section IV A the ensemble  $\mathcal{E}_{\mathcal{V}_4}$  randomly sampling  $\text{SU}(d)$ -symmetric unitaries supported on at most 4 qudits: the operator  $T_k \mathcal{E}_{\mathcal{V}_4}$ , like  $T_k \mathcal{E}_{\mathcal{V}_2}$ , admits the invariance by definition.

However, there is still a major problem using  $\mathcal{E}_{\mathcal{V}_4}$ . By Schur-Weyl duality, any 4-local  $\text{SU}(d)$ -symmetric unitaries can be produced by  $S_4$  group elements in principle, but there is no constructive strategy as opposite to the 2-local case where we simply take  $\exp(-it(i, j))$  on SWAPS. One may parameterize a general 4-local unitary by generalized Euler angles, but it is also not applicable here. To remedy the problem, we reformulate the definition of  $\mathcal{E}_{\mathcal{V}_4}$  as  $\mathcal{E}_4$ :

**Definition IV.9.** In each step of the random walk, we randomly select four integers  $i_1, i_2, i_3, i_4$  from  $1, 2, \dots, n$ . There are various 2-cycles, 3-cycles and  $(2, 2)$ -cycles permuting the integers. Then we uniformly sample unitaries determined by these cycles like

$$\exp\left(-it(i_1, i_2)\right), \quad \exp\left(-it((i_2 i_3 i_4) + (i_4 i_3 i_2))\right), \quad \exp\left(-it(i_1, i_3)(i_2, i_4)\right). \quad (217)$$

Note that a 3-cycle like  $(i_2, i_3, i_4)$  is not Hermitian in general, but  $(i_2, i_3, i_4) + (i_4, i_3, i_2)$  is a well-defined 3-local  $\text{SU}(d)$ -symmetric Hamiltonian. More importantly, since second order products of YJM-elements only produces cycles defined as above (see Section III B), following a similar argumentation from Lemma IV.5 and Theorem IV.6, we confirm that this modified ensemble forms approximate  $k$ -design when  $k < n$ . To compute

$$T_k^{(i_1, i_3)(i_2, i_4)} = \int (e^{-it(i_1, i_3)(i_2, i_4)})^{\otimes k} \otimes (e^{it(i_1, i_3)(i_2, i_4)})^{\otimes k} dt \quad (218)$$

$$T_k^{(i_1, i_3, i_4)} = \int (e^{-it((i_2, i_3, i_4) + (i_4, i_3, i_2))})^{\otimes k} \otimes (e^{it((i_2, i_3, i_4) + (i_4, i_3, i_2))})^{\otimes k} dt \quad (219)$$

constituting  $T_k^{\mathcal{E}_4}$ , we note that  $((i_1, i_3)(i_2, i_4))^2 = I$  and  $((i_2, i_3, i_4) + (i_4, i_3, i_2))^2 = (i_2, i_3, i_4) + (i_4, i_3, i_2) + 2I$ . Thus these Hermitian matrices only admit integer eigenvalues and hence the parameter  $t$  is restricted to  $[0, 2\pi]$ . Besides,  $T_k^{(i_1, i_3)(i_2, i_4)}$  is expanded in the same way as 2-cycle transpositions, e.g., Eq.(177).

Since the Hamiltonian  $2I - (i_2, i_3, i_4) - (i_4, i_3, i_2)$  and  $(i_2, i_3, i_4) + (i_4, i_3, i_2)$  have the same effect in determining commutant in the sense of Lemma IV.5, instead of evaluating  $T_k^{(i_1, i_3, i_4)}$  directly, we use the following fact to compute the  $k$ -fold channel twirled by unitary time evolution of  $2I - (i_2, i_3, i_4) - (i_4, i_3, i_2)$ :

$$\begin{aligned} & (2I - (i_2, i_3, i_4) - (i_4, i_3, i_2))^2 = 3(2I - (i_2, i_3, i_4) - (i_4, i_3, i_2)) \\ \implies & (2I - (i_2, i_3, i_4) - (i_4, i_3, i_2))^m = 3^{m-1}(2I - (i_2, i_3, i_4) - (i_4, i_3, i_2)) \\ \implies & e^{-it(2I - (i_2, i_3, i_4) - (i_4, i_3, i_2))} = \frac{1}{3}(e^{-i3t} - 1)(2I - (i_2, i_3, i_4) - (i_4, i_3, i_2)) + I. \end{aligned} \quad (220)$$

- 
- [1] W. Fulton, *Young tableaux: with applications to representation theory and geometry* (Cambridge University Press, Cambridge [England], 1997).
  - [2] B. E. Sagan, *The symmetric group*, 2nd ed., Graduate Texts in Mathematics, Vol. 203 (Springer-Verlag, New York, 2001) pp. xvi+238, representations, combinatorial algorithms, and symmetric functions.
  - [3] R. Goodman and N. R. Wallach, *Symmetry, Representations, and Invariants* (Springer New York, 2009).
  - [4] T. Ceccherini-Silberstein, F. Scarabotti, and F. Tolli, *Representation Theory of the Symmetric Groups* (Cambridge University Press, 2009).
  - [5] H. Zheng, Z. Li, J. Liu, S. Strelchuk, and R. Kondor, PRX Quantum **4**, 020327 (2023).



- [6] A. Young, *The Collected Papers of Alfred Young 1873–1940*, edited by G. de Beauregard Robinson (University of Toronto Press, 1977).
- [7] A.-A. Jucys, *Reports on Mathematical Physics* **5**, 107 (1974).
- [8] G. Murphy, *Journal of Algebra* **69**, 287 (1981).
- [9] A. Okounkov and A. Vershik, *Selecta Mathematica* **2**, 581 (1996).
- [10] M. Clausen and U. Baum, *Mathematics of Computation* **61**, 833 (1993).
- [11] D. K. Maslen, *Math. Comp* **67**, 1121 (1998).
- [12] G. H. Hardy and S. Ramanujan, *Proceedings of the London Mathematical Society* **s2-17**, 75 (1918).
- [13] J. V. Uspensky, *Bulletin de l’Academie des Sciences de Russie. VI serie* **14**, 199 (1920).
- [14] H. Rademacher, *Proceedings of the London Mathematical Society* **s2-43**, 241 (1938).
- [15] P. Erdos, *The Annals of Mathematics* **43**, 437 (1942).
- [16] A. Maróti, *Integers* **3** (2003).
- [17] W. De Azevedo Pribitkin, *The Ramanujan Journal* **18**, 113 (2009).
- [18] S. R. E. Ingram, *Proceedings of the American Mathematical Society* **1**, 358 (1950).
- [19] Y. Roichman, *Inventiones Mathematicae* **125**, 451 (1996).
- [20] M. Lassalle, *Mathematische Annalen* **340**, 383 (2008).
- [21] J. Gallier, *Discrete Mathematics* (Springer New York, 2011).
- [22] S. P. Mishchenko, *Sbornik: Mathematics* **187**, 81 (1996).
- [23] A. Giambruno and S. Mishchenko, *Proceedings of the American Mathematical Society* **144**, 943 (2015).
- [24] H. Krovi, *Quantum* **3**, 122 (2019).
- [25] A. Y. Vlasov, *Phys. Rev. A* **63**, 054302 (2001).
- [26] F. G. Brandao, A. W. Harrow, and M. Horodecki, *Communications in Mathematical Physics* **346**, 397 (2016).
- [27] A. Harrow and S. Mehraban, *arXiv preprint arXiv:1809.06957* (2018).
- [28] I. Marin, *Annales de l’Institut Fourier* **53**, 1323 (2003).
- [29] I. Marin, *Journal of Algebra* **310**, 742 (2007).
- [30] I. Marvian, H. Liu, and A. Hulse, *arXiv e-prints*, arXiv:2105.12877 (2021), arXiv:2105.12877 [quant-ph].
- [31] A. W. Harrow and R. A. Low, in *Approximation, Randomization, and Combinatorial Optimization. Algorithms and Techniques*, edited by I. Dinur, K. Jansen, J. Naor, and J. Rolim (Springer Berlin Heidelberg, Berlin, Heidelberg, 2009) pp. 548–561.
- [32] M. Hastings and A. Harrow, *Quantum Information and Computation* **9**, 336 (2009).
- [33] D. Gross, S. Nezami, and M. Walter, *Communications in Mathematical Physics* **385**, 1325 (2021).
- [34] J. Haferkamp and N. Hunter-Jones, *Physical Review A* **104**, 022417 (2021).
- [35] D. Gross, K. Audenaert, and J. Eisert, *Journal of Mathematical Physics* **48**, 052104 (2007).
- [36] D. A. Roberts and B. Yoshida, *Journal of High Energy Physics* **2017**, 121 (2017).
- [37] J. Cotler, N. Hunter-Jones, J. Liu, and B. Yoshida, *Journal of High Energy Physics* **2017**, 1 (2017).
- [38] N. Hunter-Jones, *arXiv preprint arXiv:1905.12053* (2019).
- [39] J. Liu, *Phys. Rev. Research* **2**, 043164 (2020).
- [40] S.-K. Jian, G. Bentsen, and B. Swingle, “Linear growth of circuit complexity from brownian dynamics,” (2022).
- [41] W. Van Dam, *On Quantum Computation Theory*, Ph.D. thesis (2002).
- [42] R. A. Low, *Pseudo-randomness and Learning in Quantum Computation*, Ph.D. thesis (2010).
- [43] P. Diaconis, *Group representations in probability and statistics*, Lecture notes-monograph series No. v. 11 (Institute of Mathematical Statistics, Hayward, Calif, 1988).
- [44] D. Applebaum, *Probability on Compact Lie Groups*, Probability Theory and Stochastic Modelling, Vol. 70 (Springer International Publishing, 2014).
- [45] E. S. Meckes, *The random matrix theory of the classical compact groups*, Cambridge tracts in mathematics No. 212 (Cambridge University Press, Cambridge ; New York, NY, 2019).
- [46] E. M. Rains, *The Electronic Journal of Combinatorics* **5**, R12 (1998).
- [47] K. Schmüdgen, *arXiv preprint arXiv:2008.12698* (2020).
- [48] Z. Li, H. Zheng, Y. Wang, J. Liu, Z.-W. Liu, and L. Jiang, *arXiv e-prints* (2023).
- [49] R. Rasala, *Journal of Algebra* **45**, 132 (1977).
- [50] M. Sellke, *arXiv e-prints*, arXiv:2004.05283 (2020), arXiv:2004.05283 [math.CO].
- [51] R. Zeier and T. Schulte-Herbrüggen, *Journal of Mathematical Physics* **52**, 113510 (2011).
- [52] R. Zeier and Z. Zimborás, *Journal of Mathematical Physics* **56**, 081702 (2015).
- [53] I. Marvian, H. Liu, and A. Hulse, *arXiv e-prints*, arXiv:2202.01963 (2022), arXiv:2202.01963 [quant-ph].
- [54] I. Marvian, *Nature Physics* **18**, 283 (2022).
- [55] I. Pak, F. Petrov, and V. Sokolov, *Math Intelligencer* **42**, 1 (2020).
- [56] S. Knabe, *Journal of Statistical Physics* **52**, 627 (1988).
- [57] B. Nachtergaele, *Communications in Mathematical Physics* **175**, 565 (1996).
- [58] D. Perez-Garcia, F. Verstraete, M. M. Wolf, and J. I. Cirac, *arXiv e-prints*, quant-ph/0608197 (2006), arXiv:quant-ph/0608197 [quant-ph].
- [59] D. Gosset and E. Mozgunov, *Journal of Mathematical Physics* **57**, 091901 (2016).
- [60] P. P. Varjú, *Documenta Mathematica* **18**, 1137 (2013).
